# Supplementary material for: Bidirectional Type Checking for Relational Properties
Source: arXiv:1812.05067 source file (2018-12-12)
Supplement: Supplementary file 2 [file alg-trans.tex]

\begin{lem} [Transitivity of Algorithmic Subtyping for Unary Types] \label{trans-lem-unrel}
    If $\Delta; \psi_a; \Phi_a \jalgasubtype{\grt_1}{\grt_2}{\Phi}$
    and $\Delta; \psi_a; \Phi_a \jalgasubtype{\grt_2}{\grt_3}{\Phi'}$
    and $\Delta; \psi_a; \Phi_a \sat{\cand{\Phi}{\Phi'}} $, then
    $\Delta; \psi_a; \Phi_a \jalgasubtype{\grt_1}{\grt_3}{\Phi''}$ and
    $\Delta; \psi_a; \Phi_a \sat{\Phi''} $.
\end{lem}
\begin{proof}
  Proof is by induction on the two derivations.
\end{proof}

\begin{lem} [Transitivity of Algorithmic Subtyping for Binary Types]
  The following holds:
  \begin{enumerate}
  \item \label{trans-ih-rel}
    If $\Delta; \psi_a; \Phi_a \jalgsubtype{\tau_1}{\tau_2}{\Phi}$
    and $\Delta; \psi_a; \Phi_a \jalgsubtype{\tau_2}{\tau_3}{\Phi'}$
    and $\Delta; \psi_a; \Phi_a \sat{\cand{\Phi}{\Phi'}} $, then
    $\Delta; \psi_a; \Phi_a \jalgsubtype{\tau_1}{\tau_3}{\Phi''}$ and
    $\Delta; \psi_a; \Phi_a \sat{\Phi''} $.

  \item \label{trans-ih-bb}
    If $\Delta; \psi_a; \Phi_a \jalgsubtype{\tbox{\tau_1}}{\tau_2}{\Phi}$
    and $\Delta; \psi_a; \Phi_a \jalgsubtype{\tbox{\tau_2}}{\tau_3}{\Phi'}$
    and $\Delta; \psi_a; \Phi_a \sat{\cand{\Phi}{\Phi'}} $, then
    $\Delta; \psi_a; \Phi_a \jalgsubtype{\tbox{\tau_1}}{\tau_3}{\Phi''}$ and
    $\Delta; \psi_a; \Phi_a \sat{\Phi''} $.
  \item \label{trans-ih-pl} 
    If $\Delta; \psi_a; \Phi_a \jalgsubtype{\tau_1}{\tau_2}{\Phi}$ and $\Delta; \psi_a; \Phi_a \jalgsubtype{\tau_1}{\tlift{\trm{\tau_1}{i}}}{\Phi_i}$
    and $\Delta; \psi_a; \Phi_a \jalgsubtype{\tlift{\trm{\tau_2}{i}}}{\tau_3}{\Phi'}$
    and $\Delta; \psi_a; \Phi_a \sat{\cand{\Phi}{\cand{\Phi'}{\Phi_i}}} $, then
    $\Delta; \psi_a; \Phi_a \jalgsubtype{\tau_1}{\tau_3}{\Phi''}$ and
    $\Delta; \psi_a; \Phi_a \sat{\Phi''} $.

  % \item \label{trans-ih-pl}
  %   If $\Delta; \psi_a; \Phi_a \jalgsubtype{\tbox{\tau_1}}{\tau_2}{\Phi}$
  %   and $\Delta; \psi_a; \Phi_a \jalgsubtype{\tlift{\trm{\tau_2}{i}}}{\tau_3}{\Phi'}$
  %   and $\Delta; \psi_a; \Phi_a \sat{\cand{\Phi}{\Phi'}} $, then
  %   $\Delta; \psi_a; \Phi_a \jalgsubtype{\tbox{\tau_1}}{\tau_3}{\Phi''}$ and
  %   $\Delta; \psi_a; \Phi_a \sat{\Phi''} $.
  % \item \label{trans-ih-p}
  %   If $\Delta; \psi_a; \Phi_a \jalgsubtype{\tau_1}{\tau_2}{\Phi}$
  %   and $\Delta; \psi_a; \Phi_a \jalgsubtype{\tlift{\trm{\tau_2}{i}}}{\tau_3}{\Phi'}$
  %   and $\Delta; \psi_a; \Phi_a \sat{\cand{\Phi}{\Phi'}} $, then
  %   $\Delta; \psi_a; \Phi_a \jalgsubtype{\tbox{\tau_1}}{\tau_3}{\Phi''}$ and
  %   $\Delta; \psi_a; \Phi_a \sat{\Phi''} $.

  \end{enumerate}
\end{lem}

\begin{proof}
  These three statements are proven simultaneously by induction on the
  first two derivations of (1) and (2) and the first and the third derivations of (3).

\end{proof}

\begin{proof}[Proof of statement (1)]
  Proof proceeds by induction on the first derivation.\\
  \begin{mainitem}
    %%%%%%%%%%%%%%%%%%%%%%%%%%%%%%%%%%%%%%%%%%%%%%%%%%%%%%%%%%%%%%%%%%%%%%%
    \caseL{$\stbox$ and $\Delta; \psi_a; \Phi_a \jalgsubtype{\tau_2}{\tau_3}{\Phi'}$ }
    TS: $\Delta; \psi_a; \Phi_a \jalgsubtype{\tbox{\tau_1}}{\tau_3}{\Phi''}$ and $\Delta; \psi_a; \Phi_a \sat{\Phi''} (\star) $.\\
    By IH \ref{trans-ih-rel} on the premise, we get $\Delta; \psi_a; \Phi_a \jalgsubtype{\tau_1}{\tau_3}{\Phi''} ~~~(\diam)$ and $~(\star)$.\\
    By applying \textbf{L-$\square$} to $(\diam)$, we get \\
    $\stbox[\tau_1][\tau_3][]['']$

    %%%%%%%%%%%%%%%%%%%%%%%%%%%%%%%%%%%%%%%%%%%%%%%%%%%%%%%%%%%%%%%%%%%%%%% 
    \caseL{$\stboxBR$ and $\Delta; \psi_a; \Phi_a \jalgsubtype{\tbox{\tau_2}}{\tau_3}{\Phi'}$ }
    TS: $\Delta; \psi_a; \Phi_a \jalgsubtype{\tbox{\tau_1}}{\tau_3}{\Phi''}$ and $\Delta; \psi_a; \Phi_a \sat{\Phi''} (\star) $.\\
    Obtained by IH \ref{trans-ih-bb} on the premise.

    %%%%%%%%%%%%%%%%%%%%%%%%%%%%%%%%%%%%%%%%%%%%%%%%%%%%%%%%%%%%%%%%%%%%%%% 5
    \caseL{$\stboxpushl$ and $\Delta; \psi_a; \Phi_a \jalgsubtype{\tau_2}{\tau_3}{\Phi'}$ }
    TS: $\Delta; \psi_a; \Phi_a \jalgsubtype{\tbox{\tau_1}}{\tau_3}{\Phi''}$ and $\Delta; \psi_a; \Phi_a \sat{\Phi''} (\star) $.\\
    By IH \ref{trans-ih-rel} on the premise, we get $\Delta; \psi_a; \Phi_a \jalgsubtype{\tlift{\trm{\tau_1}{i}}}{\tau_3}{\Phi''} ~~~(\diam)$ and $~(\star)$.\\
    By applying \textbf{$\square$-push-l$_i$} to $(\diam)$, we get \\
    $\stboxpushl[\tau_1][\tau_3][]['']$
    
    %%%%%%%%%%%%%%%%%%%%%%%%%%%%%%%%%%%%%%%%%%%%%%%%%%%%%%%%%%%%%%%%%%%%%%% 
    \caseL{$\stunrel[\tau][\grt_1][\grt_2][(\star)][(\diam)]$ and \\ $\Delta; \psi_a; \Phi_a \jalgsubtype{\tch{\grt_1}{\grt_2}}{\tau_3}{\Phi'} ~~~(\dagg)$ }
    TS: $\Delta; \psi_a; \Phi_a \jalgsubtype{\tau}{\tau_3}{\Phi''}$ and $\Delta; \psi_a; \Phi_a \sat{\Phi''} (\dagg\dagg) $.\\
    By inversion on $(\dagg)$, we know that $\tau_3 = \tch{\grt_1}{\grt_2}$ such that \\
    $\stunrel[\tch{\grt_1}{\grt_2}][\grt_1'][\grt_2'][(\star\star)][(\diam\diam)]$.\\
    By \lemref{trans-lem-unrel} using $(\star)$ and ($\star\star$), we get $\Delta; \psi_a; \Phi_a \jalgasubtype{\trm{\tau}{1}}{\grt_1'}{\Phi_1}$. \\
    By \lemref{trans-lem-unrel} using $(\diam)$ and ($\diam\diam$), we get $\Delta; \psi_a; \Phi_a \jalgasubtype{\trm{\tau}{2}}{\grt_2'}{\Phi_2}$. \\
    Combining these as follows, we get \\
    $\stunrel[\tau][\grt_1'][\grt_2']$.
  \end{mainitem}
\end{proof}

\begin{proof}[Proof of statement (2)] 
  Proof proceeds by induction on the second derivation.\\
  \begin{mainitem}
  \caseL{$\Delta; \psi_a; \Phi_a \jalgsubtype{\tbox{\tau_1}}{\tau_2}{\Phi'} ~~(\star)$ and $\stbox[\tau_2][\tau_3][(\diam)]$ } 
  TS: $\Delta; \psi_a; \Phi_a \jalgsubtype{\tbox{\tau_1}}{\tau_3}{\Phi''}$\\
  Obtained immediately by IH \ref{trans-ih-rel} using $(\star)$ and $(\diam)$.
  
  \caseL{$\Delta; \psi_a; \Phi_a \jalgsubtype{\tbox{\tau_1}}{\tau_2}{\Phi'} ~~(\star)$ and $\stboxBR[\tau_2][\tau_3][(\diam)]$ } 
  TS: $\Delta; \psi_a; \Phi_a \jalgsubtype{\tbox{\tau_1}}{\tbox{\tau_3}}{\Phi''}$\\
  By IH \ref{trans-ih-bb}  using $(\star)$ and $(\diam)$, we get $\Delta; \psi_a; \Phi_a \jalgsubtype{\tbox{\tau_1}}{\tau_3}{\Phi''}$.\\
  By applying \textbf{B-$\square$-R} rule to this, we obtain \\
  $\stboxBR[\tau_1][\tau_3]$
 \caseL{$\Delta; \psi_a; \Phi_a \jalgsubtype{\tbox{\tau_1}}{\tau_2}{\Phi'} ~~(\star)$ and $\stboxpushl[\tau_2][\tau_3][(\diam)]$ } 
 TS: $\Delta; \psi_a; \Phi_a \jalgsubtype{\tbox{\tau_1}}{\tau_3}{\Phi''}$\\
 By \lemref{lem:refl-subtyping} on $\tlift{\trm{\tau_1}{i}}$ (reflexivity) and \textbf{$\square$-push-l$_i$} rule, we obtain : \\ $\stboxpushl[\tau_1][\tlift{\trm{\tau_1}{i}}][][_r]$. \\
 Then, by applying IH \ref{trans-ih-pl} on $(\star)$ and $(\diam)$ and $\Delta; \psi_a; \Phi_a \jalgsubtype{\tbox{\tau_1}}{\tlift{\trm{\tau_1}{i}}}{\Phi_r}$, we get $\Delta; \psi_a; \Phi_a \jalgsubtype{\tbox{\tau_1}}{\tau_3}{\Phi''}$
 \caseL{$\Delta; \psi_a; \Phi_a \jalgsubtype{\tbox{\tau_1}}{\tau_2}{\Phi'} ~~(\star)$ and \\ $\stunrel[\tau_2][\grt_1][\grt_2][(\diam)][(\diam\diam)]$ } 
  TS: $\Delta; \psi_a; \Phi_a \jalgsubtype{\tbox{\tau_1}}{\tch{\grt_1}{\grt_2}}{\Phi''}$\\
  By \lemref{lem:subtyping-proj}, we get
  \begin{enumih}
  \item $\Delta; \psi_a; \Phi_a \jalgasubtype{\trm{\tbox{\tau_1}}{1}}{\trm{\tau_2}{1}}{\Phi_1}$
  \item $\Delta; \psi_a; \Phi_a \sat{\Phi_1}$
  \end{enumih}
  By \lemref{lem:subtyping-proj}, we get
 \begin{enumih} [resume]
 \item $\Delta; \psi_a; \Phi_a \jalgasubtype{\trm{\tbox{\tau_1}}{2}}{\trm{\tau_2}{2}}{\Phi_2}$
 \item$\Delta; \psi_a; \Phi_a \sat{\Phi_2}$
 \end{enumih}
By \lemref{trans-lem-unrel} using (a,b) and $(\diam)$ and similarly using (c,d) and $(\diam\diam)$, we get 
\begin{enumih}[resume]
\item $\Delta; \psi_a; \Phi_a \jalgasubtype{\trm{\tbox{\tau_1}}{1}}{\grt_1}{\Phi_1'}$
\item $\Delta; \psi_a; \Phi_a \sat{\Phi_1'}$
\item $\Delta; \psi_a; \Phi_a \jalgasubtype{\trm{\tbox{\tau_1}}{2}}{\grt_2}{\Phi_1'}$
\item $\Delta; \psi_a; \Phi_a \sat{\Phi_2'}$
\end{enumih}
Combining (e,f) and (g,h), we get \\
$\stunrel[\tbox{\tau_1}][\grt_1][\grt_2][][][']$ 
\end{mainitem}
\end{proof}

\begin{proof}[Proof of statement (3)] 
  Proof proceeds by induction on the first derivation.\\
  \begin{mainitem}
    \caseL{$\stbox[\tau_1][\tau_2][(\star)]$ and $\Delta; \psi_a; \Phi_a \jalgsubtype{\tbox{\tau_1}}{\tlift{\trm{\tau_1}{i}}}{\Phi_i} ~~ (\diam)$  \\ and $\Delta; \psi_a; \Phi_a \jalgsubtype{\tlift{\trm{\tau_2}{i}}}{\tau_3}{\Phi'}~~ (\dagg)$.} 
    TS: $\Delta; \psi_a; \Phi_a \jalgsubtype{\tbox{\tau_1}}{\tau_3}{\Phi''}$.\\
    By inversion on $(\diam)$, we get \\ $\stbox[\tau_1][\tlift{\trm{\tau_1}{i}}][(\diam\diam)][_i]$\\
    By IH \ref{trans-ih-pl} using $(\star)$ and $(\diam\diam)$ and $(\dagg)$, we get 
    $\Delta; \psi_a; \Phi_a \jalgsubtype{\tau_1}{\tau_3}{\Phi''}$. \\
    Finally, we apply \textbf{L-$\square$} to obtain the goal: \\
    $\stbox[\tau_1][\tau_3][]['']$

   \caseL{$\stboxBR$ and $\Delta; \psi_a; \Phi_a \jalgsubtype{\tbox{\tau_1}}{\tlift{\trm{\tau_1}{i}}}{\Phi_i}$ \\ and $\Delta; \psi_a; \Phi_a \jalgsubtype{\tlift{\trm{\tbox{\tau_2}}{i}}}{\tau_3}{\Phi'}$  and  $\Delta; \psi_a; \Phi_a \sat{\Phi''}  $.}
    TS: $\Delta; \psi_a; \Phi_a \jalgsubtype{\tbox{\tau_1}}{\tau_3}{\Phi''}$  \\ 
    Obtained immediately by IH \ref{trans-ih-pl} on the premise. Note that $\tlift{\trm{\tbox{\tau_2}}{i}} = \tlift{\trm{\tau_2}{i}}$
    \caseL{$\stboxpushl[\tau_1][\tau_2][(\star)]$ and $\Delta; \psi_a; \Phi_a \jalgsubtype{\tbox{\tau_1}}{\tlift{\trm{\tau_1}{i}}}{\Phi_i}~~(\diam)$  \\ and  $\Delta; \psi_a; \Phi_a \jalgsubtype{\tlift{\trm{\tau_2}{i}}}{\tau_3}{\Phi'}~(\dagg)$  and $\Delta; \psi_a; \Phi_a \sat{\Phi''}  $ .}
    TS: $\Delta; \psi_a; \Phi_a \jalgsubtype{\tbox{\tau_1}}{\tau_3}{\Phi''}$ .\\
    We know that $\tlift{\trm{\cdot}{i}}$ is idempotent. Therefore ${\tlift{\trm{(\tlift{\trm{\tau_1}{i}})}{i}}} = {\tlift{\trm{\tau_1}{i}}}$.\\
    So by \lemref{lem:refl-subtyping}, we know that $\Delta; \psi_a; \Phi_a \jalgsubtype{\tlift{\trm{\tau_1}{i}}}{\tlift{\trm{(\tlift{\trm{\tau_1}{i}})}{i}}}{\Phi_r}$.\\
    Using this, we can instantiate IH \ref{trans-ih-pl} on $(\star)$ and $(\dagg)$ to get $\Delta; \psi_a; \Phi_a \jalgsubtype{\tlift{\trm{\tau_1}{i}}}{\tau_3}{\Phi''}$.\\
    Next, we apply the \textbf{$\square$-push-l$_i$} to obtain \\
    $\stboxpushl[\tau_1][\tau_3][]['']$
    
   \end{mainitem}

\end{proof}
    
%%% Local Variables:
%%% mode: latex
%%% TeX-master: "main"
%%% End:
