# Supplementary material for: Bidirectional Type Checking for Relational Properties
Source: arXiv:1812.05067 source file (2018-12-12)
Supplement: Supplementary file 3 [file metatheory.tex]

%%% Local Variables:
%%% mode: latex
%%% TeX-master: "main"
%%% End:
