# Supplementary material for: Bidirectional Type Checking for Relational Properties
Source: arXiv:1812.05067 source file (2018-12-12)
Supplement: Supplementary file 4 [file push-box.tex]

\begin{figure}[htp]
\[ \begin{array}{lll} 
     \tboxp{\tau} & \trans & \tau \\
     \tboxp{\tau} & \trans & \tpushd{\tau}
% \tboxp{\tau_1 \tarrd{t} \tau_2} & \trans & \tbox{\tau_1} \tarrd{0} \tbox{\tau_2} \\
% \tboxp{\tch{\grt_1 \uarr{k}{t} \grt_2}{\grt_1' \uarr{k'}{t'} \grt_2'} } & \trans & \tboxp{\tch{\grt_1}{\grt_1'}} \tarrd{0}  \tbox{\tch{\grt_2}{\grt_2'}} \\
% \tboxp{\tch{\grt_1 \ttimes \grt_2}{\grt_1' \ttimes \grt_2'} } &\trans & \tbox{\tch{\grt_1}{\grt_1'}} \ttimes \tbox{\tch{\grt_1'}{\grt_2'}} \\
% \tboxp{\tau_1 \ttimes \tau_2} &\trans & \tbox{\tau_1} \ttimes \tbox{\tau_2} \\
% \tboxp{\tau_1 \tsum \tau_2} &\trans & \tbox{\tau_1} \tsum \tbox{\tau_2} \\
% \tboxp{\tch{\grt_1 \tsum \grt_2}{\grt_1' \tsum \grt_2'} } &\trans & \tbox{\tch{\grt_1}{\grt_1'}} \tsum \tbox{\tch{\grt_1'}{\grt_2'}} \\
% \tboxp{\tlist{n}{\alpha}{\tau}} &\trans & \tlist{n}{0}{\tbox{\tau}} \\
% \tboxp{\tch{\ulist{n}{\grt}}{\ulist{n'}{\grt'}} } &\trans & \tlist{n}{0}{\tbox{\tch{\grt}{\grt'}}}  \\
% \tboxp{\tforalld{i}{t} \tau} &\trans& \tforalld{i}{0} \tbox{\tau} \\
% \tboxp{\tch{\tforall{i}{k}{t} \grt}{\tforall{i}{k'}{t'} \grt'} } &\trans & \tforalld{i}{0} \tbox{\tch{\grt}{\grt'}} \\
% \tboxp{\texists{i} \tau} &\trans& \texists{i} \tbox{\tau} \\
% \tboxp{\tch{\texists{i} \grt}{\texists{i} \grt'} } &\trans & \texists{i} \tbox{\tch{\grt}{\grt'}} \\ 
% \tboxp{\tcimpl{C}{\tau}} &\trans& \tcimpl{C}{\tbox{\tau}} \\
% \tboxp{\tch{\tcimpl{C}{\grt}}{\tcimpl{C}{\grt'}}} &\trans & \tcimpl{C}{\tbox{\tch{\grt}{\grt'}}} \\ 
% \tboxp{\tcprod{C}{\tau}} &\trans& \tcprod{C}{\tbox{\tau}} \\
% \tboxp{\tch{\tcprod{C}{\grt}}{\tcprod{C}{\grt'}}} &\trans & \tcprod{C}{\tbox{\tch{\grt}{\grt'}}} \\ 
% \tau &\trans& \tau
\end{array}\]
\caption{Box elimination}
\end{figure}

%%% Local Variables:
%%% mode: latex
%%% TeX-master: "main"
%%% End:
