# Supplementary material for: Bidirectional Type Checking for Relational Properties
Source: arXiv:1812.05067 source file (2018-12-12)
Supplement: Supplementary file 5 [file reflexibtiy-sub.tex]

\begin{lem}[Reflexivity of Algorithmic Subtyping] \label{lem:refl-subtyping}
  The following hold.
  \begin{enumerate}
  \item $\Delta; \psi_a; \Phi_a \jalgsubtype{\tau}{\tau}{\Phi}$ and $\Delta; \psi_a; \Phi_a \sat{Phi}$.
  \item $\Delta; \psi_a; \Phi_a \jalgasubtype{\grt}{\grt}{\Phi}$ and $\Delta; \psi_a; \Phi_a \sat{Phi}$.
\end{enumerate}
\end{lem}
%%% Local Variables:
%%% mode: latex
%%% TeX-master: "main"
%%% End:
