# Supplementary material for: Bidirectional Type Checking for Relational Properties
Source: arXiv:1812.05067 source file (2018-12-12)
Supplement: Supplementary file 6 [file substitution-lemma.tex]

\begin{lem} [{\tnamemin} Substitution Lemma] \label{lem:subst-lemma}
  If $\ctx \jtypediffM{0}{e_1}{e_1}{\tau_1}$ and If $\Delta;\Phi; x:\tau_1, \Gamma \jtypediffM{t_2}{e_2}{e_2}{\tau_2}$, then $\ctx \jtypediffM{t_2}{e_2[e_1/x]}{e_2[e_1/x]}{\tau_2}$.
  
\end{lem}

\begin{proof}
  By induction on the second derivation.
\end{proof}
%%% Local Variables:
%%% mode: latex
%%% TeX-master: "main"
%%% End:
