# Supplementary material for: Bidirectional Type Checking for Relational Properties
Source: arXiv:1812.05067 source file (2018-12-12)
Supplement: Supplementary file 7 [file subtyping-proj.tex]

\begin{lem} [Algorithmic Subtyping Projection] \label{lem:subtyping-proj}
  If $\Delta; \psi; \Phi_a \jalgeqtype{\tau_1}{\tau_2}{\Phi}$ and $\Delta; \psi; \Phi_a \sat{\Phi}$, then $\exists \Phi_i.$  $\Delta; \psi; \Phi_a \jalgasubtype{\trm{\tau_1}{i}}{\trm{\tau_2}{i}}{\Phi_i}$ and $\Delta; \psi; \Phi_a \sat{\Phi_i}$ for $i \in \{1,2\}$.
  
\end{lem}

%%% Local Variables:
%%% mode: latex
%%% TeX-master: "main"
%%% End:
