# Supplementary material for: Bidirectional Type Checking for Relational Properties
Source: arXiv:1812.05067 source file (2018-12-12)
Supplement: Supplementary file 8 [file subtyping-refl.tex]

\begin{lem} [Reflexivity of Algorithmic Unary Subtyping] \label{lem:refl-subtyping}
   $\Delta; \psi_a; \Phi_a \jalgasubtype{\grt}{\grt}{\Phi}$ and $\Delta; \psi_a; \Phi_a \sat{\Phi}$.
 \end{lem}
 \begin{proof}
   By straightforward induction on the unary type.
 \end{proof}
%%% Local Variables:
%%% mode: latex
%%% TeX-master: "main"
%%% End:
