# Supplementary material for: Bidirectional Type Checking for Relational Properties
Source: arXiv:1812.05067 source file (2018-12-12)
Supplement: Supplementary file 9 [file alg-binary-type-eq-reflexivity.tex]

\begin{lem} [Reflexivity of Algorithmic Binary Type Equivalence] \label{lem:refl-ty-eq}
  $\Delta; \psi_a; \Phi_a \jalgeqtype{\tau}{\tau}{\Phi}$ and $\Delta; \psi_a; \Phi_a \sat{\Phi}$.
 \end{lem}
 \begin{proof}
   By induction on the binary type.
 \end{proof}

%%% Local Variables:
%%% mode: latex
%%% TeX-master: "main"
%%% End:
