# Supplementary material for: Bidirectional Type Checking for Relational Properties
Source: arXiv:1812.05067 source file (2018-12-12)
Supplement: Supplementary file 10 [file alg-completeness.tex]

\begin{thm}[Completeness of the Algorithmic Typechecking]\label{thm:alg-typing-completeness} We have the following.
  \begin{enumerate}
  \item Assume that $\Delta; \Phi_a; \Omega
    \jtypeM{k}{t}{e}{\grt}$.
    Then, $\exists e'$ such that
    \begin{enumerate}
    \item $\Delta; \cdot; \Phi_a; \Omega \chexec{e'}{\grt}{k}{t}{\Phi}$
    \item $\Delta; \Phi_a  \sat \Phi$
    \item $\erty{e'} = e$
    \end{enumerate}

  \item Assume that $\Delta; \Phi_a; \Gamma
    \jtypediffM{t}{e_1}{e_2}{\tau}$.
    Then,  $\exists e_1',e_2'$ such that
    \begin{enumerate}
    \item $\Delta; \cdot; \Phi_a; \Gamma \chdiff{e_1'}{e_2'}{\tau}{t}{\Phi}$
    \item $\Delta; \Phi_a  \sat \Phi$
    \item $\erty{e_1'} = e_1$ and $\erty{e_2'} = e_2$
    \end{enumerate}
 
  \end{enumerate}  
\end{thm}



\begin{proof}
  Proof is by simultaneous induction on the {\tnamemin} typing
  derivations.

\begin{spacing}{1.3}
  \hspace{-1cm} \textbf{Proof of \Cref{thm:alg-typing-completeness}.1:} \\
\begin{mainitem} 
%%%%%%%%%%%%%%%%%%%%%%%%%%%%%%%%%%%%%%%%%%
%%%%%%%%%%%%%%%%%%%%%%%%%%%%%%%%%%%%%%%%%%
%%%%%%%%%%%%%%%%%%%%%%%%%%%%%%%%%%%%%%%%%%
\caseL{\mtyvar}
We can conclude as follows
  \begin{mathpar}
    \inferrule{
      \infvar[\cdot] \\
      \Delta ; \Phi_a \jalgasubtype{\grt}{\grt}{\Phi}~~\text{by~}\cref{lem:alg-unary-subtyping-refl}
    }
    {
      \uctx \chexec{x}{\grt}{0}{0}{\ctrue}
    }~\textbf{alg-r-$\uparrow\downarrow$}
  \end{mathpar}
  
%%%%%%%%%%%%%%%%%%%%%%%%%%%%%%%%%%%%%%%%%%
%%%%%%%%%%%%%%%%%%%%%%%%%%%%%%%%%%%%%%%%%%
%%%%%%%%%%%%%%%%%%%%%%%%%%%%%%%%%%%%%%%%%%
\caseL{\mtycons}
By \Cref{thm:alg-typing-completeness}.2 on the first premise, $\exists e_1'$ such that 
\begin{enumih}
\item $\Delta; \cdot; \Phi_a; \Omega \chexec{e_1'}{\grt}{k_1}{t_1}{\Phi_1}$
\item $\Delta; \Phi_a  \sat \Phi_1$
\item $\erty{e_1'} = e_1$
\end{enumih}
By a), we can show that for $\freshCost{k_1',t_1'}$  where $\Phi_1' = \cand{\Phi_1}{\cand{\ceq{k_1}{k_1'}}{\ceq{t_1}{t_1'}}}$
\begin{equation}
  \label{eq:alg-compl-cons1}
  \Delta; k_1', t_1'; \Phi_a; \Omega \chexec{e_1'}{\grt}{k_1'}{t_1'}{\Phi_1'}
\end{equation}

By \Cref{thm:alg-typing-completeness}.2 on the second premise, $\exists e_2'$ such that 
\begin{enumih}[resume]
\item $\Delta; \cdot; \Phi_a; \Omega \chexec{e_2'}{\ulist{n}{\grt}}{k_2}{t_2}{\Phi_2}$
\item $\Delta; \Phi_a  \sat \Phi_2$
\item $\erty{e_2'} = e_2$
\end{enumih}

By a), we can show that for $\freshCost{i,k_2',t_2'}$  where $\Phi_2' = \cand{\Phi_2}{\cand{\ceq{k_2}{k_2'}}{\cand{\ceq{t_2}{t_2'}}{\ceq{i}{n}}}}$
\begin{equation}
  \label{eq:alg-compl-cons2}
  \Delta; i, k_2', t_2'; \Phi_a; \Omega \chexec{e_2'}{\ulist{i}{\grt}}{k_2'}{t_2'}{\Phi_2'}
\end{equation}
Then, we can conclude as follows 
\begin{enumconc}
\item 
  \begin{mathpar}
     \inferrule
{
\freshCost{k_1',t_1',k_2',t_2'} \\
\freshSize{i} \\
\Delta; {k_1',t_1',\psi_a}; \Phi_a; \Omega  \chexec{e_1'}{\grt}{k_1'}{t_1'}{\Phi_1'}~~\cref{eq:alg-compl-cons1} \\
\Delta; {i,k_2',t_2',\psi_a}; \Phi_a; \Omega
\chexec{e_2'}{\ulist{i}{\grt}}{k_2'}{t_2'}{\Phi_2'}~~\cref{eq:alg-compl-cons2}\\
\Phi_2'' = (\cand{\Phi_2'}{\cand{\ceq{n+1}{(i+1)}}{\cand{\ceq{k_1+k_2}{k_1'+k_2'}}{\ceq{t_1'+t_2'}{t_1+t_2}}}})
}
{
\uctx \chexec{\econsC(e_1',e_2')}{\ulist{n+1}{\grt}}{k_1+k_2}{t_1+t_2}{\cexists{k_1',t_1'}{\scost}{(\cand{\Phi_1'}{\cexists{k_2',t_2'}{\scost}{\cexists{i}{\ssize}{\Phi_2''}}})}}
}~\textbf{alg-u-cons-$\downarrow$}
  \end{mathpar}
\item Using b) and e) for the substitutions $k_i' = k_i$ and $t_i'=t_i$ for the fresh costs and $i=n
$ for the size of the tail.
\item Using c) and f), $\erty{\econsC(e_1',e_2')} = \econsC(e_1,e_2)$
\end{enumconc}
\end{mainitem}
\end{spacing}




\begin{spacing}{1.3}
  \hspace{-1cm} \textbf{Proof of \Cref{thm:alg-typing-completeness}.2:} \\
\begin{mainitem} 
%%%%%%%%%%%%%%%%%%%%%%%%%%%%%%%%%%%%%%%%%%
%%%%%%%%%%%%%%%%%%%%%%%%%%%%%%%%%%%%%%%%%%
%%%%%%%%%%%%%%%%%%%%%%%%%%%%%%%%%%%%%%%%%%
\caseL{\mtyder}

By \Cref{thm:alg-typing-completeness}.2 on the premise, $\exists e_1',e_2'$ such that 
\begin{enumih}
\item $\Delta; \cdot; \Phi_a; \Gamma \chdiff{e_1'}{e_2'}{\tau}{t}{\Phi}$
\item $\Delta; \Phi_a  \sat \Phi$
\item $\erty{e_1'} = e_1$ and $\erty{e_2'} = e_2$
\end{enumih}
Then, we can conclude by using a), b) and c) as follows:\\
 $\chRder[\cdot][']$ and 

 \begin{enumconc}
 \item \begin{mathpar}
     \inferrule { {\inferrule { \chRder[\cdot]['] } {\Delta; \cdot;
           \Phi_a; \Gamma \infdiff{\eannobi{\eder
               e_1'}{\tau}{t}}{\eannobi{\eder
               e_2'}{\tau}{t}}{\tau}{\cdot}{t}{\Phi} }
         ~\textbf{alg-r-anno-$\uparrow$}
       } \\
       \Delta ; \Phi_a \jalgeqtype{\tau}{\tau}{\Phi'}~~\text{by~}\Cref{lem:refl-ty-eq} } { \Delta;
       \cdot; \Phi_a; \Gamma \chdiff{\eannobi{\eder
           e_1'}{\tau}{t}}{\eannobi{\eder
           e_2'}{\tau}{t}}{\tau}{t}{\cand{\Phi}{\cand{\Phi'}{\cleq{t}{t}}}}
     } ~\textbf{alg-r-$\uparrow\downarrow$}
   \end{mathpar}
\item By c), $\erty{\eannobi{\eder
           e_i'}{\tau}{t}} = \eder{\erty{e_i'}}$.
\item By b) and \Cref{lem:refl-ty-eq}.
 \end{enumconc}

%%%%%%%%%%%%%%%%%%%%%%%%%%%%%%%%%%%%%%%%%%
%%%%%%%%%%%%%%%%%%%%%%%%%%%%%%%%%%%%%%%%%%
%%%%%%%%%%%%%%%%%%%%%%%%%%%%%%%%%%%%%%%%%%
\caseL{\mtyswitch}

By \Cref{thm:alg-typing-completeness}.1 on the first premise , $\exists e_1'$ such that 
\begin{enumih}
\item $\Delta; \cdot; \Phi_a; \trm{\Gamma}{1} \chexec{e_1'}{\grt_1}{k_1}{t_1}{\Phi_1}$
\item $\Delta; \Phi_a  \sat \Phi_1$
\item $\erty{e_1'} = e_1$ 
\end{enumih}
By a), we can show that for $\freshCost{k_1',t_1'}$  where $\Phi_1' = \cand{\Phi_1}{\cand{\ceq{k_1}{k_1'}}{\ceq{t_1}{t_1'}}}$
\begin{equation}
  \label{eq:alg-compl-switch1}
  \Delta; k_1', t_1'; \Phi_a; \trm{\Gamma}{1} \chexec{e_1'}{\grt_1}{k_1'}{t_1'}{\Phi_1'}
\end{equation}
By \Cref{thm:alg-typing-completeness}.1 on the second premise , $\exists e_2'$ such that 
\begin{enumih}[resume]
\item $\Delta; \cdot; \Phi_a; \trm{\Gamma}{2} \chexec{e_2'}{\grt_2}{k_2}{t_2}{\Phi_2}$
\item $\Delta; \Phi_a  \sat \Phi_2$
\item $\erty{e_2'} = e_2$ 
\end{enumih}
By d), we can show that for $\freshCost{k_2',t_2'}$ where $\Phi_2' = \cand{\Phi_2}{\cand{\ceq{k_2}{k_2'}}{\ceq{t_2}{t_2'}}}$
\begin{equation}
  \label{eq:alg-compl-switch2}
  \Delta; k_2', t_2'; \Phi_a; \trm{\Gamma}{2} \chexec{e_2'}{\grt_2}{k_2'}{t_2'}{\Phi_2'}
\end{equation}
Then, we can conclude as follows
\begin{enumconc}
\item By using \cref{eq:alg-compl-switch1,eq:alg-compl-switch2}:\\
  $\chRswitch[']$.
\item By using b) and e) and the substitutions $k_i' = k_i$ and $t_i'=t_i$  for the fresh costs where $t= t_1-k_2$.
\item By c) and f), we get $\erty{\eswitch e_i'} = \eswitch{\erty{e_i}}$
\end{enumconc}


%%%%%%%%%%%%%%%%%%%%%%%%%%%%%%%%%%%%%%%%%%
%%%%%%%%%%%%%%%%%%%%%%%%%%%%%%%%%%%%%%%%%%
%%%%%%%%%%%%%%%%%%%%%%%%%%%%%%%%%%%%%%%%%%
\caseL{$\mtyrsubsum$}
By \Cref{thm:alg-typing-completeness}.2 on the first premise, $\exists e_1',e_2'$ such that 
\begin{enumih}
\item $\Delta; \cdot; \Phi_a; \Gamma \chdiff{e_1'}{e_2'}{\tau}{t}{\Phi_1}$
\item $\Delta; \Phi_a  \sat \Phi_1$
\item $\erty{e_1'} = e$ and $\erty{e_2'} = e'$
\end{enumih}
By \Cref{thm:alg-ty-eq-completeness} on the second premise, 
\begin{enumih}[resume]
\item $\Delta ; \Phi_a \jalgeqtype{\tau}{\tau'}{\Phi_2}$ 
\item  $\Delta; \Phi_a \sat \Phi_2$.
\end{enumih}
Then, we can conclude as follows
\begin{enumconc}
\item By using a) and d) 
  \begin{mathpar}
    \inferrule
    {
      {\inferrule
        {
          \Delta; \cdot; \Phi_a; \Gamma \chdiff{e_1'}{e_2'}{\tau}{t}{\Phi_1}
        }
        {\Delta; \cdot; \Phi_a; \Gamma  \infdiff{\eannobi{e_1'}{\tau}{t}}{\eannobi{e_2'}{\tau}{t}}{\tau}{\cdot}{t}{\Phi_1}
        } ~\textbf{alg-r-anno-$\uparrow$} 
      } \\
      \Delta ; \Phi_a \jalgeqtype{\tau}{\tau'}{\Phi_2} 
    }
    { \Delta; \cdot; \Phi_a; \Gamma \chdiff{\eannobi{e_1'}{\tau}{t}}{\eannobi{e_2'}{\tau}{t}}{\tau'}{t'}{\cand{\Phi_1}{\cand{\Phi_2}{\cleq{t}{t'}}}}
       } ~\textbf{alg-r-$\uparrow\downarrow$}
  \end{mathpar}
\item By using b), e) and the third premise, we can show that $\delta; \Phi_a \sat {\cand{\Phi_1}{\cand{\Phi_2}{\cleq{t}{t'}}}}$
\item By c), $\erty{\eannobi{e_1'}{\tau}{t}} = e$ and $\eannobi{e_2'}{\tau}{t} = e'$
\end{enumconc}

%%%%%%%%%%%%%%%%%%%%%%%%%%%%%%%%%%%%%%%%%%
%%%%%%%%%%%%%%%%%%%%%%%%%%%%%%%%%%%%%%%%%%
%%%%%%%%%%%%%%%%%%%%%%%%%%%%%%%%%%%%%%%%%%
\caseL{$\mtyrappD$}
By \Cref{thm:alg-typing-completeness}.2 on the first premise, $\exists \e_1,\e_1'$ such that 
\begin{enumih}
\item $\Delta; \cdot; \Phi_a; \Gamma \chdiff{\e_1}{\e_1'}{\tau_1 \tarrd{t} \tau_2}{t_1}{\Phi_1}$
\item $\Delta; \Phi_a  \sat \Phi_1$
\item $\erty{\e_1} = e_1$ and $\erty{\e_1'} = e_1'$
\end{enumih}

By \Cref{thm:alg-typing-completeness}.2 on the second premise, $\exists \e_2,\e_2'$ such that 
\begin{enumih}[resume]
\item $\Delta; \cdot; \Phi_a; \Gamma \chdiff{\e_2}{\e_2'}{\tau_1}{t_2}{\Phi_2}$
\item $\Delta; \Phi_a  \sat \Phi_2$
\item $\erty{\e_2} = e_2$ and $\erty{\e_2'} = e_2'$
\end{enumih}
By d), we can show that for $\freshCost{t_2'}$ where $\Phi_2' = \cand{\Phi_2}{\ceq{t_2}{t_2'}}$
\begin{equation}
  \label{eq:alg-compl-app1}
  \Delta;  t_2'; \Phi_a; \Gamma \chdiff{\e_2}{\e_2'}{\tau_1}{t_2'}{\Phi_2'}
\end{equation}
Then, we can conclude as follows
\begin{enumconc}
\item 
  \begin{mathpar}
    \inferrule
    {\inferrule
      {
        {\inferrule
          {
            \Delta; \cdot; \Phi_a; \Gamma \chdiff{\e_1}{\e_1'}{\tau_1 \tarrd{t} \tau_2}{t_1}{\Phi_1}
          }
          {\Delta; \cdot; \Phi_a; \Gamma \infdiff{\eannobi{\e_1}{\tau_1 \tarrd{t} \tau_2}{t_1}}{\eannobi{\e_1'}{\tau_1 \tarrd{t} \tau_2}{t_1}}{\tau_1 \tarrd{t} \tau_2}{\cdot}{t_1}{\Phi_1} }~\textbf{alg-r-anno-$\uparrow$} 
        } \\
        \freshCost{t_2'}\\
        \Delta;  t_2'; \Phi_a; \Gamma \chdiff{\e_2}{\e_2'}{\tau_1}{t_2'}{\Phi_2'}
      }
      {
        \Delta; \cdot; \Phi_a; \Gamma \infdiff{E_1}{E_2}{\tau_2}{t_2'}{t_1+t+t_2'}{\cand{\Phi_1}{\Phi_2'}}
    }~\textbf{c-r-app}}
  {
    \Delta; \cdot; \Phi_a; \Gamma \chdiff{E_1}{E_2}{\tau_2}{t_1+t+t_2}{\cexists{t_2'}{\scost}{\cand{\Phi_1}{\cand{\Phi_2'}{\cleq{t_1+t+t_2'}{t_1+t+t_2}}}}}
  }~\textbf{alg-r-$\uparrow\downarrow$} 
\end{mathpar} \\
where $E_1= \eannobi{\e_1}{\tau_1 \tarrd{t} \tau_2}{t_1} \eapp \e_2$ and $E_2= \eannobi{\e_1'}{\tau_1 \tarrd{t} \tau_2}{t_1} \eapp \e_2'$.
\item By using b) and e) and the substitution $t_2'=t_2$  for the fresh cost.
\item Using c) and f),  $\erty{\eannobi{\e_1}{\tau_1 \tarrd{t} \tau_2}{t_1} \eapp \e_2} = e_1 \eapp e_2$ and $\erty{\eannobi{\e_1'}{\tau_1 \tarrd{t} \tau_2}{t_1} \eapp \e_2'} = e_1' \eapp e_2'$.
\end{enumconc}


%%%%%%%%%%%%%%%%%%%%%%%%%%%%%%%%%%%%%%%%%%
%%%%%%%%%%%%%%%%%%%%%%%%%%%%%%%%%%%%%%%%%%
%%%%%%%%%%%%%%%%%%%%%%%%%%%%%%%%%%%%%%%%%%
\caseL{$\mtyrunpackD$}
By \Cref{thm:alg-typing-completeness}.2 on the first premise, $\exists \e_1,\e_1'$ such that 
\begin{enumih}
\item $\Delta; \cdot; \Phi_a; \Gamma \chdiff{\e_1}{\e_1'}{\texists{i}\tau_1}{t_1}{\Phi_1}$
\item $\Delta; \Phi_a  \sat \Phi_1$
\item $\erty{\e_1} = e_1$ and $\erty{\e_1'} = e_1'$
\end{enumih}

By \Cref{thm:alg-typing-completeness}.2 on the second premise, $\exists \e_2,\e_2'$ such that 
\begin{enumih}[resume]
\item $\sorted{i}, \Delta; \cdot; \Phi_a; x: \tau_1, \Gamma \chdiff{\e_2}{\e_2'}{\tau_2}{t_2}{\Phi_2}$
\item $\sorted{i}, \Delta; \Phi_a  \sat \Phi_2$
\item $\erty{\e_2} = e_2$ and $\erty{\e_2'} = e_2'$
\end{enumih}
By d), we can show that for $\freshCost{t_2'}$ where $\Phi_2' = \cand{\Phi_2}{\ceq{t_2}{t_2'}}$
\begin{equation}
  \label{eq:alg-compl-unpack1}
  \sorted{i}, \Delta;  t_2'; \Phi_a; x: \tau_1, \Gamma \chdiff{\e_2}{\e_2'}{\tau_2}{t_2'}{\Phi_2'}
\end{equation}
Then, we can conclude as follows
\begin{enumconc}
\item \begin{mathpar}
    \inferrule { {\inferrule{ \Delta; \cdot; \Phi_a; \Gamma
          \chdiff{\e_1}{\e_1'}{\texists{i}\tau_1}{t_1}{\Phi_1}~~(a) }
        { \Delta; \cdot; \Phi_a; \Gamma
          \infdiff{E_1}{E_1'}{\texists{i}\tau_1}{\cdot}{t_1}{\Phi_1}
        }~\textbf{alg-r-anno-$\uparrow$} } \\
      \sorted{i}, \Delta;  t_2'; \Phi_a; x: \tau_1, \Gamma \chdiff{\e_2}{\e_2'}{\tau_2}{t_2'}{\Phi_2'}~~(\cref{eq:alg-compl-unpack1}) \\
      \Phi'=
      \cexists{t_2'}{\scost}{\cand{\Phi_1}{\cand{\Phi_2'}{\ceq{t_1+t_2'}{t_1+t_2}}}}
    } {\Delta; \cdot; \Phi_a; \Gamma \chdiff{\eunpack E_1 \eas (x, i)
        \ein \e_2}{\eunpack E_1' \eas (x, i) \ein
        \e_2'}{\tau_2}{t_1+t_2}{\Phi'}
    }~\textbf{alg-r-unpack-$\downarrow$}
  \end{mathpar}
  where $E_1= \eanno{\e_1}{\texists{i}\tau_1}{t_1}$ and
  $E_2= \eanno{\e_1'}{\texists{i}\tau_1}{t_1}$
\item By using b) and e) and the substitution $t_2'=t_2$  for the fresh cost.
\item Using c) and f),  $\erty{\eunpack \eannobi{\e_1}{\texists{i} \tau_1}{t_1} \eas (x,i) \ein \e_2} = \eunpack e_1 \eas (x,i) \ein e_2$ and  $\erty{\eunpack \eannobi{\e_1'}{\texists{i} \tau_1}{t_1} \eas (x,i) \ein \e_2'} = \eunpack e_1' \eas (x,i) \ein e_2'$.
\end{enumconc}
\end{mainitem}
\end{spacing}

\end{proof}
%%% Local Variables:
%%% mode: latex
%%% TeX-master: "main"
%%% End:
