# Supplementary material for: Bidirectional Type Checking for Relational Properties
Source: arXiv:1812.05067 source file (2018-12-12)
Supplement: Supplementary file 11 [file alg-soundness.tex]

\begin{thm}[Soundness of the Algorithmic Typechecking]\label{thm:alg-typing-soundness} We have the following.
  \begin{enumerate}
  \item Assume that $\uctx \chexec{e}{\grt}{k}{t}{\Phi}$ and
    \begin{enumerate}
    \item $\fivars{\Phi_a,\Omega,\grt,k, t} \subseteq dom(\Delta, \psi_a) $
    % \item $\Delta; \psi_a; \Phi_a \awfctx{\Omega}$
    % \item $\Delta;\psi_a; \Phi_a \awfty{\grt}$
    \item  $\Delta; \suba{\Phi_a} \sat \suba{\Phi}$ is provable for some $\theta_a$ such that  $\subsat{\Delta}{\theta_a}{\psi_a}$ is  derivable
    \end{enumerate}
    Then $\Delta; \suba{\Phi_a}; \suba{\Omega}
    \jtypeM{\suba{k}}{\suba{t}}{\erty{e}}{\suba{\grt}}$.

\item Assume that $\uctx \infexec{e}{\grt}{\psi}{k}{t}{\Phi}$ and 
  \begin{enumerate}
  \item $\fivars{\Phi_a,\Omega} \subseteq dom(\Delta, \psi_a)$
  % \item $\Delta; \psi_a; \Phi_a \awfctx{\Omega}$
  \item $\forall \theta~\forall \theta_a$. $\Delta; \suba{\Phi_a} \sat
    \subta{\Phi}$ is provable s.t
$\subsat{\Delta}{\theta}{\psi}$ and $\subsat{\Delta}{\theta_a}{\psi_a}$ are derivable
  \end{enumerate}
   Then $\Delta; \suba{\Phi_a};
\suba{\Omega} \jtypeM{\subta{k}}{\subta{t}}{\erty{e}}{\subta{\grt}}$ % and $\Delta; \psi_a; \Phi_a \awfty{\grt} $
.

  \item Assume that $\bctx \chdiff{e}{e'}{\tau}{t}{\Phi}$ and
    \begin{enumerate}
    \item $\fivars{\Phi_a,\Gamma,\tau,t} \subseteq dom(\Delta, \psi_a)$
    % \item $\Delta; \psi_a; \Phi_a \wfctx{\Gamma}$
    % \item $\Delta;\psi_a; \Phi_a \wfty{\tau}$
    \item  $\Delta; \suba{\Phi_a} \sat \suba{\Phi}$ is provable for some $\theta_a$ such that  $\subsat{\Delta}{\theta_a}{\psi_a}$ is derivable
    \end{enumerate}
    Then $\Delta; \suba{\Phi_a}; \suba{\Gamma} 
    \jtypediffM{\suba{t}}{\erty{e}}{\erty{e'}}{\suba{\tau}}$.

\item  Assume that $\bctx \infdiff{e}{e'}{\tau}{\psi}{t}{\Phi}$ and
  \begin{enumerate}
  \item $\fivars{\Phi_a,\Gamma} \subseteq dom(\Delta, \psi_a) $
  % \item $\Delta; \psi_a; \Phi_a \wfctx{\Gamma}$
  \item $\forall \theta~\forall \theta_a$. $\Delta; \suba{\Phi_a} \sat
    \subta{\Phi}$ is provable s.t
$\subsat{\Delta}{\theta}{\psi}$ and $\subsat{\Delta}{\theta_a}{\psi_a}$ are derivable
  \end{enumerate}
   Then $\Delta; \suba{\Phi_a};
\suba{\Gamma} \jtypediffM{\subta{t}}{\erty{e}}{\erty{e'}}{\subta{\tau}}$ % and $\Delta; \psi_a; \Phi_a \wfty{\tau}$
.

 
  \end{enumerate}  
\end{thm}

 


\begin{proof}
  Statements (1---4) follow from simultaneous structural induction on the algorithmic typing derivations. We present several cases below.

\begin{spacing}{1.3}
  \hspace{-1cm} \textbf{Proof of \Cref{thm:alg-typing-soundness}.1:} \\
  
  % Unless otherwise stated, assume that we can partition $\Delta$ as
  % $\Delta = \Delta_e, \Delta_u$ and $\forall \theta~\forall\theta_e.$
  % $\Delta_u \sat \sub{\Phi}{\theta~\theta_e}$ is provable where
  % $\subsat{\Delta_u}{\theta}{\psi}$ and
  % $\subsat{\cdot}{\theta_e}{\Delta_e}$ are derivable.
\begin{mainitem}
  \setlength{\itemsep}{10pt}

%%%%%%%%%%%%%%%%%%%%%%%%%%%%%%%%%%%%%%%%%%
%%%%%%%%%%%%%%%%%%%%%%%%%%%%%%%%%%%%%%%%%%
%%%%%%%%%%%%%%%%%%%%%%%%%%%%%%%%%%%%%%%%%%
  \caseL{\chpair}
  TS: $\Delta; \suba{\Phi_a}; \suba{\Omega}  \jtypeM{\suba{k}}{\suba{t}}{\la \erty{e_1}, \erty{e_2} \ra}{\suba{\grt_1} \ttimes \suba{\grt_2}}$. \\
By the main assumptions, we have
$\fivars{\Phi_a,\Omega,\grt,k, t} \subseteq dom(\Delta, \psi_a)~~(\star)$ \\
$\Delta; \suba{\Phi_a} \sat \suba{(\cexists{k_1,t_1}{\scost}{\cand{\Phi_1}{\cexists{k_2,t_2}{\scost}{\cand{\Phi_2}{\cand{\ceq{(t_1+t_2)}{t}}{\ceq{(k_1+k_2)}{k}}}}}})}~~(\star\star)$ \\
Using $(\star)$,  $(\star\star)$'s derivation must be in a form such that we have
\begin{enumih}
\item $\Delta \sty{K_1}{\scost}$ and  $\Delta \sty{T_1}{\scost}$ 
\item $\Delta \sty{K_2}{\scost}$ and  $\Delta \sty{T_2}{\scost}$ 
\item $\Delta; \suba{\Phi_a} \sat \subaex{\Phi_1}{k_1\mapsto K_1, t_1 \mapsto T_1}$
\item $\Delta; \suba{\Phi_a} \sat \subaex{\Phi_2}{k_2 \mapsto K_2, t_2 \mapsto T_2}$
\item $\Delta; \suba{\Phi_a} \sat {\cand{\ceq{(T_1+T_2)}{\suba{t}}}{\ceq{(K_1+K_2)}{\suba{k}}}}$
\end{enumih}

By \Cref{thm:alg-typing-soundness}.1 on the first premise using $(\star)$ and c), we can show that
\begin{equation}
  \label{eq:alg-usound-pair1}
      \Delta; \suba{\Phi_a}; \suba{\Omega}  \jtypeM{K_1}{T_1}{\erty{e_1}}{\suba{\grt_1}}
\end{equation}
By \Cref{thm:alg-typing-soundness}.1 on the second premise using $(\star)$ and d), we can show that
\begin{equation}
  \label{eq:alg-usound-pair2}
      \Delta; \suba{\Phi_a}; \suba{\Omega}  \jtypeM{K_2}{T_2}{\erty{e_2}}{\suba{\grt_2}}
\end{equation}
Combining \cref{eq:alg-usound-pair1,eq:alg-usound-pair2} with \textbf{c-prod} rule, we get \\
$      \Delta; \suba{\Phi_a}; \suba{\Omega}  \jtypeM{K_1+ K_2}{T_1+T_2}{\la \erty{e_1}, \erty{e_2} \ra}{\suba{\grt_1} \ttimes \suba{\grt_2}}$. \\
Then, by using e) with the  \textbf{c-}$\pmb{\sqsubseteq}\wexec$ rule
, we can conclude that $\Delta; \suba{\Phi_a}; \suba{\Omega}  \jtypeM{\suba{k}}{\suba{t}}{\la \erty{e_1}, \erty{e_2} \ra}{\suba{\grt_1} \ttimes \suba{\grt_2}}$. \\

%%%%%%%%%%%%%%%%%%%%%%%%%%%%%%%%%%%%%%%%%%
%%%%%%%%%%%%%%%%%%%%%%%%%%%%%%%%%%%%%%%%%%
%%%%%%%%%%%%%%%%%%%%%%%%%%%%%%%%%%%%%%%%%%
  \caseL{\chupdown}
  TS: $\Delta; \suba{\Phi_a}; \suba{\Omega}  \jtypeM{\suba{k}}{\suba{t}}{\erty{e}}{\suba{\grt}}$. \\
By the main assumptions, we have
$\fivars{\Phi_a,\Omega,\grt,k, t} \subseteq dom(\Delta, \psi_a)~~(\star)$ and \\
$\Delta; \suba{\Phi_a} \sat \suba{(\cexistsS{(\psi)}{\cand{\Phi_1}{\cand{\Phi_2}{\cand{\cleq{t'}{t}}{\cleq{k}{k'}}}}})}~~(\star\star)$ \\
By \Cref{invariant:alg-typechecking} using $(\star)$ and the first premise, we get $ \fivars{\grt',k', t',\Phi_1} \subseteq
dom(\Delta, \psi; \psi_a)~(\diam)$.\\
Using $(\star)$ and $ (\diam)$,  $(\star\star)$'s derivation must be in a form such that we have
\begin{enumih}
\item $\subsat{\Delta}{\theta_a}{\psi_a}$
\item $\Delta; \suba{\Phi_a} \sat \subaex{\Phi_1}{\theta_a}$
\item $\Delta; \suba{\Phi_a} \sat \subaex{\Phi_2}{\theta_a}$
\item $\Delta; \suba{\Phi_a} \sat {\cand{\cleq{\subta{t'}}{\suba{t}}}{\cleq{\suba{k}}{\subta{k'}}}}$
\end{enumih}
By \Cref{thm:alg-typing-soundness}.2 on the first premise using $(\star)$, a) and b), we can show that
\begin{equation}
  \label{eq:alg-usound-updown1}
      \Delta; \suba{\Phi_a}; \suba{\Omega}  \jtypeM{\subta{k'}}{\subta{t'}}{\erty{e}}{\subta{\grt'}}
\end{equation}
By \Cref{thm:alg-unary-subtyping-soundness} using the second premise and c), we obtain
\begin{equation}
  \label{eq:alg-usound-updown2}
      \Delta; \suba{\Phi_a} \jasubtype{\subta{\grt'}}{{\subta{\grt}}}
\end{equation}
Note that due to $(\star)$, we have ${\subta{\grt}}= {\suba{\grt}}$. Then we can conclude by the  \textbf{c-}${\pmb{\sqsubseteq}\wexec}$ rule using \cref{eq:alg-usound-updown1,eq:alg-usound-updown2} and (d) that  $\Delta; \suba{\Phi_a}; \suba{\Omega}  \jtypeM{\suba{k}}{\suba{t}}{\erty{e}}{\suba{\grt}}$.


%%%%%%%%%%%%%%%%%%%%%%%%%%%%%%%%%%%%%%%%%%
%%%%%%%%%%%%%%%%%%%%%%%%%%%%%%%%%%%%%%%%%%
%%%%%%%%%%%%%%%%%%%%%%%%%%%%%%%%%%%%%%%%%%
  \caseL{\chfix}
  TS: $\Delta; \suba{\Phi_a}; \suba{\Omega}  \jtypeM{\suba{k}}{\suba{t}}{\efix f(x). \erty{e}}{\suba{\grt_1} \uarr{\suba{k'}}{\suba{t'}} \suba{\grt_2}}$. \\
By the main assumptions, we have
$\fivars{\Phi_a,\Omega,\grt_1 \uarr{k'}{t'},k, t} \subseteq dom(\Delta, \psi_a)~~(\star)$ and \\
$\Delta; \suba{\Phi_a} \sat \suba{\cand{\Phi}{\cand{\ceq{0}{k}}{\ceq{0}{t'}}}}~~(\star\star)$ \\
Using $(\star)$, we can show that
\begin{enumih}
\item $\fivars{\Phi_a,\Omega,\grt_1, \grt_1 \uarr{k'}{t'}, \grt_2, k', t'} \subseteq dom(\Delta, \psi_a).$\\
\end{enumih}
We also can show that $(\star\star)$'s derivation must be in a form such that we have
\begin{enumih}[resume]
\item $\Delta; \suba{\Phi_a} \sat \suba{\Phi}$
\item $\Delta; \suba{\Phi_a} \sat \ceq{0}{\suba{k}}$
\item $\Delta; \suba{\Phi_a} \sat \ceq{0}{\suba{t}}$
\end{enumih}
By \Cref{thm:alg-typing-soundness}.1 on the first premise using a) and b), we can show that
\begin{equation}
  \label{eq:alg-usound-fix}
      \Delta; \suba{\Phi_a}; x:\suba{\grt_1},f: {\suba{\grt_1} \uarr{\suba{k'}}{\suba{t'}} \suba{\grt_2}}, \suba{\Omega}  \jtypeM{\suba{k'}}{\suba{t'}}{\erty{e}}{\suba{\grt_2}}
    \end{equation}
    By the \textbf{c-fix} rule using \cref{eq:alg-usound-fix}, we obtain \\
    $\Delta; \suba{\Phi_a}; \suba{\Omega}  \jtypeM{0}{0}{\efix f(x). \erty{e}}{\suba{\grt_1} \uarr{\suba{k'}}{\suba{t'}} \suba{\grt_2}}$. \\
    By  \textbf{c-}${\pmb{\sqsubseteq}\wexec}$ rule using (c) and (d), we obtain
    $\Delta; \suba{\Phi_a}; \suba{\Omega}
    \jtypeM{\suba{k}}{\suba{t}}{\efix f(x). \erty{e}}{\suba{\grt_1}
      \uarr{\suba{k'}}{\suba{t'}} \suba{\grt_2}}$.


%%%%%%%%%%%%%%%%%%%%%%%%%%%%%%%%%%%%%%%%%%
%%%%%%%%%%%%%%%%%%%%%%%%%%%%%%%%%%%%%%%%%%
%%%%%%%%%%%%%%%%%%%%%%%%%%%%%%%%%%%%%%%%%%
  \caseL{\chiLam}
  TS: $\Delta; \suba{\Phi_a}; \suba{\Omega}  \jtypeM{\suba{k}}{\suba{t}}{\eLam i. \erty{e}}{\tforall{i}{\suba{k_e}}{\suba{t_e}} \suba{\grt}}$. \\
By the main assumptions, we have
$\fivars{\Phi_a,\Omega, \tforall{i}{k_e}{t_e} \grt, k, t} \subseteq dom(\Delta, \psi_a)~~(\star)$ and \\
$\Delta; \suba{\Phi_a} \sat \suba{(\cand{(\cforall{i}{S}{\Phi})}{\cand{\ceq{0}{k}}{\ceq{0}{t}}})}~~(\star\star)$ \\
Using $(\star)$, we can show that
\begin{enumih}
\item $\fivars{\Phi_a,\Omega, \grt, k_e, t_e} \subseteq i, dom( \Delta, \psi_a).$
\end{enumih}
We can also show that $(\star\star)$'s derivation must be in a form such that we have
\begin{enumih}[resume]
\item $\sorted{i}, \Delta; \suba{\Phi_a} \sat \suba{\Phi}$
\item $\Delta; \suba{\Phi_a} \sat \ceq{0}{\suba{k}}$
\item $\Delta; \suba{\Phi_a} \sat {\ceq{0}{\suba{t}}}$
\end{enumih}
By \Cref{thm:alg-typing-soundness}.1 on the premise using a) and b), we can show that
\begin{equation}
  \label{eq:alg-usound-iLam}
      \sorted{i}, \Delta; \suba{\Phi_a}; \suba{\Omega}  \jtypeM{\suba{k_e}}{\suba{t_e}}{\erty{e}}{\suba{\grt}}
    \end{equation}
    By the \textbf{c-iLam} rule using \cref{eq:alg-usound-iLam}, we obtain 
    $\Delta; \suba{\Phi_a}; \suba{\Omega}  \jtypeM{0}{0}{\eLam i. \erty{e}}{\tforall{i}{\suba{k_e}}{\suba{t_e}} \suba{\grt}}$. \\
    By  \textbf{c-}${\pmb{\sqsubseteq}\wexec}$ rule using (c) and (d), we obtain
 $\Delta; \suba{\Phi_a}; \suba{\Omega}  \jtypeM{\suba{k}}{\suba{t}}{\eLam i. \erty{e}}{\tforall{i}{\suba{k_e}}{\suba{t_e}} \suba{\grt}}$.


%%%%%%%%%%%%%%%%%%%%%%%%%%%%%%%%%%%%%%%%%%
%%%%%%%%%%%%%%%%%%%%%%%%%%%%%%%%%%%%%%%%%%
%%%%%%%%%%%%%%%%%%%%%%%%%%%%%%%%%%%%%%%%%%
  \caseL{\chpack}
  TS: $\Delta; \suba{\Phi_a}; \suba{\Omega}  \jtypeM{\suba{k}}{\suba{t}}{\epack \erty{e} \ewith I }{\texists{i} \suba{\grt}}$. \\ 
By the main assumptions, we have
$\fivars{\Phi_a,\Omega, \texists{i} \grt, k, t} \subseteq dom(\Delta, \psi_a)~~(\star)$ and \\
$\Delta; \suba{\Phi_a} \sat \suba{\Phi}~~(\star\star)$ \\
Using $(\star)$ and the second premise, we can show that
\begin{enumih}
\item $\fivars{\Phi_a,\Omega, \grt\{I/i\}, k, t} \subseteq dom(\Delta, \psi_a).$
\end{enumih}
By \Cref{thm:alg-typing-soundness}.1 on the premise using a) and $(\star\star)$, we can show that
\begin{equation}
  \label{eq:alg-usound-pack}
       \Delta; \suba{\Phi_a}; \suba{\Omega}  \jtypeM{\suba{k}}{\suba{t}}{\erty{e}}{\suba{\grt}\{I/i\}}
    \end{equation}
    By the \textbf{c-pack} rule using \cref{eq:alg-usound-pack} and the second premise, we obtain \\
    $\Delta; \suba{\Phi_a}; \suba{\Omega}  \jtypeM{\suba{k}}{\suba{t}}{\epack \erty{e} \ewith I}{\texists{i} \suba{\grt}}$. 



%%%%%%%%%%%%%%%%%%%%%%%%%%%%%%%%%%%%%%%%%%
%%%%%%%%%%%%%%%%%%%%%%%%%%%%%%%%%%%%%%%%%%
%%%%%%%%%%%%%%%%%%%%%%%%%%%%%%%%%%%%%%%%%%
  \caseL{\chunpack}
  TS: $\Delta; \suba{\Phi_a}; \suba{\Omega}  \jtypeM{\suba{k}}{\suba{t}}{\eunpack \erty{e_1} \ewith (x,i) \ein \erty{e_2}}{\suba{\grt_2}}$. \\ 
By the main assumptions, we have
$\fivars{\Phi_a,\Omega, \grt_2, k, t} \subseteq dom(\Delta, \psi_a)~~(\star)$ and \\
$\Delta; \suba{\Phi_a} \sat \suba{(\cexistsS{(\psi)}{(\cand{\Phi_1}{\cexists{k_2,t_2}{\scost}{\cforall{i}{\sort}{\cand{\Phi_2}{\cand{\ceq{(t_1+t_2+\kunpack)}{t}}{\ceq{(k_1+k_2+\kunpack)}{k}}}}}})})}~~(\star\star)$ \\
By \Cref{invariant:alg-typechecking} using the first premise and $(\star)$, we get $ \fivars{\grt_1,k_1, t_1,\Phi_1} \subseteq dom(\Delta, \psi; \psi_a)~(\diam)$.\\
Using $(\star)$, $ (\diam)$ and the 4th premise,  $(\star\star)$'s derivation must be in a form such that we have
\begin{enumih}
\item $\subsat{\Delta}{\theta}{\psi}$
\item $\Delta; \suba{\Phi_a} \sat \subta{\Phi_1}$
\item $\sorted{i}, \Delta; \suba{\Phi_a} \sat \subaex{\Phi_2}{\theta, k_2 \mapsto K_2, t_2 \mapsto T_2}$
\item $\Delta; \suba{\Phi_a} \sat \ceq{\subta{t_1}+T_2+\kunpack}{\suba{t}}$
\item $\Delta ; \suba{\Phi_a} \sat \ceq{\suba{k}}{\subta{k_1}+K_2+\kunpack}$
\end{enumih}
By \Cref{thm:alg-typing-soundness}.2 on the first premise using $(\star)$, a) and b), we can show that
\begin{equation}
  \label{eq:alg-usound-unpack1}
      \Delta; \suba{\Phi_a}; \suba{\Omega}  \jtypeM{\subta{k_1}}{\subta{t_1}}{\erty{e_1}}{\texists{i} \subta{\grt_1}}
\end{equation}
From $(\star)$ and $(\diam)$, we can show that
\begin{enumih}[resume]
 \item $\fivars{\Phi_a, \grt_1, \Omega, \grt_2, k_2, t_2} \subseteq i, k_2, t_2, dom(\Delta, \psi, \psi_a)$
\end{enumih}
By \Cref{thm:alg-typing-soundness}.1 on the second premise using c), f), $(\star)$ and $(\diam)$, we obtain
\begin{equation}
  \label{eq:alg-usound-unpack2}
     \sorted{i}, \Delta; \suba{\Phi_a}; x: \subta{\grt_1}, \suba{\Omega} \jtypeM{K_2}{T_2}{\erty{e_2}}{\subta{\grt_2}}
\end{equation}
Note that due to $(\star)$, we have ${\subta{\grt_2}}= {\suba{\grt_2}}$. Then by the \textbf{c-unpack} rule using \cref{eq:alg-usound-unpack1,eq:alg-usound-unpack2}, we can show that $\Delta; \suba{\Phi_a}; \suba{\Omega}  \jtypeM{\subta{k_1} + K_1 +\kunpack}{\subta{t_1}+T_2+\kunpack}{\eunpack \erty{e_1} \ewith (x,i) \ein \erty{e_2}}{\suba{\grt_2}}$. \\
By ${\pmb{\sqsubseteq}\wexec}$ rule using (d) and (e),
we obtain
$\Delta; \suba{\Phi_a}; \suba{\Omega}
\jtypeM{\suba{k}}{\suba{t}}{\eunpack \erty{e_1} \ewith (x,i) \ein
  \erty{e_2}}{\suba{\grt_2}}$.

%%%%%%%%%%%%%%%%%%%%%%%%%%%%%%%%%%%%%%%%%%
%%%%%%%%%%%%%%%%%%%%%%%%%%%%%%%%%%%%%%%%%%
%%%%%%%%%%%%%%%%%%%%%%%%%%%%%%%%%%%%%%%%%%
  \caseL{\chsplit}
  TS: $\Delta; \suba{\Phi_a}; \suba{\Omega}  \jtypeM{\suba{k}}{\suba{t}}{\esplit (\erty{e_1}, \erty{e_2}) \ewith C}{\suba{\grt}}$. \\ 
By the main assumptions, we have
$\fivars{\Phi_a,\Omega, \grt, k, t} \subseteq dom(\Delta, \psi_a)~~(\star)$ and \\
$\Delta; \suba{\Phi_a} \sat \suba{(\cand{\cimpl{C}{\Phi_1}}{\cimpl{\neg C}{\Phi_2}})}~~(\star\star)$ \\
Using $(\star)$ and the third premise, we can show that
\begin{enumih}
\item $\fivars{C\wedge \Phi_a,\Omega, \grt, k, t} \subseteq dom(\Delta, \psi_a).$
\item $\fivars{\neg C\wedge \Phi_a,\Omega, \grt, k, t} \subseteq dom(\Delta, \psi_a).$
\end{enumih}


Using $(\star\star)$ and the third premise, we can show that
\begin{enumih}[resume]
\item $\Delta; C \wedge \suba{\Phi_a} \sat \suba{\Phi_1}$
\item $\Delta; \neg C \wedge \suba{\Phi_a} \sat \suba{\Phi_2}$
\end{enumih}
By \Cref{thm:alg-typing-soundness}.1 on the first premise using $(\star)$ and c), we can show that
\begin{equation}
  \label{eq:alg-usound-split1}
       \Delta; C \wedge \suba{\Phi_a}; \suba{\Omega}  \jtypeM{\suba{k}}{\suba{t}}{\erty{e_1}}{\suba{\grt}\{\suba{I}/i\}}
    \end{equation}
By \Cref{thm:alg-typing-soundness}.1 on the second premise using $(\star)$ and d), we can show that
\begin{equation}
  \label{eq:alg-usound-split2}
       \Delta; \neg C \wedge \suba{\Phi_a}; \suba{\Omega}  \jtypeM{\suba{k}}{\suba{t}}{\erty{e_2}}{\suba{\grt}\{\suba{I}/i\}}
    \end{equation}
    By the \textbf{c-split} rule using \cref{eq:alg-usound-split1,eq:alg-usound-split2} and the third premise, we obtain \\ $\Delta; \suba{\Phi_a}; \suba{\Omega}  \jtypeM{\suba{k}}{\suba{t}}{\esplit (\erty{e_1}, \erty{e_2}) \ewith C}{\suba{\grt}}$.



%%%%%%%%%%%%%%%%%%%%%%%%%%%%%%%%%%%%%%%%%%
%%%%%%%%%%%%%%%%%%%%%%%%%%%%%%%%%%%%%%%%%%
%%%%%%%%%%%%%%%%%%%%%%%%%%%%%%%%%%%%%%%%%%
  \caseL{\chcimplIntro}
  TS: $\Delta; \suba{\Phi_a}; \suba{\Omega}  \jtypeM{\suba{k}}{\suba{t}}{ \erty{e} }{\tcimpl{\suba{C}}{\suba{\grt}}}$. \\ 
By the main assumptions, we have
$\fivars{\Phi_a,\Omega, \tcimpl{C}{\grt}, k, t} \subseteq dom(\Delta, \psi_a)~~(\star)$ and \\
$\Delta; \suba{\Phi_a} \sat \suba{(\cimpl{C}{\Phi})}~~(\star\star)$ \\
Using $(\star)$, we can show that
\begin{enumih}
\item $\fivars{C \wedge \Phi_a,\Omega, \grt, k, t} \subseteq dom(\Delta, \psi_a).$
\end{enumih}
By \Cref{thm:alg-typing-soundness}.1 on the premise using $(\star)$ and a), we can show that
\begin{equation}
  \label{eq:alg-usound-cimpl}
       \Delta; \suba{C} \wedge \suba{\Phi_a}; \suba{\Omega}  \jtypeM{\suba{k}}{\suba{t}}{\erty{e}}{\suba{\grt}}
    \end{equation}
    By the \textbf{c-cimpI} rule using \cref{eq:alg-usound-cimpl}, we obtain  $\Delta; \suba{\Phi_a}; \suba{\Omega}  \jtypeM{\suba{k}}{\suba{t}}{ \erty{e} }{\tcimpl{\suba{C}}{\suba{\grt}}}$.


\end{mainitem}
\end{spacing}




\begin{spacing}{1.3}
  \hspace{-1cm} \textbf{Proof of \Cref{thm:alg-typing-soundness}.2:} \\
\begin{mainitem} 
 
%%%%%%%%%%%%%%%%%%%%%%%%%%%%%%%%%%%%%%%%%%
%%%%%%%%%%%%%%%%%%%%%%%%%%%%%%%%%%%%%%%%%%
%%%%%%%%%%%%%%%%%%%%%%%%%%%%%%%%%%%%%%%%%%
  \caseL{\infanno}
  TS: $\Delta; \suba{\Phi_a}; \suba{\Omega}  \jtypeM{\suba{k}}{\suba{t}}{\erty{\eanno{e}{\grt}{k}{t}}}{\suba{\grt}}$. \\  
Since by definition,  $\forall e. ~\erty{\eanno{e}{\_}{\_}{\_}} = \erty{e}$, STS: $\Delta; \suba{\Phi_a}; \suba{\Omega}  \jtypeM{\suba{k}}{\suba{t}}{\erty{e}}{\suba{\grt}}$. \\  
By the main assumptions, we have
$\fivars{\Phi_a,\Omega} \subseteq dom(\Delta, \psi_a)~~(\star)$ and $\Delta; \suba{\Phi_a} \sat \suba{\Phi}~~(\star\star)$ \\
Using the third premise, we can show that
\begin{enumih}
\item $\fivars{\Phi_a,\Omega, \grt, k, t} \subseteq dom(\Delta, \psi_a).$
\end{enumih}
By \Cref{thm:alg-typing-soundness}.1  on the first premise using $(\star\star)$ and a), we can conclude that\\
$ \Delta; \suba{\Phi_a}; \suba{\Omega}  \jtypeM{\suba{k}}{\suba{t}}{\erty{e}}{\suba{\grt}}.$
 
 
%%%%%%%%%%%%%%%%%%%%%%%%%%%%%%%%%%%%%%%%%%
%%%%%%%%%%%%%%%%%%%%%%%%%%%%%%%%%%%%%%%%%%
%%%%%%%%%%%%%%%%%%%%%%%%%%%%%%%%%%%%%%%%%%
  \caseL{\infapp}
  TS: $\Delta; \suba{\Phi_a}; \suba{\Omega}  \jtypeM{\subaex{(k_1+k_2+k_e+\kapp)}{\theta_2}}{\subaex{(t_1+t_2+t_e+\kapp)}{\theta_2}}{\erty{e_1} \eapp \erty{e_2}}{\subaex{\grt_2}{\theta_2}}$. \\
By the main assumptions, we have
$\fivars{\Phi_a,\Omega} \subseteq dom(\Delta, \psi_a)~~(\star)$ and \\
$\Delta; \suba{\Phi_a} \sat \subaex{(\cand{\Phi_1}{\Phi_2})}{\theta_2}~~(\star\star)$ such that $\subsat{\Delta}{\theta_2}{k_2,t_2,\psi}~(\diam)$ and $\subsat{\Delta}{\theta_a}{\psi_a}$ are derivable. \\
By $(\diam)$, we can show that $\theta_2 = k_2, t_2, \theta$ such that
\begin{enumih}
\item $\theta(k_2) = K_2 $ and $\theta(t_2) = T_2$ for some $K_2$ and $T_2$.\\
\item $\subsat{\Delta}{\theta}{\psi}$ 
\end{enumih}
By \Cref{thm:alg-typing-soundness}.2  on the first premise using $(\star)$ and (b), we obtain
\begin{equation}
 \Delta; \suba{\Phi_a}; \suba{\Omega}  \jtypeM{\subta{k_1}}{\subta{t_1}}{\erty{e_1}}{\subta{\grt_1} \uarr{\subta{k_e}}{\subta{t_e}} \subta{\grt_2}}\label{eq:alg-bsound-app1}
\end{equation}
By \Cref{invariant:alg-typechecking}.2 on the first premise and $(\star)$, we get
\begin{enumih}[resume]
\item $\fivars{\grt_1 \uarr{k_e}{t_e} \grt_2, k_1, t_1, \Phi_1} \subseteq dom(\Delta, \psi, \psi_a).$
\end{enumih}
By $(\star)$ and c), we get 
\begin{enumih}[resume]
\item $\fivars{\Phi_a,\Omega, \grt_2, k_2, t_2} \subseteq k_2, t_2, dom(\Delta, \psi, \psi_a).$
\end{enumih}
By \Cref{thm:alg-typing-soundness}.2  on the third premise using (c), (d) and $(\star\star)$, we obtain
\begin{equation}
  \Delta; \suba{\Phi_a}; \suba{\Omega}  \jtypeM{K_2}{T_2}{\erty{e_2}}{\subta{\grt_1}}
  \label{eq:alg-bsound-app22}
\end{equation}
Then, by using \textbf{c-app} rule using \cref{eq:alg-bsound-app1,eq:alg-bsound-app22}, we can show that \\
$\Delta; \suba{\Phi_a}; \suba{\Omega}  \jtypeM{\subta{k_1}+\subta{k_e}+K_2}{\subta{t_1}+\subta{t_e}+T_2}{\erty{e_1} \eapp \erty{e_2}}{\subaex{\grt_2}{\theta_2}}$.\\
Note that we have $\subaex{k_2}{\theta_2} = K_2$ and
$\subaex{k_2}{\theta_2} = K_2$. Moreover,
$\subaex{t_1}{\theta_2} = \subta{t_1}$ and
$\subaex{k_1}{\theta_2} = \subta{k_1}$ (similarly for $k_e$ and $t_e$)
since $k_2,t_2$ are fresh variables.


%%%%%%%%%%%%%%%%%%%%%%%%%%%%%%%%%%%%%%%%%%
%%%%%%%%%%%%%%%%%%%%%%%%%%%%%%%%%%%%%%%%%%
%%%%%%%%%%%%%%%%%%%%%%%%%%%%%%%%%%%%%%%%%%
  \caseL{\infiApp}
  TS: $\Delta; \suba{\Phi_a}; \suba{\Omega}  \jtypeM{\subta{(k+k_e[I/i])}}{\subta{(t+t_e[I/i])}}{\erty{e} \eapp [I]}{\subta{(\grt'\{I/i\})}}$. \\
By the main assumptions, we have
$\fivars{\Phi_a,\Omega} \subseteq dom(\Delta, \psi_a)~~(\star)$ and \\
$\Delta; \suba{\Phi_a} \sat \subta{\Phi_2}~~(\star\star)$ such that $\subsat{\Delta}{\theta}{\psi}~(\diam)$ and $\subsat{\Delta}{\theta_a}{\psi_a}$ are derivable. \\
By \Cref{thm:alg-typing-soundness}.2  on the first premise using $(\star)$ and $(\diam)$, we obtain
\begin{equation}
 \Delta; \suba{\Phi_a}; \suba{\Omega}  \jtypeM{\subta{k}}{\subta{t}}{\erty{e}}{\tforall{i}{\subta{k_e}}{\subta{t_e}} \subta{\grt'}}\label{eq:alg-bsound-iApp1}
\end{equation} 
Then, by \textbf{c-iApp} rule using \cref{eq:alg-bsound-iApp1} and the second premise, we can conclude that\\  $\Delta; \suba{\Phi_a}; \suba{\Omega}  \jtypeM{\subta{k}+\subta{k_e}[I/i]}{\subta{t}+\subta{t_e}[I/i]}{\erty{e}\eapp [I]}{\subta{\grt'}\{I/i\}}$.

\end{mainitem}
\end{spacing}




\begin{spacing}{1.3}
  \hspace{-1cm} \textbf{Proof of \Cref{thm:alg-typing-soundness}.3:} \\
\begin{mainitem} 
%%%%%%%%%%%%%%%%%%%%%%%%%%%%%%%%%%%%%%%%%%
%%%%%%%%%%%%%%%%%%%%%%%%%%%%%%%%%%%%%%%%%%
%%%%%%%%%%%%%%%%%%%%%%%%%%%%%%%%%%%%%%%%%%
  \caseL{\chRnochange}
  TS: $\Delta; \suba{\Phi_a}; \suba{\Gamma'}, \tbox{\suba{\Gamma}} \jtypediff{\suba{t}}{\enoch e}{\enoch e}{\tbox{\suba{\tau}}}$.\\
  By the main assumptions, we have
  $\fivars{\Phi_a,\Gamma', \tbox{\Gamma}, \tau, t} \subseteq dom(\Delta, \psi_a)~~(\star)$ and \\
  $\Delta; \suba{\Phi_a} \sat \suba{(\cand{\ceq{0}{t}}{\cexists{t'}{\scost}{\Phi}})}~~(\star\star)$ \\
  Using $(\star)$ and the first premise, we can show that
  \begin{enumih}
  \item $\fivars{\Phi_a,\Gamma, \tau, t'} \subseteq t', dom(\Delta, \psi_a).$
  \end{enumih}
  Using $(\star)$,  $(\star\star)$'s derivation must be in a form such that we have
  \begin{enumih} [resume]
  \item $\Delta; \suba{\Phi_a} \sat \ceq{0}{\suba{t}}$
  \item $\Delta \sty{T'}{\scost}$ for some $T'$
  \item $\Delta; \suba{\Phi_a} \sat \subaex{\Phi}{t' \mapsto T'}$
  \end{enumih}

By \Cref{thm:alg-typing-soundness}.3 on the premise using a), d) and $(\star)$, we can show that
  \begin{equation}
    \label{eq:alg-bsound-noch}
    \Delta;\suba{\Phi_a}; \suba{\tbox{\Gamma}}  \jtypediff{T'}{\erty{e}}{\erty{e}}{\suba{\tau}}
  \end{equation}
  By the \textbf{c-nochange} rule using \cref{eq:alg-bsound-noch}, we obtain  $\Delta; \suba{\Phi_a}; \suba{\Gamma'}, \tbox{\suba{\Gamma}}  \jtypediff{0}{\enoch \erty{e} }{\enoch \erty{e} }{\tbox{\suba{\tau}}}$.\\
  By the \textbf{c-r-}${\pmb{\sqsubseteq}}$ rule using this and b), we obtain $\Delta; \suba{\Phi_a}; \suba{\Gamma'}, \tbox{\suba{\Gamma}} \jtypediff{\suba{t}}{\enoch e}{\enoch e}{\tbox{\suba{\tau}}}$.
 
 
%%%%%%%%%%%%%%%%%%%%%%%%%%%%%%%%%%%%%%%%%%
%%%%%%%%%%%%%%%%%%%%%%%%%%%%%%%%%%%%%%%%%%
%%%%%%%%%%%%%%%%%%%%%%%%%%%%%%%%%%%%%%%%%%
  \caseL{\chRcaseL}
TS:\begin{mathpar}
\Delta; \suba{\Phi_a}; \suba{\Gamma} \jtypediff{\suba{t}}{\hspace{-1em}
       \begin{minipage}[c]{10em}
         ~ $\ecase e \eof \enil \, \rightarrow \erty{e_1}$ \\
         $~~~~~~~~|~h\,::_{N} tl\, \rightarrow \erty{e_2}$ \\
         $~~~~~~~~|~h::_{C} tl \rightarrow \erty{e_3}$
       \end{minipage}\hspace{-1em}
     }{\hspace{-1em}
       \begin{minipage}[c]{10em}
         ~ $\ecase e' \eof \enil \, \rightarrow \erty{e_1'}$ \\
         $~~~~~~~~|~h\,::_{N} tl\, \rightarrow \erty{e_2'}$ \\
         $~~~~~~~~|~h::_{C} tl \rightarrow \erty{e_3'}$
       \end{minipage}
     }{\suba{\tau'}}
\end{mathpar}\\
  By the main assumptions, we have
  $\fivars{\Phi_a,\Gamma, \tau', t} \subseteq dom(\Delta, \psi_a)~~(\star)$ and \\
  $\Delta; \suba{\Phi_a} \sat \suba{(\cexistsS{(\psi)}{\cand{\Phi_e}{\cexists{t_2}{\scost}{\Phi_{body}}}})}~~(\star\star)$ \\
By \Cref{invariant:alg-typechecking} using the first premise and $(\star)$, we get $ \fivars{\tlist{n}{\alpha}{\tau}, t_1,\Phi_e} \subseteq dom(\Delta, \psi; \psi_a)~(\diam)$.\\
Using $(\star)$ and $ (\diam)$,  $(\star\star)$'s derivation must be in a form such that we have
\begin{enumih}
\item $\subsat{\Delta}{\theta}{\psi}$
\item $\Delta; \suba{\Phi_a} \sat \subta{\Phi_e}$
\item $\Delta \sty{T_2}{\scost}$
\item $\Delta; {\ceq{\subta{n}}{0}} \wedge \suba{\Phi_a} \sat \subta{\Phi_1}$
\item $\sorted{i}, \Delta; {\ceq{\subta{n}}{i+1}} \wedge \suba{\Phi_a} \sat \subaex{\Phi_2}{\theta, t_2 \mapsto T_2}$
\item $\sorted{i},\sorted{\beta}, \Delta; {\ceq{\subta{n}}{i+1}} \wedge{\ceq{\subta{\alpha}}{\beta+1}} \wedge \suba{\Phi_a} \sat \subaex{\Phi_3}{\theta, t_2 \mapsto T_2}$
\item $\Delta; \suba{\Phi_a} \sat \ceq{\subta{t_1}+T_2}{\suba{t}}$
\end{enumih}
By \Cref{thm:alg-typing-soundness}.4 on the first premise using b) and $(\star)$, we can show that
  \begin{equation}
    \label{eq:alg-bsound-caseL1}
    \Delta;\suba{\Phi_a}; \suba{\Gamma}  \jtypediff{\subta{t_1}}{\erty{e}}{\erty{e'}}{\tlist{\subta{n}}{\subta{\alpha}}{\subta{\tau}}}
  \end{equation}

By \Cref{thm:alg-typing-soundness}.3 on the second premise using d) and $(\star)$, we can show that
  \begin{equation}
    \label{eq:alg-bsound-caseL2}
    \Delta; {\ceq{\subta{n}}{0}} \wedge \suba{\Phi_a}; \suba{\Gamma}  \jtypediff{T_2}{\erty{e_1}}{\erty{e_1'}}{{\subta{\tau'}}}
  \end{equation}

By \Cref{thm:alg-typing-soundness}.3 on the third premise using e) and $(\star)$, we can show that
  \begin{equation}
    \label{eq:alg-bsound-caseL3}
    \sorted{i}, \Delta; {\ceq{\subta{n}}{i+1}} \wedge \suba{\Phi_a}; \suba{\Gamma}  \jtypediff{T_2}{\erty{e_2}}{\erty{e_2'}}{{\subta{\tau'}}}
  \end{equation}

By \Cref{thm:alg-typing-soundness}.3 on the fourth premise using f) and $(\star)$, we can show that
  \begin{equation}
    \label{eq:alg-bsound-caseL4}
    \sorted{i}, \sorted{\beta}, \Delta; {\ceq{\subta{n}}{i+1}} \wedge{\ceq{\subta{\alpha}}{\beta+1}} \wedge \suba{\Phi_a}; \suba{\Gamma}  \jtypediff{T_2}{\erty{e_3}}{\erty{e_3'}}{{\subta{\tau'}}}
  \end{equation}
  Then by \textbf{c-r-caseL} rule using
  \cref{eq:alg-bsound-caseL1,eq:alg-bsound-caseL2,eq:alg-bsound-caseL3,eq:alg-bsound-caseL4},
  we can show that 
 \begin{mathpar}
\Delta; \suba{\Phi_a}; \suba{\Gamma} \jtypediff{\subta{t_1}+T_2}{\hspace{-1em}
       \begin{minipage}[c]{10em}
         ~ $\ecase e \eof \enil \, \rightarrow \erty{e_1}$ \\
         $~~~~~~~~|~h\,::_{N} tl\, \rightarrow \erty{e_2}$ \\
         $~~~~~~~~|~h::_{C} tl \rightarrow \erty{e_3}$
       \end{minipage}\hspace{-1em}
     }{\hspace{-1em}
       \begin{minipage}[c]{10em}
         ~ $\ecase e' \eof \enil \, \rightarrow \erty{e_1'}$ \\
         $~~~~~~~~|~h\,::_{N} tl\, \rightarrow \erty{e_2'}$ \\
         $~~~~~~~~|~h::_{C} tl \rightarrow \erty{e_3'}$
       \end{minipage}
     }{\suba{\tau'}}
\end{mathpar}\\
We conclude by applying \textbf{c-r-}${\pmb{\sqsubseteq}}$ rule to this using g).


 
%%%%%%%%%%%%%%%%%%%%%%%%%%%%%%%%%%%%%%%%%%
%%%%%%%%%%%%%%%%%%%%%%%%%%%%%%%%%%%%%%%%%%
%%%%%%%%%%%%%%%%%%%%%%%%%%%%%%%%%%%%%%%%%%
  \caseL{\chRconsbox}
 TS: $\Delta; \suba{\Phi_a}; \suba{\Gamma} \jtypediff{\suba{t}}{\econsNC(\erty{e_1},\erty{e_2})}{\econsNC(\erty{e_1'},\erty{e_2'})}{\tlist{\suba{n}}{\suba{\alpha}}{\suba{\tau}}}$.\\
 By the main assumptions, we have
  $\fivars{\Phi_a,\Gamma, \tlist{n}{\alpha}{\tau}, t} \subseteq dom(\Delta, \psi_a)~~(\star)$ and \\
 $\Delta; \suba{\Phi_a} \sat \suba{(\cexists{t_1}{\scost}{\cand{\Phi_1}{\cexists{t_2}{\scost}{\cexists{i}{\ssize}{\Phi_2'}}}})}~~(\star\star)$ \\
Using $(\star)$,  $(\star\star)$'s derivation must be in a form such that we have
\begin{enumih}
\item $\Delta \sty{T_1}{\scost}$ 
\item  $\Delta \sty{T_2}{\scost}$ 
\item $\Delta; \suba{\Phi_a} \sat \subaex{\Phi_1}{ t_1 \mapsto T_1}$
\item  $\Delta \sty{I}{\ssize}$ 
\item $\Delta; \suba{\Phi_a} \sat \subaex{\Phi_2}{t_2 \mapsto T_2, i \mapsto I}$
\item $\Delta; \suba{\Phi_a} \sat \ceq{(I+1)}{\suba{n}}$
\item $\Delta; \suba{\Phi_a} \sat \ceq{(T_1+T_2)}{\suba{t}}$
\end{enumih}

By \Cref{thm:alg-typing-soundness}.3 on the third premise using $(\star)$ and c), we can show that
\begin{equation}
  \label{eq:alg-usound-cons1}
      \Delta; \suba{\Phi_a}; \suba{\Omega}  \jtypediff{T_1}{\erty{e_1}}{\erty{e_1'}}{\tbox{\suba{\tau}}}
\end{equation}

By \Cref{thm:alg-typing-soundness}.3 on the fourth premise using $(\star)$ and e), we can show that
\begin{equation}
  \label{eq:alg-usound-cons2}
      \Delta; \suba{\Phi_a}; \suba{\Omega}  \jtypediff{T_2}{\erty{e_2}}{\erty{e_2'}}{\tlist{I}{\suba{\alpha}}{\suba{\tau}}}
\end{equation}
By \textbf{c-r-cons1} typing rule using \cref{eq:alg-usound-cons1,eq:alg-usound-cons2}, we obtain
\\ $\Delta; \suba{\Phi_a}; \suba{\Gamma} \jtypediff{T_1+T_2}{\econsNC(\erty{e_1},\erty{e_2})}{\econsNC(\erty{e_1'},\erty{e_2'})}{\tlist{I+1}{\suba{\alpha}}{\suba{\tau}}}$. \\
We conclude by applying \textbf{c-r-}${\pmb{\sqsubseteq}}$ rule to this using f) and g).



%%%%%%%%%%%%%%%%%%%%%%%%%%%%%%%%%%%%%%%%%%
%%%%%%%%%%%%%%%%%%%%%%%%%%%%%%%%%%%%%%%%%%
%%%%%%%%%%%%%%%%%%%%%%%%%%%%%%%%%%%%%%%%%%
\caseL{\chRappfun} 
\\ TS: $\Delta; \suba{\Phi_a}; \suba{\Gamma}  \jtypediff{\suba{t}}{\erty{e_1} \eapp \erty{e_2}}{\erty{e_2'}}{\tch{\suba{\grt}}{\suba{\grt'}}}$. \\
By the main assumptions, we have
$\fivars{\Phi_a,\Gamma, \tch{\grt}{\grt'}, t} \subseteq dom(\Delta, \psi_a)~~(\star)$ and \\
$\Delta; \suba{\Phi_a} \sat \suba{({\cexistsS{(\psi)}{\cand{\Phi_1}{\cand{(\cexists{t_2}{\scost}{\cand{\Phi_2}{\ceq{t_1+t_2+t_e+\kapp}{t}}})}{\Phi_3}}}})}~~(\star\star)$ such that  $\subsat{\Delta}{\theta_a}{\psi_a}$ is derivable. \\
By \Cref{invariant:alg-typechecking} using $(\star)$ and the first premise, we get $ \fivars{\grt_1 \uarr{k_e}{t_e} \grt_2,k_1, t_1,\Phi_1} \subseteq dom(\Delta, \psi; \psi_a)~(\diam)$.\\
Using $(\star)$ and $ (\diam)$,  $(\star\star)$'s derivation must be in a form such that we have
\begin{enumih}
\item $\subsat{\Delta}{\theta}{\psi}$
\item $\Delta; \suba{\Phi_a} \sat \subta{\Phi_1}$
\item $\Delta; \suba{\Phi_a} \sat \subaex{\Phi_2}{\theta, t_2 \mapsto T_2}$
\item $\Delta; \suba{\Phi_a} \sat \subta{\Phi_3}$
\item $\Delta; \suba{\Phi_a} \sat \ceq{\subta{t_1}+\subta{t_e}+T_2+\kapp}{\suba{t}}$
\end{enumih}
By \Cref{thm:alg-typing-soundness}.2 on the first premise using $(\star)$, a) and b), we can show that
\begin{equation}
  \label{eq:alg-usound-app-e1}
      \Delta; \suba{\Phi_a}; \trm{\suba{\Gamma}}{1}  \jtypeM{\subta{k_1}}{\subta{t_1}}{\erty{e_1}}{\subta{\grt_1} \uarr{\subta{k_e}}{\subta{t_e}} \subta{\grt_2}}
\end{equation}
From $(\star)$ and $(\diam)$, we can show that
\begin{enumih}[resume]
 \item $\fivars{\Phi_a, \Gamma, \tch{\grt_1}{\grt'}, t_2} \subseteq t_2, dom(\Delta, \psi; \psi_a)$
\end{enumih}
By \Cref{thm:alg-typing-soundness}.3 on the third premise using c), $(\star)$ and $(\diam)$, we obtain
\begin{equation}
  \label{eq:alg-usound-app-e2}
     \Delta; \suba{\Phi_a}; \suba{\Gamma} \jtypediff{T_2}{\erty{e_2}}{\erty{e_2'}}{\tch{\subta{\grt_1}}{\subta{\grt'}}}
   \end{equation}
   
   By \Cref{thm:alg-unary-subtyping-soundness} on the fourth 
   premise using ($\diam$), ($\star$) and (d), we obtain
\begin{equation}
  \label{eq:alg-usound-app-e3}
   \Delta ; \suba{\Phi_a}  \jasubtype{\subta{\grt_2}}{\suba{\grt}}
\end{equation}
  By \textbf{U} subtyping rule using \cref{eq:alg-usound-app-e3} and \textbf{u-refl} subtyping rule, we obtain
  \begin{equation}
    \label{eq:alg-usound-app-e4}
    \Delta ; \suba{\Phi_a}  \jsubtype{\tch{\subta{\grt_2}}{\suba{\grt'}}}{\tch{\suba{\grt}}{\suba{\grt'}}}
  \end{equation}
Then by the \textbf{c-r-app-e} rule using \cref{eq:alg-usound-app-e1,eq:alg-usound-app-e2}, we can show that\\ $\Delta; \suba{\Phi_a}; \suba{\Gamma}  \jtypediff{\subta{t_1}+\subta{t_e}+T_2+\kapp}{\erty{e_1} \eapp \erty{e_2}}{\erty{e_2'}}{\tch{\suba{\grt_2}}{\suba{\grt'}}}$. \\
Applying \textbf{c-r-}${\pmb{\sqsubseteq}}$ rule to this using (e) and \cref{eq:alg-usound-app-e4}, we can conclude as \\ $\Delta; \suba{\Phi_a}; \suba{\Gamma}  \jtypediff{\suba{t}}{\erty{e_1} \eapp \erty{e_2}}{\erty{e_2'}}{\tch{\suba{\grt}}{\suba{\grt'}}}$.

\end{mainitem}
\end{spacing}



\begin{spacing}{1.3}
  \hspace{-1cm} \textbf{Proof of \Cref{thm:alg-typing-soundness}.4:} \\
\begin{mainitem} 

%%%%%%%%%%%%%%%%%%%%%%%%%%%%%%%%%%%%%%%%%%
%%%%%%%%%%%%%%%%%%%%%%%%%%%%%%%%%%%%%%%%%%
%%%%%%%%%%%%%%%%%%%%%%%%%%%%%%%%%%%%%%%%%%
  \caseL{\infRanno}
  TS: $\Delta; \suba{\Phi_a}; \suba{\Omega}  \jtypediff{\suba{t}}{\erty{\eannobi{e}{\tau}{t}}}{\erty{\eannobi{e'}{\tau}{t}}}{\suba{\tau}}$. \\  
Since by definition,  $\forall e. ~\erty{\eannobi{e}{\_}{\_}} = \erty{e}$, STS: $\Delta; \suba{\Phi_a}; \suba{\Gamma}  \jtypediff{\suba{t}}{\erty{e}}{\erty{e'}}{\suba{\tau}}$. \\  
By the main assumptions, we have
$\fivars{\Phi_a,\Gamma} \subseteq dom(\Delta, \psi_a)~~(\star)$ and $\Delta; \suba{\Phi_a} \sat \suba{\Phi}~~(\star\star)$ \\
Using the third premise, we can show that
\begin{enumih}
\item $\fivars{\Phi_a,\Gamma, \tau, k, t} \subseteq dom(\Delta, \psi_a).$
\end{enumih}
By \Cref{thm:alg-typing-soundness}.4  on the first premise using $(\star\star)$ and a), we can conclude that\\
$ \Delta; \suba{\Phi_a}; \suba{\Gamma}  \jtypediff{\suba{t}}{\erty{e}}{\erty{e'}}{\suba{\tau}}.$
 

%%%%%%%%%%%%%%%%%%%%%%%%%%%%%%%%%%%%%%%%%%
%%%%%%%%%%%%%%%%%%%%%%%%%%%%%%%%%%%%%%%%%%
%%%%%%%%%%%%%%%%%%%%%%%%%%%%%%%%%%%%%%%%%%
  \caseL{\infRder}
  TS: $\Delta; \suba{\Phi_a}; \suba{\Omega}  \jtypeM{\subta{t}}{\erty{e}}{\erty{e'}}{\subta{\tau}}$. \\
By the main assumptions, we have
$\fivars{\Phi_a,\Gamma} \subseteq dom(\Delta, \psi_a)~~(\star)$ and \\
$\Delta; \suba{\Phi_a} \sat \subta{\Phi}~~(\star\star)$ such that $\subsat{\Delta}{\theta}{\psi}~(\diam)$ and $\subsat{\Delta}{\theta_a}{\psi_a}$ are derivable. \\
By \Cref{thm:alg-typing-soundness}.4  on the first premise using $(\star)$ and $(\diam)$, we obtain
\begin{equation}
 \Delta; \suba{\Phi_a}; \suba{\Gamma}  \jtypediff{\subta{t}}{\erty{e}}{\erty{e'}}{\tbox{\subta{\tau}}}\label{eq:alg-bsound-der1}
\end{equation} 
Then, by \textbf{c-der} rule using \cref{eq:alg-bsound-der1} and the second premise, we can conclude that\\  $\Delta; \suba{\Phi_a}; \suba{\Gamma}  \jtypediff{\subta{t}}{\erty{e}}{\erty{e'}}{\subta{\tau}}$.


\end{mainitem}
\end{spacing}

\end{proof}

%%% Local Variables:
%%% mode: latex
%%% TeX-master: "main"
%%% End:
