# Supplementary material for: Bidirectional Type Checking for Relational Properties
Source: arXiv:1812.05067 source file (2018-12-12)
Supplement: Supplementary file 12 [file alg-sub-completeness.tex]

\begin{thm}[Completeness of the Unary Algorithmic Subtyping]\label{thm:alg-subtyping-completeness}
  Assume that $\Delta; \Phi_a \jasubtype{\grt'}{\grt}$. Then
  $\exists\, \Phi.$ such that
  $\Delta ; \Phi_a \jalgasubtype{\grt'}{\grt}{\Phi}$ and
  $\Delta; \Phi_a \sat \Phi$.
\end{thm} 

\begin{proof}
  By induction on the unary subtyping derivation.
\end{proof}

%%% Local Variables:
%%% mode: latex
%%% TeX-master: "main"
%%% End:
