# Supplementary material for: Bidirectional Type Checking for Relational Properties
Source: arXiv:1812.05067 source file (2018-12-12)
Supplement: Supplementary file 13 [file alg-sub-soundness.tex]

\begin{thm}[Soundness of the Algorithmic Unary Subtyping]\label{thm:alg-unary-subtyping-soundness}
    Assume that 
    \begin{enumerate}
    \item $\Delta ; \psi_a; \Phi_a \jalgasubtype{\grt'}{\grt}{\Phi}$
    \item $\fivars{\Phi_a,\grt, \grt'} \subseteq \Delta, \psi_a$ 
    % \item $\Delta; \psi_a; \Phi_a \awfty{\grt} $
    % \item $\Delta; \psi_a; \Phi_a \awfty{\grt'} $
    \item $\Delta; \suba{\Phi_a} \sat \suba{\Phi}$ is
      provable s.t $\subsat{\Delta}{\theta_a}{\psi_a}$ is derivable.
    \end{enumerate}
    Then $\Delta ; \suba{\Phi_a} \jasubtype{\suba{\grt'}}{\suba{\grt}}$.
    
\end{thm} 
\begin{proof}
  By induction on the algorithmic unary subtyping derivation.
\end{proof}
%%% Local Variables:
%%% mode: latex
%%% TeX-master: "main"
%%% End:
