# Supplementary material for: Bidirectional Type Checking for Relational Properties
Source: arXiv:1812.05067 source file (2018-12-12)
Supplement: Supplementary file 14 [file alg-subtyping-rules.tex]

\newcommand{\astuint}
{
\inferrule{ 
}
{
  \Delta; \psi_a; \Phi_a  \jalgasubtype{\tint}{\tint}{\ctrue}
}~\textbf{alg-u-int}
}


\newcommand{\astuunit}
{
\inferrule{ 
}
{
  \Delta; \psi_a; \Phi_a  \jalgasubtype{\tunit}{\tunit}{\ctrue}
}~\textbf{alg-u-unit}
}


\newcommand{\astufun}
{
\inferrule{
\Delta; \psi_a; \Phi_a \jalgasubtype{\grt_1'}{\grt_1}{\Phi_1} \\ 
\Delta; \psi_a; \Phi_a \jalgasubtype{\grt_2}{\grt_2'}{\Phi_2}
}
{
\Delta; \psi_a; \Phi_a  \jalgasubtype{\grt_1 \uarr{k}{t} \grt_2}{\grt_1' \uarr{k'}{t'} \grt_2'}{\cand{\Phi_1}{\cand{\Phi_2}{\cand{\Phi_3}{\cand{\cleq{k'}{k}}{\cleq{t}{t'}}}}}}
}~\textbf{alg-u-fun} 
}


\newcommand{\astuforall}
{
\inferrule
{
i, \Delta; \psi_a; \Phi_a \jalgasubtype{\grt}{\grt'}{\Phi_1} \\
}
{
\Delta; \psi_a; \Phi_a  \jalgasubtype{\tforall{i}{k}{t} \grt}{\tforall{i}{k'}{t'} \grt'}{\cforall{i}{\sort}{\cand{\Phi_1}{\cand{\Phi_2}{\cand{\cleq{k'}{k}}{\cleq{t}{t'}}}}}}
}\textbf{alg-u-$\forall$} 
}


\newcommand{\astuprod}
{
\inferrule{
\Delta; \psi_a; \Phi_a \jalgasubtype{\grt_1}{\grt_1'}{\Phi_1} \\ 
\Delta; \psi_a; \Phi_a \jalgasubtype{\grt_2}{\grt_2'}{\Phi_2}
}{
\Delta; \psi_a; \Phi_a \jalgasubtype{\grt_1 \ttimes \grt_2}{\grt_1' \ttimes \grt_2'}{\cand{\Phi_1}{\Phi_2}}
}~\textbf{alg-u-prod} 
}

\newcommand{\astusum}
{
\inferrule{
\Delta; \psi_a; \Phi_a \jalgasubtype{\grt_1}{\grt_1'}{\Phi_1} \\ 
\Delta; \psi_a; \Phi_a \jalgasubtype{\grt_2}{\grt_2'}{\Phi_2}
}{
\Delta; \psi_a; \Phi_a \jalgasubtype{\grt_1 \tsum \grt_2}{\grt_1' \tsum \grt_2'}{\cand{\Phi_1}{\Phi_2}}
}~\textbf{alg-u-sum} 
}


\newcommand{\astulist}
{
\inferrule{
\Delta; \psi_a; \Phi_a \jalgasubtype{\grt}{\grt'}{\Phi_1} \\
\Phi = \cand{\ceq{n}{n'}}{\Phi}
}
{
\Delta; \psi_a; \Phi_a \jalgasubtype{\ulist{n}{\grt}}{\ulist{n'}{\grt'}}{\Phi}
}~\textbf{alg-u-list} 
}


\newcommand{\astuexists}
{
\inferrule
{
i, \Delta; \psi_a; \Phi_a \jalgasubtype{\grt}{\grt'}{\Phi} \\
i \not\in FV(\Phi_a)
}
{
\Delta; \psi_a; \Phi_a \jalgasubtype{\texists{i} {\grt}}{\texists{i} {\grt'}}{\cforall{i}{\sort}{\Phi}}
}~\textbf{alg-u-$\exists$} 
}



\newcommand{\astucimpl}
{
\inferrule{
\Delta; \psi_a; \Phi_a \jalgasubtype{\grt}{\grt'}{\Phi}
}
{
\Delta; \psi_a; \Phi_a \jalgasubtype{\tcimpl{C}{\grt}}{\tcimpl{C'}{\grt'}}{\cand{(\cimpl{C'}{C})}{\Phi}}
}\textbf{alg-u-c-impl}
}


\newcommand{\astucprod}
{
\inferrule{
\Delta; \psi_a; \Phi_a \jalgasubtype{\grt}{\grt'}{\Phi}
}
{
\Delta; \psi_a; \Phi_a \jalgasubtype{\tcprod{C}{\grt}}{\tcprod{C'}{\grt'}}{\cand{(\cimpl{C}{C'})}{\Phi}}
}\textbf{alg-u-c-prod}
}

\newcommand{\asturefl}
{
\inferrule
{
}
{\Delta; \psi_a; \Phi_a \jalgasubtype{\grt}{\grt}{\ctrue}
}\textbf{alg-u-refl}
}




%%% Local Variables:
%%% mode: latex
%%% TeX-master: "main"
%%% End:
