# Supplementary material for: Bidirectional Type Checking for Relational Properties
Source: arXiv:1812.05067 source file (2018-12-12)
Supplement: Supplementary file 15 [file alg-ty-eq-completeness.tex]

\begin{thm}[Completeness of the Binary Algorithmic Type Equivalence]\label{thm:alg-ty-eq-completeness}
   Assume that $\Delta; \Phi_a \jeqtype{\tau'}{\tau}$. Then $\exists\, \Phi.$ such that  $\Delta ; \Phi_a \jalgeqtype{\tau'}{\tau}{\Phi}$ and $\Delta; \Phi_a \sat \Phi$.
        
\end{thm} 

\begin{proof}
  By induction on the binary subtyping derivation.
\end{proof}

%%% Local Variables:
%%% mode: latex
%%% TeX-master: "main"
%%% End:
