# Supplementary material for: Bidirectional Type Checking for Relational Properties
Source: arXiv:1812.05067 source file (2018-12-12)
Supplement: Supplementary file 16 [file alg-ty-eq-soundness.tex]

\begin{thm}[Soundness of the Algorithmic Binary Type Equality]\label{thm:alg-ty-eq-soundness}
    Assume that
    \begin{enumerate}
    \item  $\Delta ; \psi_a; \Phi_a \jalgeqtype{\tau'}{\tau}{\Phi}$
    \item $\fivars{\Phi_a,\tau, \tau'} \subseteq \Delta, \psi_a$ 
    % \item $\Delta; \psi_a; \Phi_a \wfty{\tau} $
    % \item $\Delta; \psi_a; \Phi_a \wfty{\tau'} $
    \item $\Delta; \suba{\Phi_a} \sat \suba{\Phi}$ is
      provable s.t $\subsat{\Delta}{\theta_a}{\psi_a}$ is derivable.
    \end{enumerate}
    Then $\Delta ; \suba{\Phi_a}  \jeqtype{\suba{\tau'}}{\suba{\tau}}$.

\end{thm} 
\begin{proof}
  By induction on the algorithmic binary type equivalence derivation.
\end{proof}

%%% Local Variables:
%%% mode: latex
%%% TeX-master: "main"
%%% End:
