# Supplementary material for: Bidirectional Type Checking for Relational Properties
Source: arXiv:1812.05067 source file (2018-12-12)
Supplement: Supplementary file 17 [file alg-type-eq-rules.tex]

\begin{figure*}
  \fbox{$\Delta; \psi_a; \Phi_a \jalgasubtype{\grt_1}{\grt_2}{\Phi}$}~~~checks whether $\grt_1$ is subtype of $\grt_2$ and generates constraints $\Phi$\\
  \fbox{$\Delta; \psi_a; \Phi_a \jalgeqtype{\tau_1}{\tau_2}{\Phi}$}~~~checks whether $\tau_1$ is equivalent to $\tau_2$ and generates constraints $\Phi$\\

% The converse of the conlusion in rules marked * can be proved using
% other rules (given their premises).\\
% The rules marked with $(\dagg)$ are also valid for a judgment.

\raggedright
\begin{mathpar}
\astint
%
\and
%
% \astintbox
% %
\and
%
\astunit
%
\and
%
% \astunitbox
% %
\and
%
\astfun
%
\and
%
\astprod
%
\and
%
\astsum
%
\and
%
\astlist
%
\and
%
% \astlistzero
% %
% \and
%
\astforall
%
\and
%
\astexists
%
\and
%
% \astunrel
% %
% \and
%
% \astboxL
% %
% \and
% %
\astboxB
%
\and
% \astboxBR
% %
% \and
% %
% \astboxpushl
% %
% \and
% %
% \astboxpushr
% %
% \and
% %
%
% \astfunbox
% %
% \and
% %
% \astlistboxl
% %
% \and
% %
% \astlistboxr
% %
% \and
% %
% \astprodboxl
% %
% \and
% %
% \astprodboxr
% %
% \and
%
% \astsumboxl
% %
% \and
% %
% \astsumboxr
% %
% \and
%
% \astforallboxl
% %
% \and
% %
% \astforallboxr
% %
% \and
% %
% \astexistsboxl
% %
% \and
% %
% \astexistsboxr
% %
% \and
% %
\astunrel
%
\and
%
\astcimpl
%
\and
%
\astcprod
\end{mathpar} 
%\nocaptionrule
\caption{Algortihmic type equivalence rules}
\label{fig:subtyping-rules}  
\end{figure*} 

%%% Local Variables:
%%% mode: latex
%%% TeX-master: "main"
%%% End:
