# Supplementary material for: Bidirectional Type Checking for Relational Properties
Source: arXiv:1812.05067 source file (2018-12-12)
Supplement: Supplementary file 18 [file alg-typing-rules-defs.tex]

\newcommand{\infRswitch}
{
  \inferrule
  {
    \Delta; \psi_a; \Phi; \trm{\Gamma}{1}  \infexec{e_1}{\grt_1}{\psi_1}{\_}{t_1}{\Phi_1}\\
    \Delta; \psi_a; \Phi; \trm{\Gamma}{2}  \infexec{e_2}{\grt_2}{\psi_2}{k_2}{\_}{\Phi_2}
  }
  {
    \bctx  \infdiff{\eswitch e_1}{\eswitch e_2}{\tch{\grt_1}{\grt_2}}{\psi_1,\psi_2}{t_1-k_2}{\cand{\Phi_1}{\Phi_2
  }}}~\textbf{alg-r-switch$\uparrow$}
}

\newcommandx{\chRswitch}[1][1=]
{
  \inferrule
  {
    \freshCost{k_1#1, t_1#1, k_2#1, t_2#1} \\
    \Delta; k_1#1, t_1#1, \psi_a; \Phi; \trm{\Gamma}{1}  \chexec{e_1#1}{\grt_1}{k_1#1}{t_1#1}{\Phi_1#1}\\
    \Delta; k_2#1, t_2#1, \psi_a; \Phi; \trm{\Gamma}{2}  \chexec{e_2#1}{\grt_2}{k_2#1}{t_2#1}{\Phi_2#1}
  }
  {
    \bctx  \chdiff{\eswitch e_1#1}{\eswitch e_2#1}{t}{\tch{\grt_1}{\grt_2}}{\cexists{k_1,t_1}{\scost}{(\cand{\Phi_1#1}{\cexists{k_2#1,t_2#1}{\scost}{\cand{\Phi_2#1}{\ceq{t_1#1-k_2#1}{t}}}
  })}}
   }~\textbf{alg-r-switch$\downarrow$}
}

\newcommand{\chRnochange}
{
  \inferrule
  {
    \freshCost{t'} \\
    \Delta; {t', \psi_a}; \Phi_a; \tbox{\Gamma}  \chdiff{e}{e}{\tau}{t'}{\Phi}
  }
  {
    \Delta; \psi_a; \Phi_a; \Gamma', \tbox{\Gamma} \chdiff{\enoch e}{\enoch e}{\tbox{\tau}}{t}{\cand{\ceq{0}{t}}{(\cexists{t'}{\scost}{\Phi})}}
  } ~\textbf{alg-r-nochange-$\downarrow$}
%
}

\newcommand{\infRder}
{
\inferrule
{
  \bctx \infdiff{e_1}{e_2}{\tbox{\tau}}{\psi}{t}{\Phi}
}
{
  \bctx \infdiff{\eder e_1}{\eder e_2}{\tau}{\psi}{t}{\Phi}
}~\textbf{alg-r-der-$\uparrow$}
}


\newcommandx{\chRder}[2][1=\psi_a, 2=]
{
\inferrule
{
  \Delta; #1; \Phi_a; \Gamma \chdiff{e_1#2}{e_2#2}{\tbox{\tau}}{t}{\Phi}
}
{
  \Delta; #1; \Phi_a; \Gamma \chdiff{\eder e_1#2}{\eder e_2#2}{\tau}{t}{\Phi}
}~\textbf{alg-r-der-$\downarrow$} 
}



\newcommand{\infconst}
{
\inferrule
{
}
{ 
\uctx \infexec{\kw{n}}{\tint}{\emptypsi}{0}{0}{\ctrue}
} ~\textbf{alg-u-n-$\uparrow$} 
}


\newcommand{\infRconst}
{
\inferrule
{
}
{ 
\bctx \infdiff{\kw{n}}{\kw{n}}{\trint}{\emptypsi}{0}{\ctrue}
} ~\textbf{alg-r-n-$\uparrow$} 
}



\newcommand{\infunit}
{
\inferrule
{
}
{ 
\uctx \infexec{()}{\tunit}{\emptypsi}{0}{0}{\ctrue}
} ~\textbf{alg-u-unit-$\uparrow$} 
}


\newcommand{\infRunit}
{
\inferrule
{
}
{ 
\bctx \infdiff{()}{\kw{n}}{\trunit}{\emptypsi}{0}{\ctrue}
} ~\textbf{alg-r-unit-$\uparrow$} 
}


\newcommandx{\infvar}[1][1=\psi]{
\inferrule
{ 
\Omega(x) = \grt
}
{
\Delta; #1; \Phi_a; \Omega  \infexec{x}{\grt}{\emptypsi}{0}{0}{\ctrue}
} ~\textbf{alg-u-var-$\uparrow$}
}

\newcommand{\infRvar}{
\inferrule 
{ 
\Gamma(x) = \tau
}
{
\bctx \infdiff{x}{x}{\tau}{\emptypsi}{0}{\ctrue}
} ~\textbf{alg-r-var-$\uparrow$}
}


\newcommand{\chpair}
{
  \inferrule
  {
    \freshCost{k_1,t_1,k_2,t_2} \\
    \Delta; k_1, t_1, \psi_a; \Phi_a; \Omega \chexec{e_1}{\grt_1}{k_1}{t_1}{\Phi_1} \\
    \Delta; k_2, t_2, \psi_a; \Phi_a; \Omega \chexec{e_2}{\grt_1}{k_2}{t_2}{\Phi_2}
}
{ \uctx  \chexec{\la e_1, e_2 \ra}{\grt_1 \ttimes \grt_2}{k}{t}{\cexists{k_1, t_1}{\scost}{\cand{\Phi_1}{\cexists{k_2, t_2}{\scost}{{\cand{\Phi_2}{\cand{\ceq{t_1+t_2}{t}}{\ceq{k}{k_1+k_2}}}}}}}}
}~\textbf{alg-u-prod-$\downarrow$}
}

\newcommand{\chRpair}
{
  \inferrule
  {
    \freshCost{t_1,t_2} \\
    \Delta; t_1, \psi_a; \Phi_a; \Gamma \chdiff{e_1}{e_1'}{\tau_1}{t_1}{\Phi_1} \\
    \Delta; t_1, \psi_a; \Phi_a; \Gamma \chdiff{e_2}{e_2'}{\tau_1}{t_2}{\Phi_2}
}
{ \uctx  \chdiff{\la e_1, e_2 \ra}{\la e_1', e_2' \ra}{\tau_1 \ttimes \tau_2}{t}{\cexists{t_1}{\scost}{\cand{\Phi_1}{\cexists{t_1}{\scost}{\cand{\Phi_2}{\ceq{t_1+t_2}{t}}}}}}
}~\textbf{alg-r-prod-$\downarrow$}
} 

\newcommand{\chfst}
{
\inferrule
{
\uctx  \infexec{e}{\grt_1 \ttimes \grt_2}{\psi}{k}{t}{\Phi} \\
}
{ \uctx  \infexec{\eleft(e)}{\grt_1}{\psi}{k}{t}{\Phi}
}~\textbf{alg-u-proj1-$\uparrow$}
} 


\newcommand{\chRfst}
{
\inferrule
{
\bctx  \infdiff{e}{e'}{\tau_1 \ttimes \tau_2}{\psi}{t}{\Phi}
}
{ \bctx  \infdiff{\eleft(e)}{\eleft(e')}{\tau_1}{\psi}{t}{\Phi}
}~\textbf{alg-r-proj1-$\uparrow$}
} 


\newcommand{\chsnd}
{
\inferrule
{
\uctx  \infexec{e}{\grt_1 \ttimes \grt_2}{\psi}{k}{t}{\Phi} \\
}
{ \uctx  \infexec{\eright(e)}{\grt_2}{\psi}{k}{t}{\Phi}
}~\textbf{alg-u-proj2-$\uparrow$}
} 


\newcommand{\chRsnd}
{
\inferrule
{
\bctx  \infdiff{e}{e'}{\tau_1 \ttimes \tau_2}{\psi}{t}{\Phi}
}
{ \bctx  \infdiff{\eright(e)}{\eright(e')}{\tau_2}{\psi}{t}{\Phi}
}~\textbf{alg-r-proj2-$\uparrow$}
} 

 
\newcommand{\chinl}
{
  \inferrule
{
\uctx  \chexec{e}{\grt_1}{k}{t}{\Phi} \\
\Delta, \psi_a; \Phi_a \awfty{\grt_2} 
}
{ \uctx  \chexec{\einl e}{\grt_1 \tsum \grt_2}{k}{t}{\Phi}
}~\textbf{alg-u-inl-$\downarrow$}
} 



\newcommand{\chRinl}
{
  \inferrule
{
\bctx \chdiff{e_1}{e_2}{\tau_1}{t}{\Phi} \\
\Delta, \psi_a; \Phi_a \wfty{\tau_2} 
}
{ \bctx \chdiff{\einl e_1}{\einl e_2}{\tau_1 \tsum \tau_2}{t}{\Phi}
}~\textbf{alg-r-inl-$\downarrow$}
}

\newcommand{\chinr}
{
  \inferrule
{
\uctx  \chexec{e}{\grt_2}{k}{t}{\Phi} \\
\Delta, \psi_a; \Phi_a \awfty{\grt_1} 
}
{ \uctx  \chexec{\einr e}{\grt_1 \tsum \grt_2}{k}{t}{\Phi}
}~\textbf{alg-u-inr-$\downarrow$}
} 



\newcommand{\chRinr}
{
  \inferrule
{
\bctx \chdiff{e_1}{e_2}{\tau_2}{t}{\Phi} \\
\Delta, \psi_a; \Phi_a \wfty{\tau_1} 
}
{ \bctx \chdiff{\einr e_1}{\einr e_2}{\tau_1 \tsum \tau_2}{t}{\Phi}
}~\textbf{alg-r-inr-$\downarrow$}
}


\newcommand{\chcase}
{
  \inferrule
{ 
\uctx \infexec{e}{\grt_1 \tsum \grt_2}{\psi}{k_e}{t_e}{\Phi_1}
\\
\freshCost{k',t'}\\
\Delta; {k', t', \psi,\psi_a}; {\Phi_a}; \Omega , {x}: {\grt_1}
\chexec{e_1}{\grt}{k'}{t'}{\Phi_2}\\
\Delta; {k',t',\psi,\psi_a}; {\Phi_a}; \Omega ,{y} : {\grt_2}
\chexec{e_2}{\grt}{k'}{t'}{\Phi_3} \\
\Phi = \cexistsS{(\psi)}{\cand{\Phi_1}{(\cexists{k',t'}{\scost}{\cand{\Phi_2}{\cand{\Phi_3}{\cand{\ceq{k}{k'+ k_e+\kcase}}{\ceq{t'+ t_e+\kcase}{t}}}}})}}
}
{ \uctx
  \chexec{\ecase(e,x.e_1,y.e_2)}{\grt}{k}{t}{\Phi}
}~\textbf{alg-u-case-$\downarrow$}
}

\newcommand{\chRcase}
{
  \inferrule
{ 
\bctx \infdiff{e}{e'}{\tau_1 \tsum \tau_2}{\psi}{t_e}{\Phi_1} \\
\freshCost{t'}\\
\Delta; {t', \psi,\psi_a}; {\Phi_a}; \Gamma, {x}: {\tau_1}
\chdiff{e_1}{e_1'}{\tau}{t'}{\Phi_2}\\
\Delta; {t',\psi,\psi_a}; {\Phi_a}; \Gamma,{y} : {\tau_2}
\chdiff{e_2}{e_2'}{\tau}{t'}{\Phi_3} \\
\Phi = \cexistsS{(\psi)}{\cand{\Phi_1}{(\cexists{t'}{\scost}{\cand{\Phi_2}{\cand{\Phi_3}{(\ceq{t'+ t_e}{t})}}})}}
}
{ \Delta; {\psi_a}; \Phi_a; \Gamma
  \chdiff{\ecase(e,x.e_1,y.e_2)}{\ecase(e',x.e_1',y.e_2')}{\tau}{t}{\Phi}
}~\textbf{alg-r-case-$\downarrow$}
}

\newcommand{\chfix}
{
  \inferrule
{ 
 \Delta; {\psi_a};  \Phi_a; f :  \grt_1 \uarr{k'}{t'} \grt_2, x:\grt_1, \Omega \chexec{e}{\grt_2}{k'}{t'}{\Phi}
}
{
\uctx  \chexec{\efix f(x).e}{\grt_1 \uarr{k'}{t'} \grt_2}{k}{t}{\cand{\Phi}{\cand{\ceq{k}{0}}{\ceq{0}{t}}}}
} ~\textbf{alg-u-fix-$\downarrow$}
}


\newcommand{\chRfix}
{
  \inferrule
{
 \Delta; {\psi_a};  \Phi_a; f : \tau_1 \tarrd{t'} \tau_2, x:\tau_1, \Gamma \chdiff{e}{e'}{\tau_2}{t'}{\Phi}
}
{
\bctx \chdiff{\efix f(x).e}{\efix f(x).e'}{\tau_1 \tarrd{t'} \tau_2}{t}{\cand{\Phi}{\ceq{0}{t}}}
} ~\textbf{alg-r-fix-$\downarrow$}
}


\newcommand{\chRfixBox}
{
  \inferrule
{
    % \forall x_i \in \fvars{\efixNC f(x).e}.~ \exists \tau_i. ~\Gamma(x_i) = \tbox{\tau_i}\\
    \Delta; {\psi_a};  \Phi_a; f : \tbox{(\tau_1 \tarrd{t'} \tau_2)}, x:\tau_1, \tbox{\Gamma} \chdiff{e}{e'}{\tau_2}{t'}{\Phi}
}
{
\Delta; \psi_a; \Phi_a; \Gamma', \tbox{\Gamma} \chdiff{\efixNC f(x).e}{\efixNC f(x).e}{\tbox{(\tau_1 \tarrd{t'} \tau_2)}}{t}{\cand{\Phi}{\ceq{0}{t}}}
} ~\textbf{alg-r-fix-$\downarrow\square$}
}


\newcommand{\infapp}
{
\inferrule
{
\uctx  \infexec{e_1}{\grt_1 \uarr{k_e}{t_e} \grt_2}{\psi}{k_1}{t_1}{\Phi_1} \\
\freshCost{k_2,t_2} \\
\Delta; {k_2, t_2,\psi, \psi_a}; \Phi_a; \Omega  \chexec{e_2}{\grt_1}{k_2}{t_2}{\Phi_2}
}
{
\uctx  \infexec{e_1 \eapp e_2}{\grt_2}{k_2,t_2,\psi}{k_1+k_2+k_e+\kapp}{t_1+t_2+t_e+\kapp}{\cand{\Phi_1}{\Phi_2}}
}~\textbf{alg-u-app-$\uparrow$}
}

\newcommand{\infRapp}
{
\inferrule
{
\bctx  \infdiff{e_1}{e_1'}{\tau_1 \tarrd{t_e} \tau_2}{\psi}{t_1}{\Phi_1} \\
\freshCost{t_2} \\
\Delta; {t_2,\psi, \psi_a}; \Phi_a; \Gamma \chdiff{e_2}{e_2'}{\tau_1}{t_2}{\Phi_2}
}
{
\bctx  \infdiff{e_1 \eapp e_2}{e_1' \eapp e_2'}{\tau_2}{t_2,\psi}{t_1+t_2+t_e}{\cand{\Phi_1}{\Phi_2}}
}~\textbf{alg-r-app-$\uparrow$}
}

\newcommand{\chiLam}
{
  \inferrule
  {
    \sorted{i}, \uctx \chexec{e}{\grt}{k_e}{t_e}{\Phi}
  }
  {
    \uctx  \chexec{\eLam i. e}{\tforall{i}{k_e}{t_e}
        \grt}{k}{t}{\cand{(\cforall{i}{\sort}{\Phi})}{\cand{\ceq{k}{0}}{\ceq{0}{t}}}} 
  } ~\textbf{alg-u-iLam-$\downarrow$}
}

\newcommand{\chRiLam}
{
  \inferrule
  {
    \sorted{i}, \bctx \chdiff{e}{e'}{\tau}{t_e}{\Phi}
  }
  {
    \bctx  \chdiff{\eLam i. e}{\eLam i. e'}{\tforalld{i}{t_e}
        \tau}{t}{\cand{(\cforall{i}{\sort}{\Phi})}{\ceq{0}{t}}}
  } ~\textbf{alg-r-iLam-$\downarrow$}
}
 

\newcommand{\infiApp}
{
\inferrule
{
   \uctx  \infexec{e}{\tforall{i}{k_e}{t_e} \grt'}{\psi}{k}{t}{\Phi} \\
  \Delta \sty{I}{S}
}
{
  \uctx  \infexec{e \,[I]}{\grt'\{I/i\}}{\psi}{k+k_e[I/i]}{t+t_e[I/i]}{\Phi}
} ~\textbf{alg-u-iApp-$\uparrow$}
}

\newcommand{\infRiApp}
{
\inferrule
{
  \bctx  \infdiff{e}{e'}{\tforalld{i}{t_e} \tau'}{\psi}{t}{\Phi} \\
  \Delta \sty{I}{S}
}
{
  \bctx \infdiff{e \, [I]}{e' \, [I]}{\tau'\{I/i\}}{\psi}{t+t_e[I/i]}{\Phi}
} ~\textbf{alg-r-iApp-$\uparrow$}
}


\newcommand{\chpack}{
  \inferrule
{
  \Delta; {\psi_a}; \Phi_a; \Omega  \chexec{e}{\grt\{I/i\}}{k}{t}{\Phi} \\
  \Delta \sty{I}{\sort}
}
{
  \uctx  \chexec{\epack e \ewith I }{\texists{i} \grt}{k}{t}{\Phi}
} ~\textbf{alg-u-pack-$\downarrow$}
}


\newcommand{\chRpack}{
  \inferrule
  {
    \Delta; {\psi_a}; \Phi_a; \Gamma  \chdiff{e}{e'}{\tau\{I/i\}}{t}{\Phi}\\
    \Delta  \sty{I}{\sort}
}
{
  \bctx  \chdiff{\epack e \ewith I}{\epack e' \ewith I}{\texists{i} \tau}{t}{\Phi}
} ~\textbf{alg-r-pack-$\downarrow$}
}


\newcommand{\chunpack}
{
  \inferrule 
{
  \uctx  \infexec{e_1}{\texists{i} \grt_1}{\psi}{k_1}{t_1}{\Phi_1} \\
  \freshCost{k_2,t_2} \\
  \sorted{i}, \Delta; {k_2, t_2, \psi, \psi_a}; \Phi_a; x: \grt_1, \Omega
  \chexec{e_2}{\grt_2}{k_2}{t_2}{\Phi_2} \\
i \not\in FV(\Phi_a;\Omega, \grt_2, k_2, t_2) \\
\Phi = \cexistsS{(\psi)}{}{(\cand{\cand{\Phi_1}{\cexists{k_2,t_2}{\scost}{\cforall{i}{\sort}{\Phi_2}}}}{\cand{\ceq{k}{k_1+k_2+\kunpack}}{\ceq{t_1+t_2+\kunpack}{t}}})}
}
{
  \uctx  \chexec{\eunpack e_1 \eas (x, i) \ein e_2}{\grt_2}{k}{t}{\Phi}
}~\textbf{alg-u-unpack-$\downarrow$}
}

\newcommand{\chRunpack}
{
  \inferrule 
{
  \bctx \infdiff{e_1}{e_1'}{\texists{i} {\tau_1}}{\psi}{t_1}{\Phi_1} \\
  \freshCost{t_2} \\
  \sorted{i}, \Delta; {t_2, \psi, \psi_a}; \Phi_a; x: \tau_1, \Gamma
  \chdiff{e_2}{e_2'}{\tau_2}{t_2}{\Phi_2} \\
i \not\in FV(\Phi_a;\Gamma, \tau_2, t_2) \\
\Phi = \cexistsS{(\psi)}{}{(\cand{\cand{\Phi_1}{\cexists{t_2}{\scost}{\cforall{i}{\sort}{\Phi_2}}}}{\ceq{t_1+t_2}{t}})}
}
{
  \bctx  \chdiff{\eunpack e_1 \eas (x, i) \ein e_2}{\eunpack e_1' \eas (x, i) \ein e_2'}{\tau_2}{t}{\Phi}
}~\textbf{alg-r-unpack-$\downarrow$}
}



\newcommand{\chnil}
{
\inferrule
{
\Delta, \psi_a; \Phi \awfty{\grt}
}
{
\uctx  \chexec{\enil}{\ulist{n}{\grt}}{k}{t}{\cand{\ceq{n}{0}}{\cand{\ceq{k}{0}}{\ceq{0}{t}}}}
}~\textbf{alg-u-nil-$\downarrow$}
}

\newcommand{\chRnil}
{
\inferrule
{
\Delta, \psi_a; \Phi \wfty{\tau}
}
{
\bctx  \chdiff{\enil}{\enil}{\tlist{n}{\alpha}{\tau}}{t}{\cand{\ceq{n}{0}}{\ceq{0}{t}}}
}~\textbf{alg-r-nil-$\downarrow$}
}

\newcommand{\chcons}
{
  \inferrule
{
\freshCost{k_1,t_1,k_2,t_2} \\
\freshSize{i} \\
\Delta; {k_1,t_1,\psi_a}; \Phi_a; \Omega  \chexec{e_1}{\grt}{k_1}{t_1}{\Phi_1} \\
\Delta; {i,k_2,t_2,\psi_a}; \Phi_a; \Omega
\chexec{e_2}{\ulist{i}{\grt}}{k_2}{t_2}{\Phi_2}\\
\Phi_2' = (\cand{\Phi_2}{\cand{\ceq{n}{(i+1)}}{\cand{\ceq{k}{k_1+k_2}}{\ceq{t_1+t_2}{t}}}})
}
{
\uctx \chexec{\econsC(e_1,e_2)}{\ulist{n}{\grt}}{k}{t}{\cexists{k_1,t_1}{\scost}{(\cand{\Phi_1}{\cexists{k_2,t_2}{\scost}{\cexists{i}{\ssize}{\Phi_2'}}})}}
}~\textbf{alg-u-cons-$\downarrow$}
}

\newcommand{\chRconsbox}
{
  \inferrule
{
\freshCost{t_1,t_2} \\
\freshSize{i} \\
\Delta; {t_1,\psi_a}; \Phi_a; \Gamma  \chdiff{e_1}{e_1'}{\tbox{\tau}}{t_1}{\Phi_1} \\
\Delta; {i,t_2,\psi_a}; \Phi_a; \Gamma
\chdiff{e_2}{e_2'}{\tlist{i}{\alpha}{\tau}}{t_2}{\Phi_2}\\
\Phi_2' = \cand{\Phi_2}{\cand{\ceq{n}{(i+1)}}{\ceq{t_1+t_2}{t}}}
}
{
\bctx \chdiff{\econsNC(e_1,e_2)}{\econsNC(e_1',e_2')}{\tlist{n}{\alpha}{\tau}}{t}{\cexists{t_1}{\scost}{(\cand{\Phi_1}{\cexists{t_2}{\scost}{\cexists{i}{\ssize}{\Phi_2'}}})}}
}~\textbf{alg-r-consNC-$\downarrow$}
}

\newcommand{\chRcons}
{
  \inferrule
{
\freshCost{t_1,t_2} \\
\freshSize{i,\beta} \\
\Delta; {t_1,\psi_a}; \Phi_a; \Gamma  \chdiff{e_1}{e_1'}{\tau}{t_1}{\Phi_1} \\
\Delta; {i,\beta,t_2,\psi_a}; \Phi_a; \Gamma
\chdiff{e_2}{e_2'}{\tlist{i}{\beta}{\tau}}{t_2}{\Phi_2}\\
\Phi_2' = \cand{\ceq{n}{(i+1)}}{\cexists{\beta}{\ssize}{\cand{\Phi_2}{\cand{\ceq{\alpha}{\beta+1}}{\ceq{t_1+t_2}{t}}}}}
}
{
  \bctx \chdiff{\econsC(e_1,e_2)}{\econsC(e_1',e_2')}{\tlist{n}{\alpha}{\tau}}{t}{\cexists{t_1}{\scost}{(\cand{\Phi_1}{\cexists{t_2}{\scost}{\cexists{i}{\ssize}{\Phi_2'}}})}}
}~\textbf{alg-r-consC-$\downarrow$}
}

\newcommand{\chcaseL}
{
\inferrule
{
\uctx \infexec{e}{\ulist{n}{\grt}}{\psi}{k_1}{t_1}{\Phi_1} \\
\freshCost{k_2,t_2} \\
\Delta; {k_2,t_2, \psi, \psi_a}; \cand{\ceq{n}{0}}{\Phi_a}; \Omega  \chexec{e_1}{\grt'}{k_2}{t_2}{\Phi_2} \\
\freshSize{i} \\
\sized{i},\Delta; {k_2,t_2,\psi, \psi_a};  \cand{\ceq{n}{i+1}}{\Phi_a}; h :\grt, tl:\ulist{i}{\grt}, \Omega \chexec{e_2}{\grt'}{k_2}{t_2}{\Phi_3} \\
\Phi_{body} = \cand{(\cimpl{\ceqz{n}}{\Phi_2})}{\cand{(\cforall{i}{\ssize}{\cimpl{(\ceq{n}{i+1})}{\Phi_3}})}{\cand{\ceq{k}{(k_1+k_2+\kcaseL)}}{\ceq{(t_1+t_2+\kcaseL)}{t}}}} 
}
{
\uctx \chexec{ \begin{minipage}[c]{10em}
         ~ $\ecase e \eof \enil \, \rightarrow e_1$ \\
         $~~~~~~|~h\,::_{NC} tl\, \rightarrow e_2$ \\
         $~~~~~~|~h::_{C} tl~~~ \rightarrow e_3$
       \end{minipage}\hspace{-1em}
}{\grt'}{k}{t}{\cexistsS{(\psi)}{(\cand{\Phi_1}{\cexists{k_2, t_2}{\scost}{\Phi_{body}}}})}
}~\textbf{alg-u-caseL-$\downarrow$}
}

\newcommand{\chRcaseL}
{
\inferrule
{
\bctx \infdiff{e}{e'}{\tlist{n}{\alpha}{\tau}}{\psi}{t_1}{\Phi_e}\\
\freshCost{t_2} \\
\Delta; {t_2, \psi, \psi_a}; \cand{\ceqz{n}}{\Phi_a}; \Gamma  \chdiff{e_1}{e_1'}{\tau'}{t_2}{\Phi_1} \\
\sized{i},\Delta; {t_2,\psi, \psi_a};  \cand{\ceq{n}{i+1}}{\Phi_a}; h :\tbox{\tau}, tl:\tlist{i}{\alpha}{\tau}, \Gamma \chdiff{e_2}{e_2'}{\tau'}{t_2}{\Phi_2}\\
\sized{i}, \sized{\beta},\Delta; {t_2,\psi, \psi_a};  \cand{\cand{\ceq{n}{i+1}}{\ceq{\alpha}{\beta + 1}}}{\Phi_a}; h :\tau, tl:\tlist{i}{\beta}{\tau}, \Gamma \chdiff{e_3}{e_3'}{\tau'}{t_2}{\Phi_3}\\
\Phi_{body} = \cand{\cand{(\cimpl{\ceqz{n}}{\Phi_1})}{(\cforall{i}{\ssize}{\cimpl{(\ceq{n}{i+1})}{(\cand{\Phi_2}{\cforall{\beta}{\ssize}{\cimpl{(\ceq{\alpha}{\beta+1})}{\Phi_3}}})}})}}{\ceq{t_1+t_2}{t}}
}
{
\bctx \chdiff{\hspace{-1em}
       \begin{minipage}[c]{10em}
         ~$\ecase e \eof \enil \, \rightarrow e_1$ \\
         $~~~~~~|~h\,::_{NC} tl\, \rightarrow e_2$ \\
         $~~~~~~|~h::_{C} tl~~~ \rightarrow e_3$
       \end{minipage}\hspace{-1em}
     }{\hspace{-1em}
       \begin{minipage}[c]{10em}
         ~ $\ecase e' \eof \enil \, \rightarrow e_1'$ \\
         $~~~~~~~~|~h\,::_{NC} tl\, \rightarrow e_2'$ \\
         $~~~~~~~~|~h::_{C} tl~~~ \rightarrow e_3'$
       \end{minipage}
     }{\tau'}{t}{\cexistsS{(\psi)}{(\cand{\Phi_e}{\cexists{t_2}{\scost}{\Phi_{body}}})}}
}~\textbf{alg-r-caseL-$\downarrow$}
}



\newcommand{\chlet}
{
\inferrule
{
\uctx \infexec{e_1}{\grt_1}{\psi}{k_1}{t_1}{\Phi_1} \\
\freshCost{k_2,t_2} \\
\Delta; {k_2,t_2,\psi, \psi_a};  x: \grt_1, \Omega  \chexec{e_2}{\grt_2}{k_2}{t_2}{\Phi_2} \\
\Phi_2' = \cand{\Phi_2}{\cand{\ceq{k}{(k_1+k_2+\klet)}}{\ceq{(t_1+t_2+\klet)}{t}}}
}
{
\uctx \chexec{\elet x = e_1 \ein e_2}{\grt_2}{k}{t}{\cexistsall{\psi}\cand{\Phi_1}{\cexistsC{k_2,t_2}{\Phi_2'}}}
}~\textbf{alg-u-let-$\downarrow$}
}

\newcommand{\chRlet}
{
\inferrule
{
\bctx \infdiff{e_1}{e_1'}{\tau_1}{\psi}{t_1}{\Phi_1} \\
\freshCost{t_2} \\
\Delta; {t_2,\psi, \psi_a};  x: \tau_1, \Gamma  \chdiff{e_2}{e_2'}{\tau_2}{t_2}{\Phi_2} \\
}
{
\bctx \chdiff{\elet x = e_1 \ein e_2}{\elet x = e_1' \ein e_2'}{\tau_2}{t}{\cexistsall{\psi}\cand{\Phi_1}{\cexistsC{t_2}{{\cand{\Phi_2}{\ceq{t_1+t_2}{t}}}}}}
}~\textbf{alg-r-let-$\downarrow$}
}




\newcommand{\infprimapp}
{
\inferrule
{
\primctx(\zeta) : \grt_1 \uarr{k_e}{t_e} \grt_2 \\
\freshCost{k,t} \\
\Delta; {k, t, \psi_a}; \Phi_a; \Omega  \chexec{e}{\grt_1}{k}{t}{\Phi}
}
{
\uctx  \infexec{\zeta \eapp e}{\grt_2}{k,t,\psi}{k+k_e}{t+t_e}{\Phi}
}~\textbf{alg-u-primapp-$\uparrow$}
}



\newcommand{\infRprimapp}
{
\inferrule
{
\primctx(\zeta) : \tau_1 \tarrd{t_e} \tau_2 \\
\freshCost{t} \\
\Delta; { t, \psi_a}; \Phi_a; \Gamma  \chdiff{e_1}{e_2}{\tau_1}{t}{\Phi}
}
{
\bctx  \infdiff{\zeta e_1}{\zeta \eapp e_2}{\tau_2}{t,\psi}{t+t_e}{\Phi}
}~\textbf{alg-r-primapp-$\uparrow$}
}




\newcommand{\infanno}
{\inferrule
{
  \uctx \chexec{e}{\grt}{k}{t}{\Phi}\\
  \Delta; \Phi_a \awfty{\grt} \\
  \fivars{\grt,k, t} \in \Delta
}
{
  \uctx  \infexec{\eanno{e}{\grt}{k}{t}}{\grt}{\cdot}{k}{t}{\Phi}
} ~\textbf{alg-u-anno-$\uparrow$} 
}


\newcommand{\infRanno}
{\inferrule
{
  \bctx \chdiff{e}{e'}{\tau}{t}{\Phi}\\
  \Delta; \Phi_a \wfty{\tau} \\
  \fivars{\tau,t} \in \Delta
}
{
  \bctx  \infdiff{\eannobi{e}{\tau}{t}}{\eannobi{e'}{\tau}{t}}{\tau}{\cdot}{t}{\Phi}
} ~\textbf{alg-r-anno-$\uparrow$} 
}

\newcommand{\chupdown}
{
\inferrule{
  \uctx \infexec{e}{\grt'}{\psi}{k'}{t'}{\Phi_1}\\
  \Delta; {\psi, \psi_a}; \Phi_a \jalgasubtype{\grt'}{\grt}{\Phi_2} \\
}
{ 
  \uctx \chexec{e}{\grt}{k}{t}{\cexistsall{\psi}{\cand{\cand{\Phi_1}{\Phi_2}}{\cand{\cleq{t'}{t}}{\cleq{k}{k'}}}}}
} ~\textbf{alg-$\uparrow\downarrow$}
}


\newcommand{\chRupdown}
{
\inferrule{
  \bctx \infdiff{e}{e'}{\tau'}{\psi}{t'}{\Phi_1}\\
  \Delta; {\psi, \psi_a}; \Phi_a \jalgeqtype{\tau'}{\tau}{\Phi_2} \\
}
{ 
  \bctx \chdiff{e}{e'}{\tau}{t}{\cexistsall{\psi}{\cand{\cand{\Phi_1}{\Phi_2}}{\cleq{t'}{t}}}}
} ~\textbf{alg-r-$\uparrow\downarrow$}
}

\newcommand{\chcandIntro}
{\inferrule
{
  \Delta; \psi_a; \Phi \wedge C;  \Omega \chexec{e}{\grt}{k}{t}{\Phi}
}
{
  \uctx \chexec{e}{k}{t}{\tcprod{C}{\grt}}{\cand{C}{(\cimpl{C}{\Phi})}}
} ~\textbf{alg-u-c-andI$\downarrow$}
}

\newcommand{\chRcandIntro}
{\inferrule
{
  \Delta; \psi_a; \Phi \wedge C;  \Gamma \chdiff{e_1}{e_1}{\tau}{t}{\Phi}
}
{
  \uctx \chdiff{e_1}{e_2}{\tcprod{C}{\tau}}{t}{\cand{C}{(\cimpl{C}{\Phi})}}
} ~\textbf{alg-r-c-andI$\downarrow$}
}


\newcommand{\chcimplIntro}
{
\inferrule
{
\Delta; \Phi \wedge C;  \Omega  \chexec{e}{{\grt}}{k}{t}{\Phi}
}
{
  \uctx  \chexec{e}{\tcimpl{C}{\grt}}{k}{t}{\cimpl{C}{\Phi}}
} ~\textbf{alg-u-c-impI $\downarrow$}
}



\newcommand{\chRcimplIntro}
{
\inferrule
{
\Delta; \Phi \wedge C;  \Gamma  \chdiff{e}{e'}{{\tau}}{t}{\Phi}
}
{
  \bctx  \chdiff{e}{e'}{\tcimpl{C}{\tau}}{t}{\cimpl{C}{\Phi}}
} ~\textbf{alg-r-c-impI$\downarrow$}
}


\newcommand{\infcimplElim}
{
\inferrule
{
  \uctx  \infexec{e}{\tcimpl{C}{\grt}}{\psi}{k}{t}{\Phi}
}
{
  \uctx  \infexec{\ecelim e}{\grt}{\psi}{k}{t}{\cand{C}{\Phi}}
} ~\textbf{alg-u-c-implE$\uparrow$}
}

\newcommand{\infRcimplElim}
{
\inferrule
{
  \bctx  \infdiff{e}{e'}{\tcimpl{C}{\tau}}{\psi}{t}{\Phi}
}
{ 
  \bctx  \infdiff{\ecelim e}{\ecelim e'}{\tau}{\psi}{t}{\cand{C}{\Phi}}
} ~\textbf{alg-r-c-implE$\uparrow$}
}


\newcommand{\chcandElim}
{
\inferrule
{
  \uctx \infexec{e_1}{\tcprod{C}{\grt_1}}{\psi}{k_1}{t_1}{\Phi_1} \\
  \freshCost{k_2,t_2} \\
  \Delta; k_2, t_2, \psi, \psi_a; \Phi \wedge C;   x :\grt_1,  \Omega  \chexec{ e_2}{\grt_2}{k_2}{t_2}{\Phi_2} \\
  \Phi_2' = {\cimpl{C}{\cand{\Phi_2}{\cand{\ceq{k}{(k_1+k_2)}}{\ceq{(t_1+t_2)}{t}}}}}
}
{
  \uctx  \chexec{\clet e_1 \eas x \ein e_2}{\grt_2}{k}{t}{\cexistsS{(\psi)}{(\cand{\Phi_1}{\cexists{k_2,t_2}{\scost}{\Phi_2'}})}}
} ~\textbf{alg-u-c-andE$\downarrow$}
}


\newcommand{\chRcandElim}
{
\inferrule
{
  \uctx \infdiff{e_1}{e_1'}{\tcprod{C}{\tau_1}}{\psi}{t_1}{\Phi_1} \\
  \freshCost{t_2} \\
  \Delta; t_2, \psi, \psi_a; \Phi \wedge C;   x :\tau_1,  \Omega  \chdiff{e_2}{e_2'}{\tau_2}{t_2}{\Phi_2} \\
  \Phi_2' = {\cimpl{C}{\cand{\Phi_2}{\ceq{(t_1+t_2)}{t}}}}
}
{
  \uctx  \chdiff{\clet e_1 \eas x \ein e_2}{\clet e_1' \eas x \ein e_2'}{\tau_2}{t}{\cexistsS{(\psi)}{(\cand{\Phi_1}{\cexists{t_2}{\scost}{\Phi_2'}})}}
} ~\textbf{alg-r-c-andE$\downarrow$}
}



\newcommand{\chsplit}
{
\inferrule{
  \Delta; \psi_a; C \wedge \Phi_a; \Omega \chexec{e_1}{\grt}{k}{t}{\Phi_1}\\\\
  \Delta; \psi_a; \neg C \wedge \Phi_a; \Omega \chexec{e_2}{\grt}{k}{t}{\Phi_2}\\ 
   \Delta\wfcs{C}
}
{ 
  \uctx \chexec{\esplit (e_1, e_2) \ewith C}{\grt}{k}{t}{\cand{\cimpl{C}{\Phi_1}}{\cimpl{\neg C}{\Phi_2}}}
} ~\textbf{alg-u-split$\downarrow$}
}



\newcommand{\chRsplit}
{
\inferrule{
  \Delta; \psi_a; C \wedge \Phi_a; \Gamma \chdiff{e_1}{e_1'}{\tau}{t}{\Phi_1}\\\\
  \Delta; \psi_a; \neg C \wedge \Phi_a; \Gamma \chdiff{e_2}{e_2'}{\tau}{t}{\Phi_2}\\
  \Delta  \wfcs{C}
}
{ 
  \bctx \chdiff{\esplit (e_1, e_2) \ewith C}{\esplit (e_1', e_2') \ewith C}{\tau}{t}{\cand{\cimpl{C}{\Phi_1}}{\cimpl{\neg C}{\Phi_2}}}
} ~\textbf{alg-r-split$\downarrow$}
}


\newcommand{\chcontra}
{
\inferrule{
  \Delta; \psi_a; \Phi_a \sat \bot
}
{ 
  \bctx \chexec{\econtra e}{\grt}{k}{t}{\ctrue}
}~\textbf{alg-u-contra$\downarrow$}
}


\newcommand{\chRcontra}
{
\inferrule{
  \Delta; \psi_a; \Phi_a \sat \bot
}
{ 
  \bctx \chdiff{\econtra e}{\econtra e'}{\tau}{t}{\ctrue}
} ~\textbf{alg-r-contra$\downarrow$}
}




\newcommand{\chRletMax}
{
  \inferrule{
  \Delta; \psi_a; \Phi_a; \trm{\Gamma}{1} \infexec{e_1}{\grt_1}{\psi}{k_1}{t_1}{\Phi_1} \\
  \freshCost{t_2}\\
  \Delta; t_2, \psi, \psi_a; \Phi_a; x: \tchs{\grt_1}, \Gamma \chdiff{e_2}{e}{\tau_2}{t_2}{\Phi_2}
}
{ \bctx \chdiff{ \elet x = e_1 \ein e_2}{e}{\tau_2}{t}{\cexistsS{(\psi)}{(\cand{\Phi_1}{\cexists{t_2}{\scost}{\cand{\Phi_2}{\ceq{t_1+t_2+\klet}{t}}}})}}
}~\textbf{alg-r-let-e$\downarrow$}
}

\newcommand{\chRletMaxSym}
{
  \inferrule{
  \Delta; \psi_a; \Phi_a; \trm{\Gamma}{2} \infexec{e_1}{\grt_1}{\psi}{k_1}{t_1}{\Phi_1} \\
  \freshCost{t_2}\\
  \Delta; t_2, \psi, \psi_a; \Phi_a; x: \tchs{\grt_1}, \Gamma \chdiff{e}{e_2}{\tau_2}{t_2}{\Phi_2}
}
{ \bctx \chdiff{e}{ \elet x = e_1 \ein e_2}{\tau_2}{t}{\cexistsS{(\psi)}{(\cand{\Phi_1}{\cexists{t_2}{\scost}{\cand{\Phi_2}{\ceq{t_2-k_1-\klet}{t}}}})}}
}~\textbf{alg-r-e-let$\downarrow$}
}



\newcommand{\chRecase}
{  \inferrule{
    \Delta; \psi_a; \Phi_a; \trm{\Gamma}{2}  \infexec{e}{\grt_1 + \grt_2}{\psi}{k_1}{t_1}{\Phi_1} \\
    \freshCost{t_2}\\
    \Delta; \psi_a; \Phi_a; x: \tchs{\grt_1}, \Gamma \chdiff{e_1}{e'}{\tau}{t_2}{\Phi_2}\\
    \Delta; \psi_a; \Phi_a; y: \tchs{\grt_2}, \Gamma \chdiff{e_2}{e'}{\tau}{t_2}{\Phi_3}
  }{\bctx \chdiff{\ecase(e, x.e_1, y.e_2)}{e'}{\tau}{t}{\cexistsS{(\phi)}{\cand{\Phi_1}{(\cexists{t_2}{\scost}{\cand{\Phi_2}{\ceq{t_1+t_2+\kcase}{t}}})}}}
  }~\textbf{alg-r-case-e$\downarrow^-$}
}


\newcommand{\chRecaseSym}
{  \inferrule{
    \Delta; \psi_a; \Phi_a; \trm{\Gamma}{2}  \infexec{e'}{\grt_1 + \grt_2}{\psi}{k_1}{t_1}{\Phi_1} \\
    \freshCost{t_2}\\
    \Delta; \psi_a; \Phi_a; x: \tchs{\grt_1}, \Gamma \chdiff{e}{e_1'}{\tau}{t_2}{\Phi_2}\\
    \Delta; \psi_a; \Phi_a; y: \tchs{\grt_2}, \Gamma \chdiff{e}{e_2'}{\tau}{t_2}{\Phi_3}
  }{\bctx \chdiff{e}{\ecase(e', x.e_1', y.e_2')}{\tau}{t}{\cexistsS{(\phi)}{\cand{\Phi_1}{(\cexists{t_2}{\scost}{\cand{\Phi_2}{\ceq{t_2-k_1-\kcase}{t}}})}}}
  }~\textbf{alg-r-e-case$\downarrow^-$}
}

\newcommand{\chRappfun}
{
  \inferrule{
    \Delta; \psi_a; \Phi; \trm{\Gamma}{1} \infexec{e_1}{\grt_1 \uarr{k_e}{t_e} \grt_2}{\psi}{k_1}{t_1}{\Phi_1}
    \\    \freshCost{t_2} \\
    \Delta; t_2, \psi, \psi_a; \Phi_a; \Gamma \chdiff{e_2}{e_2'}{\tch{\grt_1}{\grt_2'}}{t_2}{\Phi_2} \\
    \Delta; \psi, \psi_a; \Phi_a \jalgasubtype{\grt_2}{\grt}{\Phi_3} 
}
{\bctx \chdiff{e_1 \eapp e_2}{e_2'}{\tch{\grt}{\grt_2'}}{t}{\cexistsS{(\psi)}{\cand{\Phi_1}{\cand{(\cexists{t_2}{\scost}{\cand{\Phi_2}{\ceq{t_1+t_2+t_e+\kapp}{t}}})}{\Phi_3}}}}
}~\textbf{alg-r-app-e$\downarrow$} 
}



\newcommand{\chRappfunSym}
{
  \inferrule{
    \Delta; \psi_a; \Phi; \trm{\Gamma}{2} \infexec{e_1'}{\grt_1' \uarr{k_e}{t_e} \grt_2'}{\psi}{k_1}{t_1}{\Phi_1}
    \\
    \freshCost{t_2} \\
    \Delta; t_2, \psi, \psi_a; \Phi_a; \Gamma \chdiff{e_2}{e_2'}{\tch{\grt}{\grt_1'}}{t_2}{\Phi_2} \\
    \Delta; \psi, \psi_a; \Phi_a \jalgasubtype{\grt_2'}{\grt'}{\Phi_3} 
}
{\bctx \chdiff{e_2}{e_1' \eapp e_2'}{\tch{\grt}{\grt'}}{t}{\cexistsS{(\psi)}{\cand{\Phi_1}{\cand{(\cexists{t_2}{\scost}{\cand{\Phi_2}{\ceq{t_2-k_1-k_e+\kapp}{t}}})}{\Phi_3}}}} 
}~\textbf{alg-r-e-app$\downarrow$}
}


%%% Local Variables:
%%% mode: latex
%%% TeX-master: "main"
%%% End:
