# Supplementary material for: Bidirectional Type Checking for Relational Properties
Source: arXiv:1812.05067 source file (2018-12-12)
Supplement: Supplementary file 19 [file alg-typing-rules.tex]

\begin{figure*}
  \fbox{$\Delta; \psi_a; \Phi_a; \Gamma
    \chdiff{e_1}{e_2}{\tau}{t}{\Phi}$} ~ Under the existential
  variable context $\psi_a$ and the assumption $\Phi_a$,
  $e_1 \rdiff e_2$ checks against the input type $\tau$
  and the difference cost $t$. Finally, it generates the constraint $\Phi$.\\\\
  \fbox{$\Delta; \psi_a; \Phi_a;  \Gamma \infdiff{e_1}{e_2}{\tau}{\psi}{t}{\Phi}$} ~ Under the existential variable context $\psi_a$ and the assumption $\Phi_a$,  $e_1 \rdiff e_2$ synthesizes the output type $\tau$ and the relative cost $t$ where all the newly generated existential variables are defined in $\psi$. Finally, it generates the constraint $\Phi$. \\\\
  \fbox{$\Delta; \psi_a; \Phi_a; \Omega \chexec{e}{\grt}{k}{t}{\Phi}$}
  ~ Under the existential variable context $\psi_a$ and the assumption
  $\Phi_a$, $e$ checks against the unary input type $\grt$ and the minimum execution cost $k$ and maximum execution cost $t$. Finally, it generates the constraint $\Phi$.\\\\
  \fbox{$\Delta; \psi_a; \Phi_a; \Omega
    \infexec{e}{\grt}{\psi}{k}{t}{\Phi}$} ~Under the existential
  variable context $\psi_a$ and the assumption $\Phi_a$, $e$
  synthesizes the unary output type $\grt$, the minimum execution cost
  $k$ and maximum execution cost $t$, where all the newly generated
  existential variables are defined in $\psi$. Finally, it generates
  the constraint $\Phi$.

\vspace{5mm}
\raggedright



\framebox{$\eswitch e$}
\begin{mathpar}
  \infRswitch
  \and
  \chRswitch
\end{mathpar}

\framebox{$\enoch e$}
\begin{mathpar}
  \chRnochange
\end{mathpar}
  
\framebox{$\eder e$}
\begin{mathpar}
  \infRder
  % \and
  % \chRder
\end{mathpar}

\framebox{Constant Integers $\kw{n}$ and unit}
\begin{mathpar}
  \infconst
  \and
  \infRconst
  \and
  \infunit
  \and
  \infRunit
\end{mathpar}



\framebox{Variables $x$}
\begin{mathpar}
\infvar
\and
\infRvar
\end{mathpar}


\caption{Algorithmic typing rules (part 1)}
\label{fig:alg-typing-rules1}
\end{figure*}



\begin{figure*}

\framebox{$\einl e $ }
\begin{mathpar}
  \chinl
  \and
  \chRinl
\end{mathpar}


\framebox{$\einr e $ }
\begin{mathpar}
  \chinr
  \and
  \chRinr
\end{mathpar}

\framebox{$\ecase(e,x.e_1,y.e_2)$}
\begin{mathpar}
 \chcase
 \and
 \chRcase
\end{mathpar}



\framebox{$\efix f(x).e$}
\begin{mathpar}
  \chfix
  \and
  \chRfix
  \and
  \chRfixBox
\end{mathpar}


\caption{Algorithmic typing rules (part 2)}
\label{fig:alg-typing-rules2}
\end{figure*}



\begin{figure*}

  \framebox{$e_1 \eapp e_2$}
  \begin{mathpar}
    \infapp
    \and
    \infRapp
  \end{mathpar}
  
  
  \framebox{ $(e_1, e_2)$}
  \begin{mathpar}
    \chpair
    \and
    \chRpair
  \end{mathpar}
  
  
  \framebox{ $\eleft(e)$}
  \begin{mathpar}
    \chfst
    \and
    \chRfst
  \end{mathpar}
  
  \framebox{$\enil$}
  \begin{mathpar}
    \chnil
    \and
    \chRnil
  \end{mathpar}
  
  \framebox{$\econs(e_1,e_2)$}
  \begin{mathpar}
    \chcons
    \and
    \chRcons
    \and
    \chRconsbox
  \end{mathpar}

% \framebox{ $\eright(e)$}
% \begin{mathpar}
% \chsnd
% \and
% \chRsnd
% \end{mathpar}



\caption{Algorithmic typing rules (part 3)}
\label{fig:alg-typing-rules3}
\end{figure*}





\begin{figure*} 
\framebox{$\ecase e \eof \enil \rightarrow e_1 ~|~ h::tl \rightarrow e_2$}
\begin{mathpar}
  \chcaseL
  \and
  \chRcaseL
\end{mathpar}


\framebox{$\eLam i. e$}
\begin{mathpar} 
  \chiLam
  \and
  \chRiLam
\end{mathpar}


\framebox{$e \,[I]$}
\begin{mathpar}
  \infiApp
  \and
  \infRiApp
\end{mathpar}

\framebox{$\epack e \ewith I$}
\begin{mathpar}
  \chpack
  \and
  \chRpack
\end{mathpar}

\caption{Algorithmic typing rules (part 4)}
\label{fig:alg-typing-rules4}
\end{figure*}


\begin{figure*}


  \framebox{$\eunpack e \eas (x, i) \ein e'$}
  \begin{mathpar}
    \chunpack
  \and
  \chRunpack
\end{mathpar}


\framebox{$\zeta \eapp e$}
\begin{mathpar}
  \infprimapp
  % 
  \and
  % 
  \infRprimapp
\end{mathpar}


\framebox{$\tcprod{C}{\cdot}$ intro}
\begin{mathpar}
  \chcandIntro
  \and
  \chRcandIntro
\end{mathpar}

\framebox{$\clet e_1 \eas x \ein e_2$}
\begin{mathpar}
  \chcandElim
  \and
  \chRcandElim
\end{mathpar}

\caption{Algorithmic typing rules (part 5)}
\label{fig:alg-typing-rules5}
\end{figure*}





\begin{figure*}

  \framebox{$\tcimpl{C}{\cdot}$ intro}
  \begin{mathpar}
    \chcimplIntro
    \and
    \chRcimplIntro
  \end{mathpar}
  
  \framebox{$\ecelim e$}
  \begin{mathpar}
    \infcimplElim
    \and
    \infRcimplElim
  \end{mathpar}
  

  \framebox{$\elet x = e_1 \ein e_2$}
  \begin{mathpar}
    \chlet
    % 
    \and
    % 
    \chRlet
  \end{mathpar}
  

  \framebox{$\esplit e$}
  \begin{mathpar}
    \chsplit
    \and
    \chRsplit
  \end{mathpar}

  \framebox{$\econtra e$}
  \begin{mathpar}
    \chcontra
    \and
    \chRcontra
  \end{mathpar}


  \caption{Algorithmic typing rules (part 6)}
\label{fig:alg-typing-rules6}
\end{figure*}

\begin{figure*}
  


\framebox{$\uparrow \downarrow$}
\begin{mathpar}
\chupdown
%
\and
%
\chRupdown
\end{mathpar}


\framebox{$\eanno{e}{\grt}{k}{t}$}

\begin{mathpar}
\infanno
\end{mathpar}


\framebox{$\eannobi{e}{\tau}{t}$}

\begin{mathpar}
\infRanno
\end{mathpar}



\framebox{Heuristic typing}
\begin{mathpar}
  \chRletMax
  \and
  \chRletMaxSym
  \and
  \chRappfun
  \and
  \chRappfunSym
  \and
  \chRecase 
  \and
  \chRecaseSym
\end{mathpar}

\caption{Algorithmic typing rules (part 7)}
\label{fig:alg-typing-rulesy}
\end{figure*}

%%% Local Variables:
%%% mode: latex
%%% TeX-master: "main"
%%% End: 
