# Supplementary material for: Bidirectional Type Checking for Relational Properties
Source: arXiv:1812.05067 source file (2018-12-12)
Supplement: Supplementary file 20 [file alg-unary-subtyping-reflexivity.tex]

\begin{lem}[Reflexivity of Unary Algorithmic Subtyping] \label{lem:alg-unary-subtyping-refl}
   $\Delta ; \Phi_a \jalgasubtype{\grt}{\grt}{\Phi}$ and $\Delta; \Phi_a \sat \Phi$.
\end{lem}

\begin{proof}
  By induction on the unary type.
\end{proof}

%%% Local Variables:
%%% mode: latex
%%% TeX-master: "main"
%%% End:
