# Supplementary material for: Bidirectional Type Checking for Relational Properties
Source: arXiv:1812.05067 source file (2018-12-12)
Supplement: Supplementary file 21 [file alg-unary-subtyping-transitivity.tex]

\begin{lem}[Transitivity of Unary Algorithmic Subtyping] \label{lem:alg-unary-subtyping-trans}
  If $\Delta ; \Phi_a \jalgasubtype{\grt_1}{\grt_2}{\Phi_1}$ and $\Delta ; \Phi_a \jalgasubtype{\grt_2}{\grt_3}{\Phi_2}$ and $\Delta; \Phi_a \sat \cand{\Phi_1}{\Phi_2}$, then $\Delta ; \Phi_a \jalgasubtype{\grt_1}{\grt_3}{\Phi_3}$ for some $\Phi_3$ such that $\Delta; \Phi_a \sat \Phi_3$.
\end{lem}

\begin{proof}
  By induction on the first subtyping derivation.
\end{proof}

%%% Local Variables:
%%% mode: latex
%%% TeX-master: "main"
%%% End:
