# Supplementary material for: Bidirectional Type Checking for Relational Properties
Source: arXiv:1812.05067 source file (2018-12-12)
Supplement: Supplementary file 22 [file completeness-relcostM.tex]

\begin{thm} [Completeness of \tnamemin] \label{thm:relcost-min-completeness}
  The following holds.
  \begin{enumerate}
  \item If $\Delta; \Phi; \Omega \jtype{k}{t}{e}{\grt}$ then,
    $\exists\, e^*$ such that
    $\Delta; \Phi; \Omega \jelabun{k}{t}{e}{e^*}{\grt}$.
    \item If $\Delta; \Phi; \Gamma \jtypediff{t}{e_1}{e_2}{\tau}$ then,
    $\exists\, e_1^*$ and $\exists \,e_2^*$ such that
    $\Delta; \Phi; \Gamma \jelab{t}{e_1}{e_2}{e_1^*}{e_2^*}{\tau}$.

  \end{enumerate}
\end{thm}

\begin{proof}
  Proof is by simultaneous induction on the typing derivations. The
  proof follows from the embedding rules presented in Figures
  \ref{fig:elab-rules1}-\ref{fig:elab-rules3}. We show a few
  representative cases.


\begin{spacing}{1.3}
  \hspace{-1cm} \textbf{Proof of \Cref{thm:relcost-min-completeness}.1:} \\
\begin{mainitem} 
    %%%%%%%%%%%%%%%%%%%%%%%%%%%%%%%%%%%%%%%%%%%%%%%%%%%%%%%%%%%%%%%%%%%%%%% 
    \caseL{$\tysubsum[(\star)][(\diam)][(\dagg)][\dagg\dagg]$} 
    By \Cref{thm:relcost-min-completeness}.1 on $(\star)$, we get $\exists\, e^*$ such that $\Delta; \Phi; \Omega \jelabun{k}{t}{e}{e^*}{\grt} ~~(\star\star)$. \\
    By \textbf{e-u-$\sqsubseteq$} rule using $(\star\star)$, $(\diam)$,  $(\dagg)$ and $(\dagg\dagg)$, we conclude as follows\\ $\elsubsum$

  \end{mainitem}

\end{spacing}
  
\begin{spacing}{1.3}
  \hspace{-1cm} \textbf{Proof of \Cref{thm:relcost-min-completeness}.2:} \\

  \begin{mainitem}
    %%%%%%%%%%%%%%%%%%%%%%%%%%%%%%%%%%%%%%%%%%%%%%%%%%%%%%%%%%%%%%%%%%%%%%%
    \caseL{\tyswitch[(\star)][(\diam)]}
    By \Cref{thm:relcost-min-completeness}.1 on $(\star)$, we get $\exists\, e_1^*$ such that $\Delta; \Phi; \Omega \jelabcu{k_1}{t_1}{e_1}{\grt_1} ~~(\star\star)$. \\
    By \Cref{thm:relcost-min-completeness}.1 on $(\diam)$, we get $\exists\, e_2^*$ such that $\Delta; \Phi; \Omega \jelabcu{k_2}{t_2}{e_2}{\grt_2} ~~(\diam\diam)$. \\
    By \textbf{e-switch} embedding rule using $(\star\star)$ and $(\diam\diam)$, we can conclude as follows:\\
    $\elswitch[(\star\star)][(\diam\diam)]$. \\
  
    
    %%%%%%%%%%%%%%%%%%%%%%%%%%%%%%%%%%%%%%%%%%%%%%%%%%%%%%%%%%%%%%%%%%%%%%%
    \caseL{\tynochange[(\star)][(\diam)]}
    By \Cref{thm:relcost-min-completeness}.2 on $(\star)$, we get $\exists\, e^*$ such that $\Delta; \Phi; \Gamma \jelab{t}{e}{e}{e^*}{e^*}{\tau} ~~(\dagg)$. \\
    By \lemref{lem:sub-elab} on $(\diam)$, we get $\exists e_i= \ecoerce{\Gamma(x_i)}{\tbox{(\Gamma(x_i)}}$ for all $x_i \in dom(\Gamma)~~(\dagg\dagg)$.\\
    By \textbf{e-nochange} embedding rule using $(\dagg)$ and $(\dagg\dagg )$, we can conclude as follows:\\
    $\elnochange[(\dagg)][(\dagg\dagg)]$. 
    
    %%%%%%%%%%%%%%%%%%%%%%%%%%%%%%%%%%%%%%%%%%%%%%%%%%%%%%%%%%%%%%%%%%%%%%% 
    \caseL{\tyrcaseL[(\star)][(\diam)][(\dagg)][(\spadesuit)]}
    By \Cref{thm:relcost-min-completeness}.2 on $(\star)$, we get $\exists\, e^*$  and $\exists\, e'^*$ s.t. $\Delta; \Phi; \Gamma \jelab{t}{e}{e'}{e^*}{e'^*}{\tlist{n}{\alpha}{\tau}} ~~(\star\star)$. \\
   By \Cref{thm:relcost-min-completeness}.2 on $(\diam)$, we get $\exists\, e_1^*$  and $\exists\, e_1'^*$ s.t. $\Delta; \ceqz{n} \wedge \Phi; \Gamma \jelab{t}{e_1}{e_1'}{e_1^*}{e_1'^*}{\tau'} ~~(\diam\diam)$. \\
   By \Cref{thm:relcost-min-completeness}.2 on $(\dagg)$, we get $\exists\, e_2^*$  and $\exists\, e_2'^*$ s.t. \\$\sorted{i}, \Delta; \ceq{n}{i+1} \wedge \Phi; h :\tbox{\tau}, tl : \tlist{i}{\alpha}{\tau}, \Gamma \jelab{t}{e_2}{e_2'}{e_2^*}{e_2'^*}{\tau'} ~(\dagg\dagg)$. \\
   By \Cref{thm:relcost-min-completeness}.2 on $(\spadesuit)$, we get $\exists\, e_2^{**}$  and $\exists\, e_2'^{**}$ s.t.\\ $\sorted{i}, \sorted{\beta}, \Delta; \ceq{n}{i+1} \wedge \ceq{\alpha}{\beta+1} \wedge \Phi; h :\tau, tl : \tlist{i}{\beta}{\tau}, \Gamma \jelab{t}{e_2}{e_2'}{e_2^{**}}{e_2'^{**}}{\tau'} ~(\spadesuit\spadesuit)$. \\
    
    By \textbf{e-caseL} embedding rule using $(\star\star)$, $(\diam\diam)$, and $(\spadesuit\spadesuit)$, we can conclude as follows\\
    $\elrcaseL$


    %%%%%%%%%%%%%%%%%%%%%%%%%%%%%%%%%%%%%%%%%%%%%%%%%%%%%%%%%%%%%%%%%%%%%%%
    \caseL{\tyrfixNC[(\star)][(\diam)]}
    By \Cref{thm:relcost-min-completeness}.2 on $(\star)$, we get $\exists\, e^*$ such that $\Delta; \Phi; x: \tau_1, f: \tbox{(\tau_1 \tarrd{t} \tau_2)}, \Gamma \jelab{t}{e}{e}{e^*}{e^*}{\tau_2} ~~(\star\star)$. \\
    By \lemref{lem:sub-elab} on $(\diam)$, we get $\exists e_i= \ecoerce{\Gamma(x_i)}{\tbox{(\Gamma(x_i)}}$ for all $x_i \in dom(\Gamma)~~(\diam\diam)$.\\
    
    By \textbf{e-fixNC} embedding rule using $(\star\star)$ and $(\diam\diam )$, we can conclude as follows:\\
    $\elrfixNC$. 


    %%%%%%%%%%%%%%%%%%%%%%%%%%%%%%%%%%%%%%%%%%%%%%%%%%%%%%%%%%%%%%%%%%%%%%% 
    \caseL{\tyriLam[(\star)]}
    By \Cref{thm:relcost-min-completeness}.2 on $(\star)$, we get $\exists\, e^*$ and $\exists\, e'^*$ such that $\sorted{i}, \Delta; \Phi; \Gamma \jelab{t}{e}{e'}{e^*}{e'^*}{\tau} ~~(\star\star)$. \\
    By \textbf{e-iLam} embedding rule using $(\star\star)$ , we can conclude as follows:\\
    $\elriLam$. 

    %%%%%%%%%%%%%%%%%%%%%%%%%%%%%%%%%%%%%%%%%%%%%%%%%%%%%%%%%%%%%%%%%%%%%%% 
    \caseL{\tyriApp[(\star)][(\diam)]}
    By \Cref{thm:relcost-min-completeness}.2 on $(\star)$, we get $\exists\, e^*$ such that $\Delta; \Phi; \Gamma \jelab{t}{e}{e'}{e^*}{e'^*}{\tforall{i}{t'} \tau} ~~(\star\star)$. \\
    By \textbf{e-iApp} embedding rule using $(\star\star)$ and $(\diam)$, we can conclude as follows:\\
    $\elriApp$. 

    %%%%%%%%%%%%%%%%%%%%%%%%%%%%%%%%%%%%%%%%%%%%%%%%%%%%%%%%%%%%%%%%%%%%%%% 
    \caseL{\tyrpack[(\star)][(\diam)]}
    By \Cref{thm:relcost-min-completeness}.2 on $(\star)$, we get $\exists\, e^*$ and $\exists\, e'^*$ such that $\Delta; \Phi; \Gamma \jelab{t}{e}{e'}{e^*}{e'^*}{\tau\{I/i\}} ~~(\star\star)$. \\
    By \textbf{e-pack} embedding rule using $(\star\star)$ and $(\diam)$ , we can conclude as follows:\\
    $\elrpack$. 

    %%%%%%%%%%%%%%%%%%%%%%%%%%%%%%%%%%%%%%%%%%%%%%%%%%%%%%%%%%%%%%%%%%%%%%% 
    \caseL{\tyrunpackD[(\star)][(\diam)]}
    By \Cref{thm:relcost-min-completeness}.2 on $(\star)$, we get $\exists\, e_1^*$ and $\exists\, e_1'^*$ such that $\Delta; \Phi; \Gamma \jelab{t}{e_1}{e_1'}{e_1^*}{e_1'^*}{\texists{i} \tau_1} ~~(\star\star)$. \\
    By \Cref{thm:relcost-min-completeness}.2 on $(\diam)$, we get $\exists\, e_2^*$ and $\exists\, e_2'^*$ such that $\sorted{i}, \Delta; \Phi; x: \tau_1, \Gamma \jelab{t}{e_2}{e_2'}{e_2^*}{e_2'^*}{\tau_2} ~~(\diam\diam)$. \\
    By \textbf{e-unpack} embedding rule using $(\star\star)$ and $(\diam\diam)$ , we can conclude as follows:\\
    $\elrunpack$. 

    %%%%%%%%%%%%%%%%%%%%%%%%%%%%%%%%%%%%%%%%%%%%%%%%%%%%%%%%%%%%%%%%%%%%%%% 
    \caseL{$\tyrsubsum[(\star)][(\diam)][\dagg]$}  
    By \Cref{thm:relcost-min-completeness}.2 on $(\star)$, we get $\exists\, e_1^*,e_2^*$ such that $\Delta; \Phi; \Gamma \jelabc{t}{e_1}{e_2}{\tau} ~~(\star\star)$. \\
    By \Cref{lem:sub-elab} on $(\diam)$, we can show that $\exists e' = \ecoerce{\tau}{\tau'}~~(\diam\diam)$.\\
    By \textbf{e-r-$\sqsubseteq$} rule using $(\star\star)$, $(\diam\diam)$ and $(\dagg)$, we conclude as follows\\ $\elrsubsum$


\end{mainitem}


\end{spacing}




\end{proof}
%%% Local Variables:
%%% mode: latex
%%% TeX-master: "main"
%%% End:
