# Supplementary material for: Bidirectional Type Checking for Relational Properties
Source: arXiv:1812.05067 source file (2018-12-12)
Supplement: Supplementary file 23 [file constraint-gen.tex]

\begin{figure*}
  \centering
  \begin{smathpar}
\inferrule
{
\strut
}
{
  \subsat{\Delta}{[]}{\cdot}
}
%
\and
%
\inferrule
{
\Delta \vdash I :: \sort\\
\subsat{\Delta}{\theta}{\psi}
}
{
  \subsat{\Delta}{\theta[M \mapsto I]}{M::\sort,\psi}
}
%
\end{smathpar}

\caption{Sorting of Substitutions}
\label{fig:wf-subst}
\end{figure*}

%%% Local Variables: 
%%% mode: latex
%%% TeX-master: "main"
%%% End: 
