# Supplementary material for: Bidirectional Type Checking for Relational Properties
Source: arXiv:1812.05067 source file (2018-12-12)
Supplement: Supplementary file 24 [file elaboration-rules-defs.tex]

\newcommandx{\elswitch}[2][1=,2=]
{
    \inferrule{
    \Delta; \Phi_a; \trm{\Gamma}{1} \jelabun{k_1}{t_1}{e_1}{e_1^*}{\grt_1}~~#1\\
    \Delta; \Phi_a; \trm{\Gamma}{2} \jelabun{k_2}{t_2}{e_2}{e_2^*}{\grt_2}~~#2
    } {\ctx \jelab{t_1-k_2}{e_1}{e_2}{\eswitch e_1^*}{\eswitch e_2^*}{\tch{\grt_1}{\grt_2}}}~\textbf{e-switch}
}

\newcommandx{\elnochange}[2][1=,2=]
{
  \inferrule
  {
    \Delta; \Phi_a; \Gamma \jelab{t}{e}{e}{e^*}{e^*}{\tau}~~#1 \\
    \forall x_i \in dom(\Gamma), ~~e_i = \ecoerce{\Gamma(x_i)}{\tbox{\Gamma(x_i)}}~~#2
  }
  {
    \Delta; \Phi_a; \Gamma, \Gamma' \jelab{0}{e}{e}{\elet \overline{ y_i = e_i \eapp x_i} \ein \enoch e^* [\overline{y_i/x_i}]}{\elet \overline{ y_i = e_i \eapp x_i} \ein \enoch e^* [\overline{y_i/x_i}]}{\tbox{\tau}}
  } ~\textbf{e-nochange}
}

\newcommand{\elconst}
{
  \inferrule
  {
    \strut
  }
  {
    \octx \jelabun{0}{0}{\econst}{\econst}{\tint}
  }~\textbf{e-u-const}
}

\newcommand{\elrconst}
{
  \inferrule
  {
    \strut
  }
  {
    \ctx \jelabsame{0}{\econst}{\econst}{\trint}
  }~\textbf{e-r-const}
}


\newcommand{\elunit}
{
  \inferrule
  {
    \strut
  }
  {
    \octx \jelabun{0}{0}{\eunit}{\eunit}{\tunit}
  }~\textbf{e-u-unit}
}

\newcommand{\elrunit}
{
  \inferrule
  {
    \strut
  }
  {
    \ctx \jelabsame{0}{\eunit}{\eunit}{\trunit}
  }~\textbf{e-r-unit}
}

\newcommand{\elvar}{
  \inferrule{\Omega(x) = \grt}{\octx \jelabun{0}{0}{x}{x}{\grt}}~\textbf{e-u-var}
}

\newcommand{\elrvar}{
  \inferrule{\Gamma(x) = \tau}{\ctx \jelabsame{0}{x}{x}{\tau}}~\textbf{e-r-var}
}

 \newcommand{\elinl}
{  \inferrule
  {
    \octx  \jelabcu{k}{t}{e}{\grt_1}\\
    {
     \ifextra
     \Delta; \Phi_a \wfty{\grt_2}
     \fi
   }
  }
  { \octx  \jelabcu{k}{t}{\einl e}{\grt_1 + \grt_2}
  }~\textbf{e-u-inl}
}

\newcommand{\elrinl}
{  \inferrule
  {
    \ctx  \jelabc{t}{e_1}{e_2}{\tau_1}\\
    {
     \ifextra
     \Delta; \Phi_a \wfty{\tau_2}
     \fi
   }
  }
  { \ctx  \jelabc{t}{\einl e_1}{\einl e_2}{\tau_1 + \tau_2}
  }~\textbf{e-r-inl}
}

\newcommand{\elinr}
{  \inferrule
  {
    \octx  \jelabcu{k}{t}{e}{\grt_2}\\
    {
     \ifextra
     \Delta; \Phi_a \wfty{\grt_1}
     \fi
   }
  }
  { \octx  \jelabcu{k}{t}{\einr e}{\grt_1 + \grt_2}
  }~\textbf{e-u-inr}
}

\newcommand{\elrinr}
{  \inferrule
  {
    \ctx  \jelabc{t}{e_1}{e_2}{\tau_2}\\
    {
     \ifextra
     \Delta; \Phi_a \wfty{\tau_1}
     \fi
   }
  }
  { \ctx  \jelabc{t}{\einr e_1}{\einl e_2}{\tau_1 + \tau_2}
  }~\textbf{e-r-inr}
}

\newcommand{\elcase}
{  \inferrule{
    \octx \jelabcu{k}{t}{e}{\grt_1 + \grt_2}\\
    \Delta; \Phi_a; x: \grt_1, \Omega \jelabcu{k'}{t'}{e_1}{\grt}\\
    \Delta; \Phi_a; y: \grt_2, \Omega  \jelabcu{k'}{t'}{e_2}{\grt}
  }{\octx \jelabun{k+k'+\kcase}{t+t'+\kcase}{\ecase(e, x.e_1, y.e_2)}{\ecase(e^*, x.e_1^*, y.e_2^*)}{\grt}}
  ~\textbf{e-u-case}
} 
%


\newcommand{\elrcase}
{  \inferrule{
    \ctx \jelabc{t}{e}{e'}{\tau_1 + \tau_2}\\
    \Delta; \Phi_a; x: \tau_1, \Gamma \jelabc{t'}{e_1}{e_1'}{\tau}\\
    \Delta; \Phi_a; y: \tau_2, \Gamma  \jelabc{t'}{e_2}{e_2'}{\tau} \\
    e_1^{**} =  \ecase(e^*, x.e_1^*, y.e_2^*) \\
    e_2^{**} = \ecase(e', x.e_1'^*, y.e_2'^*)
}{\ctx \jelab{t+t'}{
    \ecase(e, x.e_1, y.e_2)}{\ecase(e', x.e_1', y.e_2')}{e_1^{**}}{e_2^{**}}{\tau}}~\textbf{e-r-case}}
%


\newcommand{\elfix}
{  \inferrule{
       {\ifextra
       \Delta; \Phi_a \awfty{\grt_1 \uarr{k}{t} \grt_2}  
       \fi} \\
       \Delta; \Phi_a;  x: \grt_1, f : \grt_1 \uarr{k}{t} \grt_2, \Omega  
       \jelabcu{k}{t}{e}{\grt_2}
     }       
     {\octx \jelabcu{0}{0}{ \efix f(x).e}{\grt_1 \uarr{k}{t} \grt_2}}~\textbf{e-u-fix}
}
%


\newcommand{\elrfix}
{  \inferrule{
       {\ifextra
       \Delta; \Phi_a \wfty{\tau_1 \tarrd{t} \tau_2}  
       \fi} \\
       \Delta; \Phi_a;  x: \tau_1, f : \tau_1 \tarrd{t} \tau_2, \Gamma  
       \jelabc{t}{e_1}{e_2}{\tau_2}
     }       
     {\ctx \jelabc{0}{ \efix f(x).e_1}{\efix f(x).e_2}{
              \tau_1 \tarrd{t} \tau_2}}~\textbf{e-r-fix}
}
%

\newcommand{\elrfixNC}
{  \inferrule
  {
    {\ifextra \Delta; \Phi_a \wfty{\tau_1 \tarrd{t} \tau_2}
      \fi} \\
    \Delta; \Phi_a;  x: \tau_1, f : \tbox{(\tau_1 \tarrd{t} \tau_2)}, \Gamma \jelabc{t}{e}{e}{\tau_2} \\
    \forall x_i \in dom(\Gamma), ~~e_i = \ecoerce{\Gamma(x_i)}{\tbox{\Gamma(x_i)}} \\
    e^{**}= \elet \overline{ y_i = e_i \eapp x_i} \ein \efixNC f(x).e^*[\overline{y_i/x_i}]
  }
  {\ctx \jelab{0}{\efix f(x).e}{\efix f(x).e}{e^{**}}{e^{**}}{
              \tbox{(\tau_1 \tarrd{t} \tau_2)}}}~\textbf{e-r-fixNC}
} 


\newcommand{\elapp}
{\inferrule{\octx \jelabcu{k_1}{t_1}{e_1}{\grt_1}
  \uarr{k}{t} \grt_2 \\
  \octx \jelabcu{k_2}{t_2}{e_2}{\grt_1}
}
{\octx \jelabun{k_1+k_2+k +\kapp}{t_1+t_2+t+\kapp}{e_1 \eapp e_2}{e_1^* \eapp e_2^*}{\grt_2}}~\textbf{e-u-app}}


\newcommand{\elrapp}
{\inferrule{\ctx \jelabc{t_1}{e_1}{e_1'}{\tau_1}
  \tarrd{t} \tau_2 \\
  \ctx \jelabc{t_2}{ e_2}{e_2'}{\tau_1}
}
{\ctx \jelab{t_1+t_2+t}{e_1 \eapp e_2}{e_1' \eapp e_2'}{e_1^* \eapp e_2^*}{e_1'^* \eapp e_2'^*}{\tau_2}}~\textbf{e-r-app}}


\newcommand{\elprod}
{\inferrule{\octx \jelabcu{k_1}{t_1}{e_1}{\grt_1}\\
    \octx \jelabcu{k_2}{t_2}{ e_2}{\grt_2}}
{
  \octx 
  \jelabun{k_1+k_2}{t_1+t_2}{\la e_1, e_2 \ra}{\la e_1^*, e_2^* \ra}{\grt_1 \ttimes \grt_2}
}~\textbf{e-u-prod}
}

\newcommand{\elrprod}
{\inferrule{\ctx \jelabc{t_1}{e_1}{e_1'}{\tau_1}\\ \ctx
  \jelabc{t_2}{ e_2}{e_2'}{\tau_2}
}
{
  \ctx 
  \jelab{t_1+t_2}{\la e_1, e_2 \ra}{\la e_1' , e_2' \ra}{\la e_1^*, e_2^* \ra}{\la e_1'^* , e_2'^* \ra}{\tau_1 \ttimes \tau_2}
}~\textbf{e-r-prod}
}



\newcommand{\elproj}
{\inferrule{
    \octx \jelabc{k}{t}{e}{\grt_1 \ttimes\grt_2}
}
{\octx \jelabun{k}{t}{ \eleft(e)}{ \eleft(e^*)}{\grt_1}}~\textbf{e-u-proj1}
}

\newcommand{\elrproj}
{\inferrule{
    \ctx \jelabc{t}{e}{e'}{\tau_1 \ttimes\tau_2}
}
{\ctx \jelab{t}{ \eleft(e)}{\eleft(e')}{ \eleft(e^*)}{\eleft(e'^*)}{\tau_1}}~\textbf{e-r-proj1}
}


\newcommand{\elnil}
{  \inferrule
  {
    \Delta; \Phi_a \wfty{\grt}
  }
  { \octx \jelabun{0}{0}{\enil}{\enil}{\ulist{0}{\grt}}
  }~\textbf{e-u-nil}
}

\newcommand{\elrnil}
{  \inferrule
  {
    \Delta; \Phi_a \wfty{\tau}
  }
  { \ctx \jelab{0}{\enil}{\enil}{\enil}{\enil}{\tlist{0}{\alpha}{\tau}}
  }~\textbf{e-r-nil}
}



\newcommand{\elcons} 
{   \inferrule
  { \octx \jelabcu{t_1}{k_1}{e_1}{\grt} \\
    \octx \jelabcu{t_2}{k_2}{e_2}{\ulist{n}{\grt}}
  }
  { \octx \jelabun{k_1+k_2}{t_1+t_2}{ \econs(e_1,e_2) }{ \econsC(e_1^*,e_2^*)}{\ulist{n+1}{\grt}}}~\textbf{e-u-cons}
}

\newcommand{\elrcons} 
{   \inferrule
  { \ctx \jelabc{t_1}{e_1}{e_1'}{\tau} \\
    \ctx \jelabc{t_2}{e_2}{e_2'}{\tlist{n}{\alpha}{\tau}}
  }
  { \ctx \jelab{t_1+t_2}{ \econs(e_1,e_2) }{\econs(e_1',e_2')}{ \econsC(e_1^*,e_2^*)}{ \econsC(e_1'^*,e_2'^*)}{\tlist{n+1}{\alpha+1}{\tau}}}~\textbf{e-r-cons1}
}

\newcommand{\elrconsbox}
{   \inferrule
  { \ctx \jelabc{t_1}{e_1}{e_1'}{\tbox{\tau}} \\
    \ctx \jelabc{t_2}{e_2}{e_2'}{\tlist{n}{\alpha}{\tau}}}
  { \ctx \jelab{t_1+t_2}{ \econs(e_1,e_2) }{\econs(e_1',e_2')}{ \econsNC(e_1',e_2')}{ \econsNC(e_1^*,e_2^*)}{\tlist{n+1}{\alpha}{\tau}}}~\textbf{e-r-cons2}}


\newcommand{\elcaseL}
{ \inferrule
  {\octx \jelabcu{k}{t}{e}{\ulist{n}{\grt}}\\
   \Delta; \Phi_a \wedge n = 0  ;\Omega \jelabcu{k'}{t'}{e_1}{\grt'}\\
   i, \Delta; \Phi_a \wedge n = i+1;  h: \grt,
   tl : \ulist{i}{\grt}, \Omega \jelabcu{k'}{t'}{e_2}{\grt'}
   }
   {\octx \jelabun{k+k'+\kcaseL}{t+t'+\kcaseL}
     { \hspace{-1.5em}
       \begin{minipage}[c]{9em}
         ~ $\ecase e \eof \enil \rightarrow e_1$ \\
         $~~~~~~~~~~|~h\,:: tl \rightarrow e_2$
       \end{minipage}
     }
     {\hspace{-1em}
       \begin{minipage}[c]{10em}
         ~ $\ecase e^* \eof \enil \, \rightarrow e_1^*$ \\
         $~~~~~~~~|~h\,::_{NC} tl\, \rightarrow e_2^*$ \\
         $~~~~~~~~|~h::_{C} tl \rightarrow e_2^*$
       \end{minipage}\hspace{-1em}
     }{\grt'}}~\textbf{e-u-caseL}
}

\newcommand{\elrcaseL}
{ \inferrule
  {\ctx \jelabc{t}{e}{e'}{\tlist{n}{\alpha}{\tau}}\\
   \Delta; \Phi_a \wedge n = 0  ;\Gamma \jelabc{t'}{e_1}{e_1'}{\tau'}\\
   i, \Delta; \Phi_a \wedge n = i+1;  h: \tbox{\tau},
   tl : \tlist{i}{\alpha}{\tau}, \Gamma \jelabc{t'}{e_2}{e_2'}{\tau'}
\\
   i, \beta, \Delta; \Phi_a \wedge n = i+1 \wedge \alpha = \beta +1 ;
   h: \tau, tl : \tlist{i}{\beta}{\tau}, \Gamma \jelab{t'}{e_2}{e_2'}{e_2^{**}}{e_2'^{**}}{\tau'}
   }
   {\ctx \jelab{t+t'}
     { \hspace{-0.5em}
       \begin{minipage}[c]{9em}
         ~ $\ecase e \eof \enil \rightarrow e_1$ \\
         $~~~~~~~~~~|~h\,:: tl \rightarrow e_2$
       \end{minipage}
     }
     {\hspace{-0.5em}
       \begin{minipage}[c]{9em}
         ~ $\ecase e \eof \enil \rightarrow e_1'$ \\
         $~~~~~~~~~~|~h\,:: tl \rightarrow e_2'$
       \end{minipage}
     }
     {\hspace{-0.5em}
       \begin{minipage}[c]{10em}
         ~ $\ecase e^* \eof \enil \, \rightarrow e_1^*$ \\
         $~~~~~~~~|~h\,::_{NC} tl\, \rightarrow e_2^*$ \\
         $~~~~~~~~|~h::_{C} tl~~~ \rightarrow e_2^{**}$
       \end{minipage}\hspace{-0.5em}
     }{\hspace{-1em}
       \begin{minipage}[c]{10em}
         ~ $\ecase e'^* \eof \enil \, \rightarrow e_1'^*$ \\
         $~~~~~~~~|~h\,::_{NC} tl\, \rightarrow e_2'^*$ \\
         $~~~~~~~~|~h::_{C} tl~~~ \rightarrow e_2'^{**}$
       \end{minipage}
     }{\tau'}}~\textbf{e-r-caseL}
}




\newcommand{\eliLam}
{ \inferrule{
    i::S, \octx \jelabcu{k}{t}{e}{\grt} \\
    i \not \in \fiv{\Phi_a; \Omega} 
  }
  { \octx \jelabun{0}{0}{\eLam. e}{\eLam i. e^*}{\tforall{i}{k}{t} \grt}}~\textbf{e-u-iLam}
}


\newcommand{\elriLam}
{ \inferrule{
    i::S, \ctx \jelabc{t}{e}{e'}{\tau} \\
    i \not \in \fiv{\Phi_a; \Gamma} 
  }
  { \ctx \jelab{0}{\eLam. e}{\eLam. e'}{\eLam i. e^*}{\eLam i. e'^*}{\tforalld{i}{t} \tau}}~\textbf{e-r-iLam}}
%

\newcommand{\eliApp}
{  \inferrule{
    \octx \jelabcu{k}{t}{e}{\tforall{i}{k'}{t'} \grt}\\
    \Delta \vdash I : S
  }
  {\octx \jelabun{k+k'[I/i]+\kiApp}{t+t'[I/i]+\kiApp}{e []}{e^* [I]}{\grt\{ I/ i\}}}~\textbf{e-u-iApp}
}

\newcommand{\elriApp}
{  \inferrule{
    \ctx \jelabc{t}{e}{e'}{\tforalld{i}{t'} \tau}\\
    \Delta \vdash I : S
  }
  {\ctx \jelab{t+t'[I/i]}{e []}{e' []}{e^* [I]}{e'^* [I]}{\tau\{ I/ i\}}}~\textbf{e-r-iApp}}

% 

\newcommand{\elpack}{
\inferrule
{
  \octx  \jelabcu{k}{t}{e}{\grt\{I/i\}}\\
  \Delta \sty{I}{\sort}
}
{
  \octx  \jelabun{k}{t}{\epack e}{\epack e^* \ewith I}{\texists{i} \grt}
} ~\textbf{e-u-pack}
}

\newcommand{\elrpack}{
\inferrule
{
  \ctx  \jelabc{t}{e}{e'}{\tau\{I/i\}}\\
  \Delta \sty{I}{\sort}
}
{
  \ctx  \jelab{t}{\epack e}{\epack e'}{\epack e^* \ewith I}{\epack e'^* \ewith I}{\texists{i} \tau}
} ~\textbf{e-r-pack}
}


\newcommand{\elunpack}{
\inferrule
{
  \octx \jelabcu{k_1}{t_1}{e_1}{\texists{i} \grt_1}\\
  \sorted{i}, \Delta; \Phi_a ; x: \grt_1, \Omega \jelabcu{k_2}{t_2}{e_2}{\grt_2}\\
  i \not\in FV(\Phi_a;\Omega, \grt_2, k_2,t_2)
}
{
  \octx  \jelabun{k_1+k_2+\kunpack}{t_1+t_2}{\eunpack e_1 \eas x \ein  e_2}{\eunpack e_1 \eas (x, i) \ein  e_2}{\eunpack e_1^* \eas (x, i) \ein  e_2^* }{\grt_2}
}~\textbf{e-u-unpack}
}

\newcommand{\elrunpack}{
\inferrule
{
  \ctx \jelabc{t_1}{e_1}{e_1'}{\texists{i} \tau_1}\\
  \sorted{i}, \Delta; \Phi_a; x: \tau_1, \Gamma \jelabc{t_2}{e_2}{e_2'}{\tau_2}\\
  i \not\in FV(\Phi_a;\Gamma, \tau_2, t_2) \\
  e_1^{**} = \eunpack e_1^* \eas (x, i) \ein  e_2^* \\
  e_2^{**} = \eunpack e_1'^* \eas (x, i) \ein  e_2'^*
}
{
  \ctx  \jelab{t_1+t_2}{\eunpack e_1 \eas x \ein  e_2}{\eunpack e_1' \eas x \ein  e_2'}{e_1^{**}}{e_2^{**}}{\tau_2}
}~\textbf{e-r-unpack}
}



\newcommand{\elrlet}
{\inferrule{
  \ctx \jelabc{t_1}{e_1}{e_1'}{\tau_1}\\
  \Delta; \Phi_a; x: \tau_1, \Gamma  \jelabc{t_2}{e_2}{e_2'}{\tau_2}
}
{ \ctx \jelab{t_1+t_2}{ \elet x = e_1 \ein e_2 }{\elet x = e_1' \ein e_2'}{ \elet x = e_1^* \ein e_2^*}{\elet x = e_1'^* \ein e_2'^*}{
  \tau_2} }~\textbf{e-r-let}
}

\newcommand{\ellet}
{\inferrule{
  \octx \jelabcu{k_1}{t_1}{e_1}{\grt_1}\\
  \Delta; \Phi_a; x: \grt_1, \Omega  \jelabcu{k_2}{t_2}{e_2}{\grt_2}
}
{ \octx \jelabun{k_1+k_2+\klet}{t_1+t_2+\klet}{ \elet x = e_1 \ein e_2 }{ \elet x = e_1^* \ein e_2^*}{
  \grt_2} }~\textbf{e-u-let}
}



\newcommand{\elcandIntro}
{\inferrule
{
\Delta; \Phi_a \sat C \\
  \Delta; \Phi_a \wedge C; \Omega  \jelabcu{k}{t}{e}{\grt}
}
{
  \octx  \jelabcu{k}{t}{e}{\tcprod{C}{\grt}}
} ~\textbf{e-u-andI}
}


\newcommand{\elrcandIntro}
{\inferrule
{
\Delta; \Phi_a \sat C \\
  \Delta; \Phi_a \wedge C; \Gamma  \jelabc{t}{e}{e'}{\tau}
}
{
  \ctx  \jelabc{t}{e}{e'}{\tcprod{C}{\tau}}
} ~\textbf{e-r-andI}
}

\newcommand{\elcandElim}
{
\inferrule
{
  \octx \jelabcu{k_1}{t_1}{e_1}{\tcprod{C}{\grt_1}}\\
  \Delta; \Phi_a \wedge C; x :\grt_1, \Omega  \jelabcu{k_u}{t_2}{ e_2}{\grt_2}
}
{
  \ctx  \jelabun{k_1+k_2}{t_1+t_2}{\clet e_1 \eas x \ein e_2}{\clet e_1^* \eas x \ein e_2^*}{\grt_2}
} ~\textbf{e-u-c-andE}
}


\newcommand{\elrcandElim}
{
\inferrule
{
  \ctx \jelabc{t_1}{e_1}{e_1 '}{\tcprod{C}{\tau_1}}\\
  \Delta; \Phi_a \wedge C; x :\tau_1, \Gamma  \jelabc{t_2}{ e_2}{e_2'}{\tau_2}
}
{
  \ctx  \jelab{t_1+t_2}{\clet e_1 \eas x \ein e_2}{\clet e_1' \eas x \ein e_2'}{\clet e_1^* \eas x \ein e_2^*}{\clet e_1'^* \eas x \ein e_2'^*}{\tau_2}
} ~\textbf{e-r-c-andE}
}

\newcommand{\elcimplIntro}
{
\inferrule
{
\Delta; \Phi_a \wedge C; \Omega  \jelabcu{k}{t}{e}{\grt}
}
{
  \octx  \jelabcu{k}{t}{e}{\tcimpl{C}{\grt}}
} ~\textbf{e-u-c-impI}
}


\newcommand{\elrcimplIntro}
{
\inferrule
{
\Delta; \Phi_a \wedge C; \Gamma  \jelabc{t}{e}{e'}{\tau}
}
{
  \ctx  \jelabc{t}{e}{e'}{\tcimpl{C}{\tau}}
} ~\textbf{e-r-c-impI}
}


\newcommand{\elcimplElim}
{
\inferrule
{
  \octx  \jelabcu{k}{t}{e}{\tcimpl{C}{\grt}}\\
\Delta; \Phi_a \sat C
}
{
  \octx  \jelabcu{k}{t}{\ecelim e}{\grt}
} ~\textbf{e-u-c-implE}
}


\newcommand{\elrcimplElim}
{
\inferrule
{
  \ctx  \jelabc{t}{e}{e'}{\tcimpl{C}{\tau}}\\
\Delta; \Phi_a \sat C
}
{
  \ctx  \jelabc{t}{\ecelim e}{\ecelim  e'}{\tau}
} ~\textbf{e-r-c-implE}
}




\newcommand{\elprimapp}
{\inferrule{
    \primctx(\zeta) = \grt_1 \uarr{k}{t} \grt_2 \\
    \octx \jelabcu{k'}{t'}{e}{\grt_1}
}
{
  \octx \jelabcu{k+k'}{t+t'}{\zeta \eapp e}{\grt_2}}~\textbf{e-u-primapp}
}

\newcommand{\elrprimapp}
{\inferrule{
    \primctx(\zeta) = \tau_1 \tarrd{t} \tau_2 \\
    \ctx \jelabc{t'}{e}{e'}{\tau_1}
}
{
 \ctx \jelabc{t+t'}{\zeta \eapp e}{\zeta \eapp e'}{
  \tau_2}}~\textbf{e-r-primapp}}



\newcommand{\elrletMax}
{
  \inferrule{
  \rctx{1} \jelabcu{k_1}{t_1}{e_1}{\grt_1} \\
  \Delta; \Phi_a; x: \tchs{\grt_1}, \Gamma \jelabc{t_2}{e_2}{e}{\tau_2}
}
{ \ctx \jelab{t_1+t_2+\klet}{ \elet x = e_1 \ein e_2}{ e}{ \elet x = e_1^* \ein e_2^*}{ e^*}{\tau_2} }~\textbf{e-r-let-e}
}

\newcommand{\elrletcsym}
{
  \inferrule{
  \rctx{2} \jelabcu{k_1}{t_1}{e_1}{\grt_1} \\
  \Delta; \Phi_a; x: \tchs{\grt_1}, \Gamma \jelabc{t_2}{e}{e_2}{\tau_2}
}
{ \ctx \jelab{t_2-k_1-\klet}{ e }{\elet x = e_1 \ein e_2}{ e^*}{\elet x = e_1^* \ein e_2^*}{\tau_2} }~\textbf{e-r-e-r-let}
}


\newcommand{\elrappfun}
{
  \inferrule{
    \rctx{1} \jelabcu{k_1}{t_1}{e_1}{\grt_1 \uarr{k}{t} \grt_2}
  \\ \ctx \jelabc{t_2}{e_2}{e_2'}{\tch{\grt_1}{\grt_2'}}
}
{\ctx \jelab{t_1+t_2+t+\kapp}{e_1 \eapp e_2}{e_2'}{e_1^* \eapp e_2^*}{e_2'^*}{\tch{\grt_2}{\grt_2'}}}~\textbf{e-r-app-e}}




\newcommand{\elrappfunsym}
{
  \inferrule{
    \rctx{2} \jelabcu{k_1}{t_1}{e_1'}{\grt_1' \uarr{k}{t} \grt_2'}
  \\ \ctx \jelabc{t_2}{e_2}{e_2'}{\tch{\grt_2}{\grt_1'}}
}
{\ctx \jelab{t_2-k_1-k-\kapp}{e_2 }{e_1' \eapp  e_2'}{e_2^*}{e_1'^* \eapp  e_2'^*}{
  \tch{\grt_2}{\grt_2'}}}~\textbf{e-r-e-r-app}}


\newcommand{\elrecase}
{  \inferrule{
    \rctx{2} \jelabcu{k'}{\_}{e'}{\grt_1 + \grt_2} \\
    \Delta; \Phi_a; x: \tchs{\grt_1}, \Gamma \jelabc{t}{e}{e_1'}{\tau}\\
    \Delta; \Phi_a; y: \tchs{\grt_2}, \Gamma \jelabc{t}{e}{e_2'}{\tau}
}{\ctx \jelab{t-k'-\kcase}{e}{\ecase(e', x.e_1', y.e_2')}{e^*}{\ecase(e'^*, x.e_1'^*, y.e_2'^*)}{\tau}}~\textbf{e-r-e-r-case}}
%

\newcommand{\elrcasee}
{  \inferrule{
    \rctx{1} \jelabcu{\_}{t}{e}{\grt_1 + \grt_2} \\
    \Delta; \Phi_a; x: \tchs{\grt_1}, \Gamma \jelabc{t'}{e_1}{e'}{\tau}\\
    \Delta; \Phi_a; y: \tchs{\grt_2}, \Gamma \jelabc{t'}{e_2}{e'}{\tau}
}{\ctx \jelab{t'+t+\kcase}{\ecase(e, x.e_1, y.e_2)}{e'}{\ecase(e^*, x.e_1^*, y.e_2^*)}{e'^*}{\tau}}~\textbf{e-r-case-r-e}}
%



\newcommand{\elsubsum}
{
  \inferrule
  {
    \Delta; \Phi_a; \Omega \jelabcu{k}{t}{e}{\grt} \\
    \Delta; \Phi_a \jasubtype{\grt}{\grt'} \\
    \Delta; \Phi_a \sat \cleq{k'}{k} \\
    \Delta; \Phi_a \sat \cleq{t}{t'}
  }
  {
    \Delta; \Phi_a; \Omega \jelabcu{k'}{t'}{e}{\grt'} \\
  }~\textbf{e-u-$\sqsubseteq$}
}



\newcommandx{\elrsubsum}[4][1=,2=,3=,4=]
{
  \inferrule
  {
    \Delta; \Phi_a; \Gamma \jelabc{t}{e_1}{e_2}{\tau}~~#1 \\
    \Delta; \Phi_a \jsubtype{\tau}{\tau'} ~~#2\\
    e' = \ecoerce{\tau}{\tau'} ~~#3\\
    \Delta; \Phi_a \sat \cleq{t}{t'}~~#4
  }
  {
    \Delta; \Phi_a; \Gamma \jelab{t'}{e_1}{e_2}{e' \eapp e_1^*}{e' \eapp e_2^*}{\tau'} \\
  }~\textbf{e-r-$\sqsubseteq$}
}


\newcommand{\elsplit}
{
  \inferrule
  {
    \Delta; C \wedge \Phi_a; \Omega \jelabcu{k}{t}{e}{\grt} \\
    \Delta; \neg C \wedge \Phi_a; \Omega \jelabun{k}{t}{e}{e^{**}}{\grt} \\
    \Delta \wfcs{C}
  }
  {
    \Delta; \Phi_a; \Omega \jelabun{k}{t}{e}{\esplit (e^{*},e^{**}) \ewith C}{\grt} \\
  }~\textbf{e-u-split}
}


\newcommand{\elrsplit}
{
  \inferrule
  {
    \Delta; C \wedge \Phi_a; \Gamma \jelabc{t}{e_1}{e_2}{\tau} \\
    \Delta; \neg C \wedge \Phi_a; \Gamma \jelab{t}{e_1}{e_2}{e_1^{**}}{e_2^{**}}{\tau} \\
    \Delta \wfcs{C}
  }
  {
    \Delta; \Phi_a; \Gamma \jelab{t}{e_1}{e_2}{\esplit (e_1^*, e_1^{**}) \ewith C}{\esplit (e_2^*, e_2^{**}) \ewith C}{\tau} \\
  }~\textbf{e-r-split}
}


\newcommand{\elcontra}
{
  \inferrule
  {
    \Delta; \Phi_a \sat \bot\\
    \Delta; \Phi_a \wfty{\Omega}
  }
  {
    \octx \jelabun{k}{t}{e}{\econtra e}{\tau} \\
  }~\textbf{e-u-contra}
}

\newcommand{\elrcontra}
{
  \inferrule
  {
    \Delta; \Phi_a \sat \bot\\
    \Delta; \Phi_a \wfty{\Gamma}
  }
  {
    \ctx \jelab{t}{e_1}{e_2}{\econtra e_1}{\econtra e_2}{\tau} \\
  }~\textbf{e-r-contra}
}


%%% Local Variables:
%%% mode: latex
%%% TeX-master: "main"
%%% End:
