# Supplementary material for: Bidirectional Type Checking for Relational Properties
Source: arXiv:1812.05067 source file (2018-12-12)
Supplement: Supplementary file 25 [file elaboration-rules.tex]

\begin{figure*}
  \fbox{$\Delta; \Phi_a; \Gamma
    \jelab{t}{e_1}{e_2}{e_1^*}{e_2^*}{\tau}$} ~ Expressions
  $e_1 \rdiff e_2$ are embedded into $e_1^* \rdiff e_1^*$ with the
  relational type $\tau$
  and the relational cost $t$.\\\\
  \fbox{$\Delta; \Phi_a; \Omega \jelabun{k}{t}{e}{e^*}{\grt}$} ~
  Expression $e$ is embedded into $e*$ with the unary type $\grt$
  and the minimum and maximum execution costs $k$ and $t$, respectively.\\\\

\framebox{General rules}
  \begin{mathpar}
    \elswitch
    %
    \and
    % 
    \elnochange
    % 
    \and
  \end{mathpar}


\framebox{Constant integers and unit}
\begin{mathpar}
  \elconst
  \and
  \elrconst
  % 
  \and
  % 
  \elunit
  \and
  \elrunit
  \end{mathpar}




  \framebox{Variables $x$}
  \begin{mathpar}
    \elvar
    \and
    \elrvar
  \end{mathpar}
  

 \framebox{$\einl e $ }
\begin{mathpar}
  \elinl
  \and
  % 
  \elrinl
  % 
\end{mathpar}


\framebox{$\einr e $ }
\begin{mathpar}
  \elinr
  \and
  \elrinr
 \end{mathpar}

\framebox{$\ecase(e,x.e_1,y.e_2)$}
\begin{mathpar}
  \elcase
  \and
  % 
  \elrcase
\end{mathpar}


\caption{Embedding Rules (Part 1)}
  \label{fig:elab-rules1}
\end{figure*}

%

\begin{figure*}

\framebox{$\efix f(x).e$}
\begin{mathpar}
   \elfix
    \and
    %
    \elrfix
    %
    \and
    %
    \elrfixNC
\end{mathpar}


\framebox{$e_1 \eapp e_2$}
\begin{mathpar}
  \elapp
  \and
  % 
  \elrapp
  % 
\end{mathpar}


\framebox{$\la e_1, e_2 \ra$}
\begin{mathpar}
    \elprod
    \and
    \elrprod
    \and
  \end{mathpar}
  \caption{Embedding Rules (Part 2)}
  \label{fig:elab-rules2}



\framebox{$\eleft (e)$}
\begin{mathpar}
  \elproj
  \and
  \elrproj
  \and
\end{mathpar}


\end{figure*}

    

\begin{figure*}

  \framebox{$\enil$}
\begin{mathpar}
  \elnil
  \and
  \elrnil
  \and
  \end{mathpar}


\framebox{$\econs(e_1,e_2)$}
\begin{mathpar}
  \elcons
  \and
  \elrcons
    \and
    \elrconsbox
    \and
\end{mathpar}

\framebox{$\ecase e \eof \enil \rightarrow e_1 ~|~ h::tl \rightarrow e_2$}
\begin{mathpar}
  \elcaseL
  \and
  \elrcaseL
    \and
\end{mathpar}

\framebox{$\eLam e$}
  \begin{mathpar}
    \eliLam
    \and
    % 
    \elriLam
\end{mathpar}
  
\framebox{$e \eApp $}
  \begin{mathpar}
    \eliApp
    % 
    \and
    % 
    \elriApp
  \end{mathpar}



  \caption{Embedding Rules (Part 3)}
  \label{fig:elab-rules3}
\end{figure*} 



\begin{figure*}

  \framebox{$\epack e$}
\begin{mathpar}
  \elpack
  \and
  \elrpack
\end{mathpar}


\framebox{$\eunpack e \eas x \ein e'$}
\begin{mathpar}
  \elunpack
  % 
  \and
  % 
  \elrunpack
  \end{mathpar}



\framebox{$\elet x = e_1 \ein e_2$}
\begin{mathpar}
  \ellet
  \and
  \elrlet
\end{mathpar}

\framebox{$\tcprod{C}{\tau}$ intro. rules}
\begin{mathpar}
  \elcandIntro
  \and
  \elrcandIntro
\end{mathpar}

\framebox{$\tcprod{C}{\tau}$ elim. rules}
\begin{mathpar}
  \elcandElim
  \and
  \elrcandElim
\end{mathpar}

\framebox{$\tcimpl{C}{\tau}$ intro. rules}
\begin{mathpar}
  \elcimplIntro
  \and
  \elrcimplIntro
\end{mathpar}

  \caption{Embedding Rules (Part 4)}
  \label{fig:elab-rules4}
\end{figure*} 


\begin{figure*} 


\framebox{$\tcprod{C}{\tau}$ elim. rules}
\begin{mathpar}
  \elcimplElim
  \and
  \elrcimplElim
\end{mathpar}


\framebox{Primitive application}
\begin{mathpar}
  \elprimapp
  \and
  \elrprimapp
  \and
  \elcontra
  \and
  \elrcontra
\end{mathpar} 

\framebox{Subsumption}
\begin{mathpar}
  \elsubsum
  \and
  \elrsubsum
\end{mathpar}


\framebox{Constraint-based rules}
\begin{mathpar}
  \elsplit
  \and
  \elrsplit
\end{mathpar}
  \caption{Embedding Rules (Part 5)}
  \label{fig:elab-rules5}
\end{figure*} 



\begin{figure*}
\framebox{Heuristic rules}
  \begin{mathpar}
    \elrletMax
    \and
    \elrletcsym
    \and
    \elrappfun
    \and
    \elrappfunsym
    \and
    \elrcasee
    \and 
    \elrecase

  \end{mathpar} 
  \caption{Embedding Rules (Part 6)}
  \label{fig:elab-rules6}
\end{figure*} 


%%% Local Variables:
%%% mode: latex
%%% TeX-master: "main"
%%% End:
