# Supplementary material for: Bidirectional Type Checking for Relational Properties
Source: arXiv:1812.05067 source file (2018-12-12)
Supplement: Supplementary file 26 [file invariant-alg-typing.tex]

\begin{thm}[Invariant of the Algorithmic Typechecking]\label{invariant:alg-typechecking} We have the following. 
  \begin{enumerate}
  \item Assume that $\uctx \chexec{e}{\grt}{k}{t}{\Phi}$ and
    $\fivars{\Phi_a,\Omega; \grt,k,t} \subseteq dom(\Delta, \psi_a)$. Then $\fivars{\Phi} \subseteq
    dom(\Delta;\psi_a)$.
\item  Assume that $\uctx \infexec{e}{\grt}{\psi}{k}{t}{\Phi}$ and
    $\fivars{\Phi_a,\Omega} \subseteq dom(\Delta, \psi_a)$. Then  $\fivars{\grt,k, t,\Phi} \subseteq
dom(\Delta, \psi; \psi_a)$.
\item Assume that $\bctx \chdiff{e}{e'}{\tau}{t}{\Phi}$ and
  $\fivars{\Phi_a,\Gamma,\tau,t} \subseteq dom(\Delta, \psi_a)$.Then
  $\fivars{\Phi} \subseteq dom(\Delta;\psi_a)$.
\item Assume that $\bctx \infdiff{e}{e'}{\tau}{\psi}{t}{\Phi}$ and
  $\fivars{\Phi_a,\Gamma} \subseteq dom(\Delta,\psi_a)$.Then
  $\fivars{\tau, t, \Phi} \subseteq dom(\Delta;\psi;\psi_a)$.
  \end{enumerate} 
\end{thm}

 
% \begin{thm}[Invariant of the Algorithmic Subtyping]\label{invariant:alg-subtyping} We have the following. 
%   \begin{enumerate}
%     \item Assume that $\Delta ; \psi_a; \Phi_a \jalgasubtype{\grt'}{\grt}{\Phi}$ and $\fivars{\Phi_a,\grt, \grt'}
% \subseteq \Delta, \psi_a$. Then $\fivars{\Phi} \subseteq \Delta, \psi_a$.

%     \item Assume that $\Delta ; \psi_a; \Phi_a \jalgsubtype{\tau'}{\tau}{\Phi}$ and $\fivars{\Phi_a,\tau, \tau'}
% \subseteq \Delta, \psi_a$. Then $\fivars{\Phi} \subseteq \Delta, \psi_a$.
%       \end{enumerate} 
% \end{thm}




%%% Local Variables:
%%% mode: latex
%%% TeX-master: "main"
%%% End:
