# Supplementary material for: Bidirectional Type Checking for Relational Properties
Source: arXiv:1812.05067 source file (2018-12-12)
Supplement: Supplementary file 27 [file main.tex]

\documentclass[a4paper]{article}

\usepackage[a4paper,total={6in, 8.5in}]{geometry}
\usepackage{amsmath,amssymb,amsthm,bm}
\usepackage{../mathpartir}
\usepackage{stmaryrd}
\usepackage{soul}
\usepackage{listings} 
\usepackage{xcolor}
\usepackage{rotating}
\usepackage{setspace}
\usepackage{wasysym}
\usepackage{thmtools}
\usepackage{morefloats}
\usepackage{enumitem}

\usepackage{mathtools}
\DeclarePairedDelimiter{\ceil}{\lceil}{\rceil}
\DeclarePairedDelimiter{\floor}{\lfloor}{\rfloor}
\usepackage{xargs}
\usepackage[colorlinks, allcolors = blue,]{hyperref}
\numberwithin{equation}{section}

\usepackage{cleveref}


\newcommand{\esyntax}[1]{\mathsf{#1}}



\newcommand{\ezgi}[1]{{\color{red}[\text{Ezgi TODO: #1}]}}

\newcommand{\tname}{RelCost}
\newcommand{\bitname}{BiRelCost}
\newcommand{\tnamemin}{RelCost Core}

\newif\ifextra
\extratrue 

\title{Bidirectional Type Analysis for Relational Costs}
\author{}
\input{../ldefs}
\input{../defs}
\input{bdefs}  


\date{}

\begin{document}
\maketitle


%%%%%%%%%%%%%%%%%%%%%%%%%  



\section{Structure of the Appendix}


This appendix considers the following additions to the main paper.
\begin{itemize}
\item The constrained type $\tcimpl{C}{\tau}$, which is eliminated with
  the ``$\ecelim e$'' construct.
\item The type $\achange\,\grt$ is generalized to
  $\tch{\grt_1}{\grt_2}$ (like in {\tname}'s appendix), allowing us to
  relate two expressions of two different unary types $\grt_1$ and
  $\grt_2$, respectively. As a result of this change, \textbf{switch}
  rule, \textbf{$\to \wexec$} subtyping rule, and some of the
  asynchronous rules are also generalized.%  The advantage of this
  % generalization is useful for the $\kw{2Dcount}$ example, explained
  % in depth in Section \ref{sec:examples}.

\end{itemize}

We first present {\tname}'s syntax, typing and subtyping rules. Then,
we introduce {\tnamemin} and the embedding of {\tname} into
{\tnamemin}. Finally, the bidirectional system {\bitname} is
introduced.% The remaining sections
% describe the necessary definitions, lemmas and theorems for proving
% the soundness of the {\tname}'s unary and binary (relational) typing
% with respect to the abstract cost semantics. Finally, we present three
% additional examples.

In \Cref{sec:examples}, we present our benchmark programs along with
the results of the experimental evaluation.

We use some abbreviations throughout. STS stands for ``suffices to
show", TS stands for ``to show", and RTS stands
for ``remains to show".

\listoffigures
\renewcommand{\listtheoremname}{List of Theorems and Lemmas}


\listoftheorems

\clearpage

 
\input{syntax}

% \begin{figure}
%   \centering
%   \[ \begin{array}{@{}l@{~~}l@{~}l@{~}l@{}l}
%        \text{meta~variables} & M & \bnfdef & i,n,m, \cdots \\
%        \text{index~terms} & I,k,t & \bnfdef & \cdots~|~ M \\
%        \text{meta~contexts} & \psi &  \bnfdef & \emptyset~ |~ \psi, M : \sort\\
%        \text{meta~substitutions} & \theta &  \bnfdef & []~ |~ \theta[M \mapsto I]\\
%        \text{constraints} & C &  \bnfdef & \cdots ~ |~ \cforallS{i}{S}{C} ~|~ \cexistsK{i}{S}{C} \\
%        \text{expressions} & e &  \bnfdef & \cdots ~ |~ \eanno{e}{\grt}{k}{t} ~|~ \eannobi{e}{\tau}{t} \\
%      \end{array}\]
%    \caption{Extended {\tnamemin} syntax for {\bitname}}
%  \end{figure}


\input{types-wf}
\input{constraint-gen}

\input{subtyping-rules-defs}
\input{subtyping-rules}


\input{typing-rules-defs}
\input{typing-rules}

% Elaboration
\input{elaboration-rules-defs} 
\input{elaboration-rules} 

% RelCost Core System
\input{type-eq-rules-defs}
\input{type-eq-rules}
\input{typing-rules-min-defs}
\input{typing-rules-min}

\clearpage
% Algorithmic System
\input{alg-typing-rules-defs}
\input{alg-typing-rules}
\input{alg-subtyping-rules}
\input{alg-type-eq-rules-defs}
\input{alg-type-eq-rules} 
\input{ty-anno-erasure}
\clearpage

\subsection{Metatheory}
% \input{subtyping-proj}
% \input{substitution-lemma}
% \input{subtyping-refl}
% \input{alg-trans}
% \input{transitivity}


\input{subtyping-elab}

\input{alg-binary-type-eq-reflexivity}
\input{alg-unary-subtyping-reflexivity}
\input{alg-unary-subtyping-transitivity}


\input{alg-sub-soundness}
\input{alg-sub-completeness}
 
\input{alg-ty-eq-soundness}
\input{alg-ty-eq-completeness}

\input{soundness-relcostM}
\input{completeness-relcostM}

\input{invariant-alg-typing}
\input{alg-soundness}
\input{alg-completeness} 

 \input{examples} 

\end{document}

%%% Local Variables:
%%% mode: latex
%%% TeX-master: t
%%% End:
