# Supplementary material for: Bidirectional Type Checking for Relational Properties
Source: arXiv:1812.05067 source file (2018-12-12)
Supplement: Supplementary file 28 [file soundness-relcostM.tex]

\begin{thm} [Soundness of {\tnamemin} \& Type Preservation of Embedding]\label{thm:relcost-min-soundness}
  The following holds.
  \begin{enumerate}
  \item If $\Delta; \Phi; \Omega \jelabun{k}{t}{e}{e^*}{\grt}$, then
    $\Delta; \Phi; \Omega \jtypeM{k}{t}{e^*}{\grt}$ and $\Delta; \Phi; \Omega \jtype{k}{t}{e}{\grt}$.
  \item If
    $\Delta; \Phi; \Gamma \jelab{t}{e_1}{e_2}{e_1^*}{e_2^*}{\tau}$,
    then $\Delta; \Phi; \Gamma \jtypediffM{t}{e_1^*}{e_2^*}{\tau}$ and
    $\Delta; \Phi; \Gamma \jtypediff{t}{e_1}{e_2}{\tau}$.
\end{enumerate}
\end{thm}

  \begin{proof}
    Proof is by simultaneous induction on the embedding
    derivations. The proof follows from the embedding rules
    presented in \Cref{fig:relcostcore-typing1,fig:relcostcore-typing2,fig:relcostcore-typing3,fig:relcostcore-typing4,fig:relcostcore-typing5,fig:relcostcore-typing6}. We show a few
    representative cases.


\begin{spacing}{1.3}
  \hspace{-1cm} \textbf{Proof of \Cref{thm:relcost-min-soundness}.2:} \\
\begin{mainitem} 
    %%%%%%%%%%%%%%%%%%%%%%%%%%%%%%%%%%%%%%%%%%%%%%%%%%%%%%%%%%%%%%%%%%%%%%% 
  \caseL{$\elswitch[(\star)][(\diam)]$}
  By \Cref{thm:relcost-min-soundness}.1 on $(\star)$, we get $\Delta; \Phi; \Omega \jtypeM{k_1}{t_1}{e_1^*}{\grt_1}~~(\star\star)$. \\
  By \Cref{thm:relcost-min-soundness}.1 on $(\diam)$, we get $\Delta; \Phi; \Omega \jtypeM{k_2}{t_2}{e_2^*}{\grt_2}~~(\diam\diam)$. \\
  Then, we conclude as follows: $\mtyswitch$ 

  \caseL{$\elrsubsum[(\star)][(\diam)][(\dagg)]$}
  By \Cref{thm:relcost-min-soundness}.2 on $(\star)$,  $\Delta; \Phi; \Gamma \jtypediffM{t}{e_1^*}{e_2^*}{\tau}~~(\star\star)$. \\
  By \Cref{lem:sub-elab} using $(\diam)$, we know that $\Delta; \Phi; \cdot \jtypediffM{0}{e'}{e'}{\tau \tarrd{0} \tau'}~~(\diam\diam)$.\\
  By applying \textbf{c-r-app} rule in \Cref{fig:relcostcore-typing3}
  tp $(\star\star)$ and $(\diam\diam)$, we get
  $\Delta; \Phi; \Gamma \jtypediffM{t}{e' \eapp e_1^*}{e' \eapp e_2^*}{\tau'}~~(\spadesuit)$. \\
  By reflexivity of binary type equivalence, we know 
  $\Delta; \Phi_a \jeqtype{\tau'}{\tau'}~~(\spadesuit\spadesuit)$.\\
  Then, we conclude as
  follows:
  \begin{mathpar}
       \inferrule{ 
     \ctx \jtypediffM{t}{e' \eapp e_1^*}{e' \eapp e_2^*}{\tau'}~~(\spadesuit)\\
     \Delta; \Phi_a \jeqtype{\tau'}{\tau'} ~~(\spadesuit\spadesuit)\\\\
    \Delta; \Phi_a \sat \cleq{t}{t'} ~~(\dagg)
  }
  {\ctx \jtypediffM{t'}{e' \eapp e_1^*}{e' \eapp e_2^*}{\tau'} }
  ~{\textbf{c-r}-\pmb{\sqsubseteq}}
  \end{mathpar}

  \end{mainitem}

\end{spacing}

\end{proof}


%%% Local Variables:
%%% mode: latex
%%% TeX-master: "main"
%%% End:
