# Supplementary material for: Bidirectional Type Checking for Relational Properties
Source: arXiv:1812.05067 source file (2018-12-12)
Supplement: Supplementary file 29 [file subtyping-elab.tex]

\begin{lem} [Embedding of Binary Subtyping] \label{lem:sub-elab}
  If $\Delta; \Phi \jsubtype{\tau}{\tau'}$ then $\exists e \in$  {\tnamemin}  such that $\Delta; \Phi; \cdot \jtypediffM{0}{e}{e}{\tau \tarrd{0} \tau'}$.
\end{lem}


\begin{proof}
  Proof is by induction on the subtyping derivation. We denote the
  witness $e$ of type $\tau \tarrd{0} \tau'$ as $\ecoerce{\tau}{\tau'}$ for clarity.

  \begin{mainitem}
    \caseL{\starrD[(\star)][(\diam)]} 
    By IH on $(\star)$, $\exists \ecoerce{\tau_1'}{\tau_1}.~~\Delta; \Phi; \cdot \jmintypesame{0}{\ecoerce{\tau_1'}{\tau_1}}{\tau_1' \tarrd{0} \tau_1}$\\
    By IH on $(\diam)$, $\exists \ecoerce{\tau_2}{\tau_2'}.~~\Delta; \Phi; \cdot \jmintypesame{0}{\ecoerce{\tau_2}{\tau_2'}}{\tau_2 \tarrd{0} \tau_2'}$\\
    
    Then, using these two statements and $\Delta; \Phi \sat t \leq t'$
    with binary subeffecting rule (rule \textbf{c-r-$\sqsubseteq$} in \Cref{fig:relcostcore-typing5}), we can
    construct the following derivation where
    $e= \elam x. \elam y. \ecoerce{\tau_2}{\tau_2'} \eapp (x \eapp
    (\ecoerce{\tau_1'}{\tau_1} \eapp y))$
    
    $\Delta; \Phi; \cdot \jmintypesame{0}{e}{(\tau_1 \tarrd{t} \tau_2) \tarrd{0} \tau_1' \tarrd{t'} \tau_2'}$\\
    
    %%%%%%%%%%%%%%%%%%%%%%%%%%%%%%%%%%%%%%%%%%%%%%%%%%%%%%%%%%%%%%%%%%%%%%%
    \caseL{\stunit} Then, we can immediately construct the derivation
    using the rule \textbf{c-nochange} in
    \Cref{fig:relcostcore-typing1}.
    \begin{mathpar}
      \inferrule{ } { \Delta; \Phi; \cdot \jmintypesame{0}{\elam x. \enoch ()}{\trunit \tarrd{0} \tbox{\trunit}}
      }
    \end{mathpar}
 
    %%%%%%%%%%%%%%%%%%%%%%%%%%%%%%%%%%%%%%%%%%%%%%%%%%%%%%%%%%%%%%%%%%%%%%%
    \caseL{\stint}
    Then, we can construct the derivation using the primitive function $\mbox{box}_{\tint} : \trint \tarrd{0} \tbox{\trint}$
    \begin{mathpar}
      \inferrule{ } { \Delta; \Phi; \cdot \jmintypesame{0}{\elam x. \mbox{box}_{\tint} x}{\trint \tarrd{0} \tbox{\trint}}
      }
    \end{mathpar}


   %%%%%%%%%%%%%%%%%%%%%%%%%%%%%%%%%%%%%%%%%%%%%%%%%%%%%%%%%%%%%%%%%%%%%%%
    \caseL{\stintU}
    Then, we can construct the derivation using the primitive function $\mbox{box}_{U} : \tbox{\tch{\tint}{\tint}} \tarrd{0} \trint$
    \begin{mathpar}
      \inferrule{ } { \Delta; \Phi; \cdot \jmintypesame{0}{\elam x. \mbox{box}_{U} x}{\tbox{\tch{\tint}{\tint}} \tarrd{0} \trint}
      }
    \end{mathpar}


    %%%%%%%%%%%%%%%%%%%%%%%%%%%%%%%%%%%%%%%%%%%%%%%%%%%%%%%%%%%%%%%%%%%%%%%
    \caseL{\stbox}
    Then, we can immediately construct the derivation using the rule \textbf{c-der} in
    \Cref{fig:relcostcore-typing1}.
    \begin{mathpar}
      \inferrule{ } { \Delta; \Phi; \cdot \jmintypesame{0}{\elam x. \eder x}{\tbox{\tau} \tarrd{0} \tau}
      }
    \end{mathpar} 

    %%%%%%%%%%%%%%%%%%%%%%%%%%%%%%%%%%%%%%%%%%%%%%%%%%%%%%%%%%%%%%%%%%%%%%%
    \caseL{\stboxD}
    Then, we can immediately construct the derivation using the rule \textbf{c-nochange} in
    \Cref{fig:relcostcore-typing1}.
    \begin{mathpar}
      \inferrule{ } { \Delta; \Phi; \cdot \jmintypesame{0}{\elam x. \enoch x}{\tbox{\tau} \tarrd{0} \tbox{\tbox{\tau}}}
      }
    \end{mathpar}

    %%%%%%%%%%%%%%%%%%%%%%%%%%%%%%%%%%%%%%%%%%%%%%%%%%%%%%%%%%%%%%%%%%%%%%%
    \caseL{\stboxB[(\star)]}
    By IH on $(\star)$, $\exists \ecoerce{\tau_1}{\tau_2}.~~ \Delta; \Phi; \cdot \jmintypesame{0}{\ecoerce{\tau_1}{\tau_2}}{\tau_1 \tarrd{0} \tau_2}$\\

    Then, using $(\star)$ and the rules  \textbf{c-der} and \textbf{c-nochange} in
    \Cref{fig:relcostcore-typing1}, we can construct the derivation 
    \begin{mathpar}
      \inferrule{ } { \Delta; \Phi; \cdot \jmintypesame{0}{\elam x. \enoch ( \ecoerce{\tau_1}{\tau_2} \eapp (\eder x))}{\tbox{\tau_1} \tarrd{0} \tbox{\tau_2}}
      } 
    \end{mathpar}

    %%%%%%%%%%%%%%%%%%%%%%%%%%%%%%%%%%%%%%%%%%%%%%%%%%%%%%%%%%%%%%%%%%%%%%%
    \caseL{\stincl}
    Then, we can immediately construct the derivation using the rule \textbf{c-switch} in
    \Cref{fig:relcostcore-typing1}.
    \begin{mathpar}
      \inferrule{ } { \Delta; \Phi; \cdot \jmintypesame{0}{\elam x. \eswitch x}{\tau \tarrd{0} \tch{\trm{\tau}{1}}{\trm{\tau}{2}}}
      } 
    \end{mathpar}

    %%%%%%%%%%%%%%%%%%%%%%%%%%%%%%%%%%%%%%%%%%%%%%%%%%%%%%%%%%%%%%%%%%%%%%%
    \caseL{\strefl}
    Then, we can immediately construct the derivation 
    \begin{mathpar}
      \inferrule{ } { \Delta; \Phi; \cdot \jmintypesame{0}{\elam x. x}{\tau \tarrd{0} \tau}}
    \end{mathpar}

    %%%%%%%%%%%%%%%%%%%%%%%%%%%%%%%%%%%%%%%%%%%%%%%%%%%%%%%%%%%%%%%%%%%%%%%
    \caseL{\sttrans[(\star)][(\diam)]}
    By IH on $(\star)$, $\exists \ecoerce{\tau_1}{\tau_2}.~~ \sorted{i}, \Delta; \Phi; \cdot \jmintypesame{0}{\ecoerce{\tau_1}{\tau_2}}{\tau_1 \tarrd{0} \tau_2}$\\
    By IH on $(\diam)$, $\exists \ecoerce{\tau_2}{\tau_3}.~~ \sorted{i}, \Delta; \Phi; \cdot \jmintypesame{0}{\ecoerce{\tau_2}{\tau_3}}{\tau_2 \tarrd{0} \tau_3}$\\

    Then, using $(\star)$ and $(\diam)$, we can construct the
    derivation simply by function composition
    \begin{mathpar}
      \inferrule{ } { \Delta; \Phi; \cdot \jmintypesame{0}{\elam x. \ecoerce{\tau_2}{\tau_3} \eapp (\ecoerce{\tau_1}{\tau_2} \eapp x)}{\tau_1 \tarrd{0} \tau_3}
      } 
    \end{mathpar}


    %%%%%%%%%%%%%%%%%%%%%%%%%%%%%%%%%%%%%%%%%%%%%%%%%%%%%%%%%%%%%%%%%%%%%%% 5
    \caseL{\starrboxD}
    Then, we can immediately construct the derivation  where $e= \elam x. \elam y. \enoch (\eder x) \eapp (\eder y))$\\
    $\Delta; \Phi; \cdot \jmintypesame{0}{e}{\tbox{(\tau_1 \tarrd{k} \tau_2)} \tarrd{0} \tbox{\tau_1} \tarrd{0} \tbox{\tau_2}}$\\
    
   %%%%%%%%%%%%%%%%%%%%%%%%%%%%%%%%%%%%%%%%%%%%%%%%%%%%%%%%%%%%%%%%%%%%%%% 5
    \caseL{\starrW}
    Then, we can immediately construct the following derivation where $e= {\elam x. \elam y. \eswitch (x \eapp y)}$ using the \textbf{c-switch} and \textbf{c-app} rules. \\
    $\Delta; \Phi; \cdot \jmintypesame{0}{e}{(\tch{\grt_1 \uarr{k}{t} \grt_2}{\grt_1' \uarr{k'}{t'} {\grt_2'}}) \tarrd{0} \tch{\grt_1}{\grt_1'} \tarrd{t-k'} \tch{\grt_2}{\grt_2'}}$\\

    %%%%%%%%%%%%%%%%%%%%%%%%%%%%%%%%%%%%%%%%%%%%%%%%%%%%%%%%%%%%%%%%%%%%%%% 5
    \caseL{\stforallD[(\star)]}
    By IH on $(\star)$, $\exists \ecoerce{\tau}{\tau'}.~~ \sorted{i}, \Delta; \Phi; \cdot \jmintypesame{0}{\ecoerce{\tau}{\tau'}}{\tau \tarrd{0} \tau'}$\\
    
    Then, using this, the second premise and the \textbf{c-r-iLam} and \textbf{c-r-iApp} rules in {\tnamemin},
    we can construct the following derivation:\\
    
    $\Delta; \Phi; \cdot \jmintypesame{0}{\elam x. \eLam i. \ecoerce{\tau}{\tau'}\eapp(x \eapp  [i])}{(\tforalld{i}{t} \tau) \tarrd{0} \tforalld{i}{t'} \tau' }$\\
    
   %%%%%%%%%%%%%%%%%%%%%%%%%%%%%%%%%%%%%%%%%%%%%%%%%%%%%%%%%%%%%%%%%%%%%%% 5
    \caseL{\stforallboxD}
    Then, we can immediately construct the following derivation using the \textbf{c-der},  \textbf{c-nochange}, \textbf{c-r-iLam} and \textbf{c-r-iApp} rules in \Cref{fig:relcostcore-typing1,fig:relcostcore-typing4}. \\
    
    $\Delta; \Phi; \cdot \jmintypesame{0}{\elam x. \eLam i. \enoch((\eder x)\, [i])}{\tbox{(\tforalld{i}{t} \tau)} \tarrd{0} \tforalld{i}{t'} \tbox{\tau} }$\\

    %%%%%%%%%%%%%%%%%%%%%%%%%%%%%%%%%%%%%%%%%%%%%%%%%%%%%%%%%%%%%%%%%%%%%%% 5
    \caseL{\stforallU}
    Then, we can immediately construct the following derivation where $e= {\elam x. \eLam i. \eswitch (x \, [i])}$ using the \textbf{c-switch} and \textbf{c-iApp} rules in \Cref{fig:relcostcore-typing1,fig:relcostcore-typing4}. \\
    $\Delta; \Phi; \cdot \jmintypesame{0}{e}{(\tch{\tforall{i}{k}{t} \grt}{\tforall{i}{k'}{t'} \grt'}) \tarrd{0} {\tforalld{i}{t-k'} \tch{\grt}{\grt'}}}$\\

    %%%%%%%%%%%%%%%%%%%%%%%%%%%%%%%%%%%%%%%%%%%%%%%%%%%%%%%%%%%%%%%%%%%%%%% 5
    \caseL{\sttimes[(\star)][(\diam)]}
    By IH on $(\star)$, $\exists \ecoerce{\tau_1}{\tau_1'}.~~\Delta; \Phi; \cdot \jmintypesame{0}{\ecoerce{\tau_1}{\tau_1'}}{\tau_1 \tarrd{0} \tau_1'}$\\
    By IH on $(\diam)$, $\exists \ecoerce{\tau_2}{\tau_2'}.~~\Delta; \Phi; \cdot \jmintypesame{0}{\ecoerce{\tau_2}{\tau_2'}}{\tau_2 \tarrd{0} \tau_2'}$\\
    Then, using these two statements and the rules \textbf{c-prod} and \textbf{c-proj} in \Cref{fig:relcostcore-typing2}, we can show the following derivation where $e = \elam x. \la \ecoerce{\tau_1}{\tau_1'} \eapp (\eleft x), \ecoerce{\tau_2}{\tau_2'} \eapp(\eright x) \ra$
    
    $\Delta; \Phi; \cdot \jmintypesame{0}{e}{(\tau_1 \ttimes \tau_2) \tarrd{0} \tau_1' \ttimes \tau_2'}$\\
    

    %%%%%%%%%%%%%%%%%%%%%%%%%%%%%%%%%%%%%%%%%%%%%%%%%%%%%%%%%%%%%%%%%%%%%%% 5
    \caseL{\sttimesbox} We show the direction from right-to-left using
    the rules \textbf{c-der}, \textbf{c-nochange}, \textbf{c-r-proj}, \textbf{c-r-let} and
    \textbf{c-r-prod} in \Cref{fig:relcostcore-typing1,fig:relcostcore-typing2,fig:relcostcore-typing4} where the expression
    \begin{minipage}[t]{1.0\linewidth}
$e= \elam x. \elet a =  \eleft x \ein \\ ~~~~~~~~~~~\elet b = \eright  x \ein \enoch(\la \eder a, \eder b \ra).$
\end{minipage}
\\
    $\Delta; \Phi; \cdot \jmintypesame{0}{e}{\tbox{\tau_1} \ttimes \tbox{\tau_2} \tarrd{0} \tbox{(\tau_1 \ttimes \tau_2)}}$\\
    
    
   %%%%%%%%%%%%%%%%%%%%%%%%%%%%%%%%%%%%%%%%%%%%%%%%%%%%%%%%%%%%%%%%%%%%%%% 5
    \caseL{\sttimesU}
    Then, we can immediately construct the following derivation where $e= {\elam x.  (\la \eswitch \eleft x, \eswitch \eright x \ra)}$ using the \textbf{c-switch}, \textbf{c-r-prod} and \textbf{c-r-proj} rules in \Cref{fig:relcostcore-typing1,fig:relcostcore-typing2}. \\
    $\Delta; \Phi; \cdot \jmintypesame{0}{e}{(\tch{\grt_1 \ttimes \grt_2}{\grt_1' \ttimes {\grt_2'}}) \tarrd{0} \tch{\grt_1}{\grt_1'} \ttimes \tch{\grt_2}{\grt_2'}}$\\

    %%%%%%%%%%%%%%%%%%%%%%%%%%%%%%%%%%%%%%%%%%%%%%%%%%%%%%%%%%%%%%%%%%%%%%% 5
    \caseL{\stsumbox} We can construct the following derivation by
    using the rules \textbf{c-der}, \textbf{c-nochange},
    \textbf{c-r-case}, \textbf{c-r-inl} and \textbf{c-r-inr} in
    \Cref{fig:relcostcore-typing1}
    where the expression
    \begin{minipage}[t]{1.0\linewidth}
$e= \elam x. \ecase(x, a. \enoch (\einl \eder a), b. \enoch (\einr \eder b)).$
\end{minipage}
\\
    $\Delta; \Phi; \cdot \jmintypesame{0}{e}{\tbox{\tau_1} \tsum \tbox{\tau_2} \tarrd{0} \tbox{(\tau_1 \tsum \tau_2)}}$\\
    
    %%%%%%%%%%%%%%%%%%%%%%%%%%%%%%%%%%%%%%%%%%%%%%%%%%%%%%%%%%%%%%%%%%%%%%% 5
    \caseL{\stlist[(\star)][(\diam)][(\dagg)]}
    By IH on $(\dagg)$, $\exists \ecoerce{\tau}{\tau'}.~~\Delta; \Phi; \cdot \jmintypesame{0}{\ecoerce{\tau}{\tau'}}{\tau \tarrd{0} \tau'}$\\
    We first construct the more generic term for type:\\
    \begin{equation}
      \trunit \tarrd{0} \tforallN{n}  \tforallN{n'} \tforallN{\alpha} \tforallN{\alpha'} (\tcprod{(n=n' \wedge \alpha \leq \alpha')} \tlist{n}{\alpha}{\tau}) \tarrd{0} \tlist{n'}{\alpha'}{\tau'}
    \label{eq:sub-list}
  \end{equation}
  and then instantiate the term for \cref{eq:sub-list} later.\\
  It can be shown that such a derivation can be constructed for
  expression \\
    \begin{minipage}[t]{1.0\linewidth}
      $e'= \efix \mbox{fList}(\_). \eLam n. \eLam n'. \eLam \alpha. \eLam \alpha'. \elam x. \clet x \eas e \ein \\
      ~~~~~~\ecase e \eof \\
      ~~~~~~~~\enil \rightarrow \enil \\
      ~~~~~~|~h\,::_{N} tl\, \rightarrow \elet r = \mbox{fList} \eapp () \,[n-1]\,[n'-1] \, [\alpha]  \, [\alpha'] \eapp tl \ein \econsNC(\enoch (\ecoerce{\tau}{\tau'} \eapp \eder h), r) \\
      ~~~~~~|~h::_{C} tl\, \rightarrow \elet r = \mbox{fList} \eapp () \, [n-1] \,[n'-1]\,[\alpha-1]  \, [\alpha'-1] \eapp tl \ein \econsC(\ecoerce{\tau}{\tau'} \eapp h, r)
      $ 
    \end{minipage}
    \\\\
    Then, we can instantiate \mbox{fList} using $(\star)$ and $(\diam)$ as follows where \\
    \begin{minipage}[t]{1.0\linewidth}
    $e''= \elam x.\mbox{fList} \eapp () \eapp [n] [n'] [\alpha] [\alpha'] \eapp x$
  \end{minipage}
\\
    
    $\Delta; \Phi; \cdot \jmintypesame{0}{e''}{\tlist{n}{\alpha}{\tau} \tarrd{0} \tlist{n'}{\alpha'}{\tau'}}$\\
    
    %%%%%%%%%%%%%%%%%%%%%%%%%%%%%%%%%%%%%%%%%%%%%%%%%%%%%%%%%%%%%%%%%%%%%%% 5
    \caseL{\stlistbox} 
    We first construct the more generic term for type
    \begin{equation}
    \trunit \tarrd{0} \tforallN{n} \tforallN{\alpha} \tlist{n}{\alpha}{\tbox{\tau}} \tarrd{0}
    \tbox{(\tlist{n}{\alpha}{\tau})}\label{eq:sub-list-box} 
  \end{equation}

    and then instantiate the term for \cref{eq:sub-list-box} later.
    It can be shown that such a derivation can be constructed for expression \\
    \begin{minipage}[t]{1.0\linewidth}
      $e'= \efix \mbox{fList}(\_). \eLam n. \eLam \alpha. \elam x. \\
      ~~~~~~\ecase e \eof \\
      ~~~~~~~~\enil \rightarrow \enoch (\enil)  \\
      ~~~~~~|~h\,::_{N} tl\, \rightarrow \elet r = \mbox{fList} \eapp () \,[n-1] \, [\alpha] \eapp tl \ein \\
      ~~~~~~~~~~~~~~~~~~~~~~~~~~~~\enoch (\econsNC(\eder h, \eder r)) \\
      ~~~~~~|~h::_{C} tl\, \rightarrow \elet r = \mbox{fList} \eapp () \, [n-1] \,[\alpha-1] \eapp tl \ein \\
      ~~~~~~~~~~~~~~~~~~~~~~~~~~~~\enoch(\econsC(\eder h, \eder r))
      $ 
    \end{minipage}
    \\\\
    Then, we can instantiate \mbox{fList} with a concrete $n$ and $\alpha$ as follows where \begin{minipage}[t]{1.0\linewidth}
    $e''= \elam x. \mbox{fList} \eapp () \eapp [n] [\alpha] \eapp x $
  \end{minipage}

    $\Delta; \Phi; \cdot \jmintypesame{0}{e''}{\tlist{n}{\alpha}{\tbox{\tau}} \tarrd{0} \tbox{(\tlist{n}{\alpha}{\tau})}}$\\
    
    %%%%%%%%%%%%%%%%%%%%%%%%%%%%%%%%%%%%%%%%%%%%%%%%%%%%%%%%%%%%%%%%%%%%%%% 5
    \caseL{\stlistzero}
    We first construct the more generic term for type
    \begin{equation}
    \trunit \tarrd{0} \tforallN{n} \tforallN{\alpha} (\tcprod{\alpha=0}{\tlist{n}{\alpha}{\tau}}) \tarrd{0} \tlist{n}{\alpha}{\tbox{\tau}}\label{eq:sub-list-zero}   
  \end{equation}
    and then instantiate the term for \cref{eq:sub-list-zero} later.
    It can be shown that such a derivation can be constructed for expression\\
    \begin{minipage}[t]{1.0\linewidth}
      $e'= \efix \mbox{fList}(\_). \eLam n. \eLam \alpha. \elam x. \clet x \eas e \ein \\
      ~~~~~~\ecase e \eof  \\
      ~~~~~~~~\enil \rightarrow \enil \\
      ~~~~~~|~h\,::_{N} tl\, \rightarrow \elet r = \mbox{fList} \eapp () \,[n-1] [\alpha] \eapp tl \ein \econsNC(\enoch h, r) \\
      ~~~~~~|~h::_{C} tl\, \rightarrow \econtra $ 
    \end{minipage}
    \\\\
    Then, we can instantiate \mbox{fList} with a concrete $n$ and
    $\alpha$ (note the premise $\alpha=0$) as follows
    where \begin{minipage}[t]{1.0\linewidth}
      $e''= \elam x. \mbox{fList} \eapp () \eapp [n] [\alpha] \eapp x $
  \end{minipage}

    $\Delta; \Phi; \cdot \jmintypesame{0}{e''}{\tlist{n}{0}{\tau} \tarrd{0} \tlist{n}{0}{\tbox{\tau}}}$\\
    
    %%%%%%%%%%%%%%%%%%%%%%%%%%%%%%%%%%%%%%%%%%%%%%%%%%%%%%%%%%%%%%%%%%%%%%% 5
    \caseL{\stexists[(\star)]}
    By IH on $(\star)$, $\exists \ecoerce{\tau}{\tau'}.~~ \sorted{i}, \Delta; \Phi; \cdot \jmintypesame{0}{\ecoerce{\tau}{\tau'}}{\tau \tarrd{0} \tau'}$\\
    
    Then, using this and the \textbf{c-r-pack} and \textbf{c-r-unpack} rules in {\tnamemin} in \Cref{fig:relcostcore-typing4},
    we can construct the following derivation where $e= \elam x. \eunpack x \eas (y, i) \ein \epack (\ecoerce{\tau}{\tau'} \eapp y)  \ewith i$\\
    
    $\Delta; \Phi; \cdot \jmintypesame{0}{e}{(\texists{i} \tau) \tarrd{0} \texists{i} \tau' }$\\
    
   %%%%%%%%%%%%%%%%%%%%%%%%%%%%%%%%%%%%%%%%%%%%%%%%%%%%%%%%%%%%%%%%%%%%%%% 5
    \caseL{\stexistsbox}
    Then, we can immediately construct the following derivation using the \textbf{c-der}, \textbf{c-nochange}, \textbf{c-r-pack} and \textbf{c-r-unpack} rules in in \Cref{fig:relcostcore-typing1,fig:relcostcore-typing4} where $e= \elam x. \eunpack x \eas  (y, i) \ein \enoch(\epack \eder y \ewith i)$. \\
    
    $\Delta; \Phi; \cdot \jmintypesame{0}{e}{(\texists{i} \tbox{\tau}) \tarrd{0} \tbox{(\texists{i} \tau)} }$\\

   %%%%%%%%%%%%%%%%%%%%%%%%%%%%%%%%%%%%%%%%%%%%%%%%%%%%%%%%%%%%%%%%%%%%%%% 5
    \caseL{\stcimpl[(\star)][(\diam)]}
    By IH on $(\diam)$, $\exists \ecoerce{\tau}{\tau'}.~~ \Delta; \Phi; \cdot \jmintypesame{0}{\ecoerce{\tau}{\tau'}}{\tau \tarrd{0} \tau'}$\\
    
    Then, using this and the premise $(\star)$ along with the \textbf{c-r-c-implI} and \textbf{c-r-c-implE} rules in \Cref{fig:relcostcore-typing5},
    we can construct the following derivation where $e= \elam x. \ecoerce{\tau}{\tau'} \eapp (\ecelim x) $\\
    
    $\Delta; \Phi; \cdot \jmintypesame{0}{e}{(\tcimpl{C}{\tau}) \tarrd{0} \tcimpl{C'}{\tau'}}$\\

   %%%%%%%%%%%%%%%%%%%%%%%%%%%%%%%%%%%%%%%%%%%%%%%%%%%%%%%%%%%%%%%%%%%%%%% 5
    \caseL{\stcimplbox}
    Then, we can immediately construct the following derivation using the \textbf{c-der}, \textbf{c-nochange} and \textbf{c-r-c-implE} rules in {\tnamemin} where $e= \elam x. \enoch(\ecelim \eder x)$. \\
    
    $\Delta; \Phi; \cdot \jmintypesame{0}{e}{\tbox{(\tcimpl{C} \tau)} \tarrd{0}  (\tcimpl{C} \tbox{\tau}) }$\\
    
   \caseL{\stcprod[(\star)][(\diam)]}
    By IH on $(\diam)$, $\exists \ecoerce{\tau}{\tau'}.~~ \Delta; \Phi; \cdot \jmintypesame{0}{\ecoerce{\tau}{\tau'}}{\tau \tarrd{0} \tau'}$\\
     
    Then, using this and the premise $(\star)$ along with the \textbf{c-r-c-prodI} and \textbf{c-r-c-prodE} rules in \Cref{fig:relcostcore-typing2},
    we can construct the following derivation where $e= \elam x. \clet x \eas y \ein \ecoerce{\tau}{\tau'} \eapp y $\\
    
    $\Delta; \Phi; \cdot \jmintypesame{0}{e}{(\tcprod{C}{\tau}) \tarrd{0} \tcprod{C'}{\tau'}}$\\

   %%%%%%%%%%%%%%%%%%%%%%%%%%%%%%%%%%%%%%%%%%%%%%%%%%%%%%%%%%%%%%%%%%%%%%% 5
    \caseL{\stcprodbox}
    Then, we can immediately construct the following derivation using the \textbf{c-der}, \textbf{c-nochange}, \textbf{c-r-c-prodI} and \textbf{c-r-c-prodE} rules in \Cref{fig:relcostcore-typing1,fig:relcostcore-typing2,fig:relcostcore-typing4} where $e= \elam x. \clet x \eas y \ein \enoch(\eder y)$. \\
    
    $\Delta; \Phi; \cdot \jmintypesame{0}{e}{ (\tcprod{C} \tbox{\tau}) \tarrd{0}  \tbox{(\tcprod{C} \tau)} }$\\
 
  \end{mainitem}
  
\end{proof}

%%% Local Variables:
%%% mode: latex
%%% TeX-master: "main"
%%% End:
