# Supplementary material for: Bidirectional Type Checking for Relational Properties
Source: arXiv:1812.05067 source file (2018-12-12)
Supplement: Supplementary file 30 [file subtyping-rules-defs.tex]

\newcommand{\stint}{
  \inferrule{
}
{
  \Delta; \Phi_a  \jsubtype{\trint}{\tbox{\trint}}
}~\textbf{int-$\square$}
}

\newcommand{\stintU}{
  \inferrule{
}
{
  \Delta; \Phi_a  \jsubtype{\tbox{\tch{\tint}{\tint}}}{\trint}
}~\textbf{$\square$U-int}
}

\newcommand{\stunit}
{
\inferrule{
}
{
  \Delta; \Phi_a  \jsubtype{\trunit}{\tbox{\trunit}}
}~\textbf{unit}
}
\newcommandx{\starrD}[2][1=, 2=]
{
  \inferrule{
\Delta; \Phi_a  \jsubtype{\tau_1'}{\tau_1}~~ #1 \\
\Delta;\Phi_a  \jsubtype{\tau_2}{\tau_2'}~~ #2 \\
\Delta; \Phi_a \sat t \leq t'
}
{
\Delta; \Phi_a \jsubtype{\tau_1 \tarrd{t} \tau_2}{\tau_1' \tarrd{t'} \tau_2'}
}~\textbf{$\to \wdiff$}
}



\newcommand{\starrboxD}
{
  \inferrule
{
\strut
}
{
\Delta; \Phi_a  \jsubtype{\tbox{(\tau_1 \tarrd{t} \tau_2)}}{ \tbox{\tau_1}
    \tarrd{0} \tbox{\tau_2}}
}~\textbf{$\to \square \wdiff$}
}


\newcommand{\starrW}
{
  \inferrule
{
\strut
}
{
\Delta; \Phi_a  \jsubtype{\tch{\grt_1 \uarr{k}{t} \grt_2}{\grt_1' \uarr{k'}{t'} \grt_2'}}{ \tch{\grt_1}{\grt_1'}
    \tarrd{t-k'} \tch{\grt_2}{\grt_2'}}
}~\textbf{$\to \wexec \wdiff$}
}



\newcommandx{\stforallD}[1][1=]
{
  \inferrule
{
\sorted{i}, \Delta; \Phi_a  \jsubtype{\tau}{\tau'} ~~ #1\\
\sorted{i}, \Delta; \Phi_a \sat \cleq{t}{t'} \\
 i \not\in FV(\Phi_a)
}
{
\Delta; \Phi_a \jsubtype{\tforalld{i}{t}{\tau}}{\tforalld{i}{t'}{\tau'}}
}~\textbf{$\forall \wdiff$}
}


\newcommand{\stforallboxD}
{
  \inferrule
{
}
{
\Delta; \Phi_a  \jsubtype{\tbox{(\tforalld{i}{t}{\tau})}}{\tforalld{i}{0}{\tbox{\tau}}}
}~\textbf{$\forall$ $\square$}
}


\newcommand{\stforallU}
{
  \inferrule
{
}
{
\Delta; \Phi_a  \jsubtype{\tch{\tforall{i}{k}{t}{\grt}}{\tforall{i}{'k}{t'}{\grt'}}}{\tforalld{i}{t-k'}{\tch{\grt}{\grt'}}}
}~\textbf{$\forall$U}
}



\newcommandx{\sttimes}[2][1=, 2=]
{
  \inferrule{
\Delta; \Phi_a  \jsubtype{\tau_1}{\tau_1'} ~~#1\\
\Delta; \Phi_a  \jsubtype{\tau_2}{\tau_2'} ~~#2
}{
\Delta; \Phi_a  \jsubtype{\tau_1 \times \tau_2}{\tau_1' \times \tau_2'}
}~\textbf{$\times$}
}

\newcommand{\sttimesbox}
{\inferrule{
}
{
\Delta; \Phi_a  \jeqtype{\tbox{\tau_1} \times \tbox{\tau_2}}{\tbox{(\tau_1 \times \tau_2)}}
}
~\textbf{$\times\square$}
}

\newcommand{\sttimesU}
{\inferrule{
}
{
\Delta; \Phi_a  \jsubtype{\tch{\grt_1 \times \grt_2}{\grt_1' \times \grt_2'}}{ \tch{\grt_1}{\grt_1'} \times \tch{\grt_2}{\grt_2'}}
}
~\textbf{$\times$U}
}


\newcommand{\stsum}
{
  \inferrule{
\Delta; \Phi_a  \jsubtype{\tau_1}{\tau_1'} \\ 
\Delta; \Phi_a  \jsubtype{\tau_2}{\tau_2'}
}{
\Delta; \Phi_a  \jsubtype{\tau_1 + \tau_2}{\tau_1' + \tau_2'}
}~\textbf{${+}$}
}


\newcommand{\stsumbox}
{
  \inferrule
{
}
{
\Delta; \Phi_a  \jsubtype{\tbox{\tau_1} + \tbox{\tau_2}}{\tbox{(\tau_1 + \tau_2)}}
}~\textbf{${+}\square$}
}

\newcommandx{\stlist}[3][1=,2=,3=]
{
  \inferrule{
\Delta; \Phi_a  \sat \ceq{n}{n'} ~~#1 \\
\Delta; \Phi_a  \sat \cleq{\alpha}{\alpha'} ~~#2\\
\Delta; \Phi_a  \jsubtype{\tau}{\tau'}~~#3
}
{
\Delta; \Phi_a   \jsubtype{\tlist{n}{\alpha}{\tau}}{\tlist{n'}{\alpha'}{\tau'}}
}~\textbf{l1}
}

\newcommand{\stlistzero}
{
  \inferrule
{
\Delta; \Phi_a \models \ceqz{\alpha}
}
{
\Delta; \Phi_a  \jsubtype{\tlist{n}{\alpha}{\tau}}{\tlist{n}{\alpha}\tbox{{\tau}}}
}~\textbf{l2}
}

\newcommand{\stlistbox}
{
  \inferrule
{
% \Delta; \Phi_a \models \ceqz{\alpha}
}
{
\Delta; \Phi_a  \jsubtype{\tlist{n}{\alpha}{\tbox{\tau}}}{\tbox{(\tlist{n}{\alpha}{\tau})}}
}~\textbf{l$\square$}
}

\newcommand{\sttree}
{
  \inferrule{
\Delta; \Phi_a  \sat \ceq{n}{n'} \\
\Delta; \Phi_a  \sat \cleq{\alpha}{\alpha'} \\
\Delta; \Phi_a  \jsubtype{\tau}{\tau'}
}
{
\Delta; \Phi_a   \jsubtype{\ttree{n}{\alpha}{\tau}}{\ttree{n'}{\alpha'}{\tau'}}
}~\textbf{t1}
}

\newcommand{\sttreezero}
{
  \inferrule
{
\Delta; \Phi_a \models \ceqz{\alpha}
}
{
\Delta; \Phi_a  \jsubtype{\ttree{n}{\alpha}{\tau}}{\ttree{n}{\alpha}{\tbox{\tau}}}
}~\textbf{t2}
}

\newcommand{\sttreebox}
{
  \inferrule
{
}
{
\Delta; \Phi_a  \jsubtype{\ttree{n}{\alpha}{\tbox{\tau}}}{\tbox{(\ttree{n}{\alpha}{\tau})}}
}~\textbf{t$\square$}
}

\newcommandx{\stexists}[1][1=]{
  \inferrule
{
\sorted{i}, \Delta; \Phi_a  \jsubtype{\tau}{\tau'} ~~#1 \\
i \not\in FV(\Phi_a)
}
{
\Delta; \Phi_a  \jsubtype{\texists{i}{\tau}}{\texists{i}{\tau'}}
}~\textbf{$\exists$} 
}


\newcommand{\stexistsbox}
{
\inferrule
{
}
{
\Delta; \Phi_a  \jsubtype{\texists{i}{\tbox{\tau}}}{\tbox{(\texists{i}{\tau})}}
}~\textbf{$\exists\square$}
}


\newcommandx{\stcimpl}[2][1=, 2=]
{
  \inferrule{
    \Delta; \Phi_a \wedge C' \sat C ~~#1\\
    \Delta; \Phi_a  \jsubtype{\tau}{\tau'} ~~#2
  }
  {
    \Delta; \Phi_a  \jsubtype{\tcimpl{C}{\tau}}{\tcimpl{C'}{\tau'}}
  }\textbf{c-impl}
}

\newcommand{\stcimplbox}
{
\inferrule
{
}
{
\Delta; \Phi_a  \jsubtype{\tbox{(\tcimpl{C}{\tau})}}{\tcimpl{C}{\tbox{\tau}}}
}~\textbf{c-impl-$\square$}
}


\newcommandx{\stcprod}[2][1=,2=]
{
\inferrule{
\Delta; \Phi_a \wedge C \sat  C' ~~#1 \\
\Delta; \Phi_a  \jsubtype{\tau}{\tau'} ~~#2
}
{
\Delta; \Phi_a  \jsubtype{\tcprod{C}{\tau}}{\tcprod{C'}{\tau'}}
}\textbf{c-and}
}

\newcommand{\stcprodbox}
{
\inferrule
{
}
{
\Delta; \Phi_a  \jsubtype{\tcprod{C}{\tbox{\tau}}}{\tbox{(\tcprod{C}{\tau})}}
}~\textbf{c-and-$\square$}
}


\newcommand{\stbox}
{\inferrule
{
}
{
\Delta; \Phi_a  \jsubtype{\tbox{\tau}}{\tau}
}~\textbf{T}
}

\newcommand{\stboxD}
{\inferrule
{
}
{
\Delta; \Phi_a  \jsubtype{\tbox{\tau}}{\tbox{\tbox{\tau}}}
}~\textbf{D}
}

\newcommandx{\stboxB}[1][1=]
{\inferrule
{
\Delta; \Phi_a  \jsubtype{\tau_1}{\tau_2} #1
}
{
\Delta; \Phi_a  \jsubtype{\tbox{\tau_1}}{\tbox{\tau_2}}
}~\textbf{B-$\square$}
}

\newcommand{\stgrt}
{\inferrule
{
  \Delta;\Phi_a \jasubtype{\grt_1}{\grt_1'} \\
  \Delta;\Phi_a \jasubtype{\grt_2}{\grt_2'}
}
{
\Delta; \Phi_a  \jsubtype{\tch{\grt_1}{\grt_2}}{\tch{\grt_1'}{\grt_2'}}
}~\textbf{U}
}


\newcommand{\stboxpush}
{\inferrule
{
i \in \{1,2\}
}
{
\Delta; \Phi_a  \jsubtype{\tbox{\tau}}{\tpushd{\tau}}
}~\textbf{$\square$-push-L}
}


\newcommand{\stboxpushR}
{\inferrule
{
  \tau \not = \tau_1 \tarrd{k} \tau_2 \\
  \tau \not =  \tch{\grt_1}{\grt_2}
}
{
\Delta; \Phi_a  \jsubtype{\tpushd{\tau}}{\tbox{\tau}}
}~\textbf{$\square$-push-R}
}


\newcommand{\stboxLift}
{\inferrule
{
i \in \{1,2\}
}
{
\Delta; \Phi_a  \jsubtype{\tbox{\tau}}{\tpushd{\trm{\tau}{i}}}
}~\textbf{$\square$-lift}
}


\newcommand{\stboxPull}
{\inferrule
{
\Delta; \Phi_a  \jsubtype{\tau}{\tlift{\trm{\tau}{i}}}
}
{
\Delta; \Phi_a  \jsubtype{\tau}{\tbox{(\tpull{\tau})}}
}~\textbf{$\square$-pull}
}



\newcommand{\stincl}
{\inferrule
{
}
{
\Delta; \Phi_a  \jsubtype{\tau}{\tch{\trm{\tau}{1}}{\trm{\tau}{2}}}
}~\textbf{W}
}

\newcommand{\strefl}
{
\inferrule
{
}
{\Delta; \Phi_a  \jsubtype{\tau}{\tau}
}\textbf{refl}
}

\newcommandx{\sttrans}[2][1=,2=]
{
\inferrule{
\Delta; \Phi_a  \jsubtype{\tau_1}{\tau_2}~~#1 \\
\Delta; \Phi_a  \jsubtype{\tau_2}{\tau_3}~~#2
}
{
\Delta; \Phi_a  \jsubtype{\tau_1}{\tau_3}
}\textbf{tran}
}

\newcommand{\stsplit}
{
\inferrule{
\Delta; \Phi_a \wedge C \sat \eta \\
\Delta; \Phi_a \wedge \cneg{C} \sat  \eta
}
{
\Delta; \Phi_a \sat  \eta
}\textbf{split}
}
%%%%%%%%%%%%%%%%%%%%%%%%%%%%%%%%%%%%%%%%%%%%%%%%%%%%%%%%%%%%%%%%%%%%
% Unary Subtyping
%%%%%%%%%%%%%%%%%%%%%%%%%%%%%%%%%%%%%%%%%%%%%%%%%%%%%%%%%%%%%%%%%%%%


\newcommand{\starrE}
{
  \inferrule{
\Delta; \Phi_a  \jasubtype{\grt_1'}{\grt_1} \\
\Delta;\Phi_a  \jasubtype{\grt_2}{\grt_2'} \\
\Delta; \Phi_a \sat k' \leq k \\
\Delta; \Phi_a \sat t \leq t' 
}
{
\Delta; \Phi_a \jasubtype{\grt_1 \uarr{k}{t} \grt_2}{\grt_1' \uarr{k'}{t'} \grt_2'}
}~\textbf{$\to \wexec$}
}



\newcommand{\stforallE}
{
  \inferrule
{
\sorted{i}, \Delta; \Phi_a  \jasubtype{\grt}{\grt'} \\
\sorted{i}, \Delta; \Phi_a \sat \cleq{k'}{k} \\
\sorted{i}, \Delta; \Phi_a \sat \cleq{t}{t'} \\
 i \not\in FV(\Phi_a)
}
{
\Delta; \Phi_a \jasubtype{\tforall{i}{k}{t}{\grt}}{\tforall{i}{k'}{t'}{\grt}}
}~\textbf{u-$\forall \wexec$}
}



\newcommand{\stutimes}
{
  \inferrule{
\Delta; \Phi_a  \jasubtype{\grt_1}{\grt_1'} \\
\Delta; \Phi_a  \jasubtype{\grt_2}{\grt_2'}
}{
\Delta; \Phi_a  \jasubtype{\grt_1 \times \grt_2}{\grt_1' \times \grt_2'}
}~\textbf{u-$\times$}
}


\newcommand{\stutsum}
{
  \inferrule{
\Delta; \Phi_a  \jasubtype{\grt_1}{\grt_1'} \\
\Delta; \Phi_a  \jasubtype{\grt_2}{\grt_2'}
}{
\Delta; \Phi_a  \jasubtype{\grt_1 \tsum \grt_2}{\grt_1' \tsum \grt_2'}
}~\textbf{u-$\tsum $}
}


\newcommand{\stulist}
{
  \inferrule{
\Delta; \Phi_a  \sat \ceq{n}{n'} \\
\Delta; \Phi_a  \jasubtype{\grt}{\grt'}
}
{
\Delta; \Phi_a   \jasubtype{\ulist{n}{\grt}}{\ulist{n'}{\grt'}}
}~\textbf{u-l}
}

\newcommand{\stutree}
{
  \inferrule{
\Delta; \Phi_a  \sat \ceq{n}{n'} \\
\Delta; \Phi_a  \jasubtype{\grt}{\grt'}
}
{
\Delta; \Phi_a   \jasubtype{\utree{n}{\grt}}{\utree{n'}{\grt'}}
}~\textbf{u-t}
}



\newcommand{\stuexists}{
  \inferrule
{
\sorted{i}, \Delta; \Phi_a  \jasubtype{\grt}{\grt'} \\
i \not\in FV(\Phi_a)
}
{
\Delta; \Phi_a  \jasubtype{\texists{i}{\grt}}{\texists{i}{\grt'}}
}~\textbf{u-$\exists$} 
}


\newcommand{\stucimpl}
{
  \inferrule{
    \Delta; \Phi_a \wedge C' \sat C \\
    \Delta; \Phi_a  \jasubtype{\grt}{\grt'}
  }
  {
    \Delta; \Phi_a  \jasubtype{\tcimpl{C}{\grt}}{\tcimpl{C'}{\grt'}}
  }\textbf{u-c-impl}
}

\newcommand{\stucprod}
{
\inferrule{
\Delta; \Phi_a \wedge C \sat  C' \\
\Delta; \Phi_a  \jasubtype{\grt}{\grt'}
}
{
\Delta; \Phi_a  \jasubtype{\tcprod{C}{\grt}}{\tcprod{C'}{\grt'}}
}\textbf{u-c-and}
}


\newcommand{\sturefl}
{
\inferrule
{
}
{\Delta; \Phi_a  \jasubtype{\grt}{\grt}
}\textbf{u-refl}
}

\newcommand{\stutrans}
{
\inferrule{
\Delta; \Phi_a  \jasubtype{\grt_1}{\grt_2} \\
\Delta; \Phi_a  \jasubtype{\grt_2}{\grt_3} 
}
{
\Delta; \Phi_a  \jasubtype{\grt_1}{\grt_3}
}\textbf{u-tran}
}


%%% Local Variables: 
%%% mode: latex
%%% TeX-master: "main"
%%% End: 
