# Supplementary material for: Bidirectional Type Checking for Relational Properties
Source: arXiv:1812.05067 source file (2018-12-12)
Supplement: Supplementary file 31 [file subtyping-rules.tex]

\begin{figure}[t]
  \fbox{$\Delta; \Phi_a \jsubtype{\tau_1}{\tau_2}$}~~~$\Rtype$ $\tau_1$ is a subtype of $\rtype$ $\tau_2$\\
  \fbox{$\Delta; \Phi_a \jasubtype{\grt_1}{\grt_2}$}~~~$\Type$ $\grt_1$ is a subtype of $\type$ $\grt_2$\\

% The converse of the conlusion in rules marked with (*) can be proved using
% other rules (given their premises).



\raggedright
\begin{mathpar}
%
\stint
%
\and
%
\stintU
%
\and
%
\stunit
%
%
\and
% %
\starrD
%
\and
%
\starrboxD
%
\and
%
\starrW 
%
\and
%
\stforallD
%
\and
%
\stforallboxD
%
\and
%
\stforallU
%
\and
%
\sttimes
%
%
\and
%
\sttimesbox
%
\and
%
\sttimesU
%
\and
%
\stsum
%
\and
%
\stsumbox
%
\and
%
\stlist
%
\and
%
\stlistzero
%
\and
%
\stlistbox
%
\and

\end{mathpar} 
%\nocaptionrule
\caption{{\tname} subtyping rules (part 1)}
\label{fig:subtyping-rules1}  
\end{figure} 



\begin{figure}[t]
  \fbox{$\Delta; \Phi_a \jsubtype{\tau_1}{\tau_2}$}~~~Binary type $\tau_1$ is a subtype of type $\tau_2$\\

\raggedright
\begin{mathpar}
% \sttree
% %
% \and
% %
% \sttreezero
% %
% \and
% %
% \sttreebox
% %
% \and
% %
\stexists
%
\and
%
\stexistsbox
%
\and
%
\stcprod
%
\and
%
\stcprodbox
%
\and
%
\stcimpl
%
\and
%
\stcimplbox
%
\and
%
\and
%
\stbox
%
\and
%
\stboxD
%
\and
%
\stboxB
%
\and
%
\stincl
%
\and
%
\stgrt
%
\and
%
\strefl
%
\and
%
\sttrans
%
% \and
% %
% \stsplit

\end{mathpar} 
%\nocaptionrule
\caption{{\tname} subtyping rules (Part 2)}
\label{fig:subtyping-rules2}  
\end{figure} 
%%%%%%%%%%%%%%%%%%%%%%%%%%%%%%%%%%%%%%%%%%%%%%%%%%%%
% Unary subtyping
%%%%%%%%%%%%%%%%%%%%%%%%%%%%%%%%%%%%%%%%%%%%%%%%%%%%
\begin{figure}[t]
  \fbox{$\Delta; \Phi_a \jasubtype{\grt_1}{\grt_2}$}~~~ $\Type$ $\grt_1$ is a subtype of $\type$ $\grt_2$\\

\begin{mathpar}
\starrE
%
\and
%
\stforallE
%
\and
%
\stutimes
%
\and
%
\stutsum
%
\and
%
\stulist
%
\and
%
% \stutree
% %
% \and
% %
\stuexists
%
\and
%
\stucprod
%
\and
%
\stucimpl
%
\and
%
\sturefl 
%
\and
%
\stutrans
%
\end{mathpar} 
%\nocaptionrule
\caption{{\tname} unary subtyping rules}
\label{fig:subtyping-rules3}  
\end{figure} 

%%% Local Variables: 
%%% mode: latex
%%% TeX-master: "main"
%%% End: 
