# Supplementary material for: Bidirectional Type Checking for Relational Properties
Source: arXiv:1812.05067 source file (2018-12-12)
Supplement: Supplementary file 32 [file syntax.tex]

\begin{figure}
  \centering
\[
\begin{array}{llll}
 
%
  % \mbox{Costs} & k & ::= & n ~|~ k + k ~|~ \max(k_1, k_2) ~|~ \ldots \\
%
%   \mbox{Types} & \tau & ::= & \tunit ~|~ \tint ~|~ \tau_1 \ttimes \tau_2 ~|~  \tau_1 \tsum \tau_2 ~|~ % \tau_1 \tinter \tau_2 ~|~
%    \tau_1 \tarrd{t} \tau_2 ~|~ \tau_1 \uarr{k}{t} \tau_2 ~|~ \\ 
%                  &&& \tlist{n}{\alpha}{\tau} ~|~ \ttree{n}{\alpha}{\tau}  ~|~
%                      \tforalld{i}{t} \tau  ~|~ \tforall{i}{t}{t} \tau  ~|~ \texists{i} \tau ~|~  \\
%                  &&& \tcprod{C}{\tau} ~|~ \tch{\tau}  ~|~ \tbox{\tau} \\
% %

  \mbox{Relational types} & \tau & ::= & \tunit ~|~ \tint ~|~ \tau_1 \ttimes \tau_2 ~|~  \tau_1 \tsum \tau_2 ~|~ \tau_1 \tarrd{t} \tau_2 ~|~ \tlist{n}{\alpha}{\tau} ~|~ \\ 
  &&&  \tforalld{i}{t} \tau  ~|~ \texists{i} \tau ~|~ \tch{\grt_1}{\grt_2} ~|~ \tbox{\tau} ~|~ \tcprod{C}{\tau}  ~|~ \tcimpl{C}{\tau} \\\\
%
  \mbox{Unary types} & \grt & ::= & \trunit ~|~ \trint ~|~ \grt_1 \ttimes \grt_2 ~|~  \grt_1 \tsum \grt_2 ~|~ 
   \grt_1 \uarr{k}{t} \grt_2 ~|~ % \grt_1 \uarrd \grt_2 ~|~
                              \ulist{n}{\grt} ~|~ \\ 
  &&& 
      \tforall{i}{k}{t} \grt  ~|~ % \uforalld{i} \grt  ~|~
      \texists{i} \grt ~|~ \tcprod{C}{\grt}  ~|~ \tcimpl{C}{\grt}

\\[2mm]
\\
\mbox{Sorts}
 & \sort & \bnfdef &
\ssize \bnfalt
\scost%  \bnfalt  
% \svar
\\[2mm]

\mbox{Index terms} 
 & I, k, t, \alpha & \bnfdef & 
i \bnfalt
\szero \bnfalt 
\sinf \bnfalt
\splusone{I} \bnfalt
\splus{I_1}{I_2} \bnfalt
\sminus{I_1}{I_2} \bnfalt
\sdiv{I_1}{I_2} \bnfalt
\smult{I_1}{I_2} \bnfalt
\sceil{I} \bnfalt
\sfloor{I} \bnfalt
\\
& &  &
\slog{I} \bnfalt
\spower{I_1}{I_2} \bnfalt
\smin{I_1}{I_2} \bnfalt
\smax{I_1}{I_2} \bnfalt
\ssum{i}{I_1}{I_n}{I}%  \bnfalt
% \scond{C}{I_1}{I_2} 

\\[2mm]


\mbox{Constraints}
& C & \bnfdef &
\ceq{I_1}{I_2} \bnfalt
\clt{I_1}{I_2} \bnfalt
\cneg{C} \bnfalt
% \cfalse{} \bnfalt
% \cand{C_1}{C_2} \bnfalt
% \cor{C_1}{C_2}
\\[2mm]

\mbox{Constraint env.}
& \Phi & \bnfdef &
\ctrue \bnfalt
\cand{C}{\Phi}
\\
\\[2mm]

\mbox{Sort env.}
& \Delta & \bnfdef &
\emptyset \bnfalt
\Delta, i :: S 

  \\[2mm]
  \mbox{Unary type env.}
                 & \Omega & \bnfdef &
                                      \emptyset \bnfalt
                                      \Omega, x : {\grt} 
  \\[2mm]

\mbox{Relational type env.}
& \Gamma & \bnfdef &
\emptyset \bnfalt
\Gamma, x : {\tau} 
\\[2mm]

\mbox{Primitive env.}
& \primctx & \bnfdef &
\emptyset \bnfalt
\primctx, \zeta: \tau_1 \tarrd{t} \tau_2 \bnfalt
\primctx, \zeta: \grt_1 \uarr{k}{t} \grt_2
\\
%
  \\ 
%
  \mbox{{\tname} typing judg.}
  & & & \Omega  \jtype{k}{t}{e}{\grt} \\
  & & & \Gamma \jtypediff{t}{e_1}{e_2}{\tau} \\
  \\
  \mbox{{\tnamemin} typing judg.}
  & & & \Omega  \jtypeM{k}{t}{e}{\grt} \\
  & & & \Gamma \jtypediffM{t}{e_1}{e_2}{\tau} \\
  
\end{array}
\]
  \caption{Syntax of types and contexts}
\end{figure}


\begin{figure}
  \centering
\[
\begin{array}{llll}
  \mbox{Terms} & e & ::= & x  ~|~ \econst ~|~ \efix f(x). e ~|~ e_1 \eapp e_2 ~|~ \zeta \eapp e ~|~ \la e_1, e_2 \ra ~|~ \eleft(e) ~|~ \eright(e) ~|~  
  \\   &  & &  
              \einl e ~|~ \einr e ~|~ \ecase (e, x.e_1, y.e_2)   ~|~
              \enil ~|~ \econs(e_1,e_2) ~|~  \\   &  & & \ecase e \eof \enil \rightarrow e_1 ~|~ h ::tl \rightarrow e_2  ~|~  \eLam. e ~|~ e \eApp ~|~ \\  & & & 
\epack e ~|~ \eunpack e_1 \eas x \ein e_2 ~|~ \elet x = e_1 \ein e_2  ~|~  \eunit ~|~  \\ & & & 
\clet e_1 \eas x \ein e_2  ~|~ \ecelim e \\
               % 
\\
  \mbox{Values} & v & ::= & \econst ~|~ \efix f(x).v ~|~ \la  v_1, v_2 \ra ~|~ \einl v ~|~ \einr v
  ~|~ \enil ~|~ \econs(v_1,v_2) ~|~ \eLam e ~|~ \epack
  v ~|~ \eunit 
\end{array}
\]
  \caption{Syntax of values and expressions in {\tname}} 
  
\end{figure}


\begin{figure}
  \centering
\[
\begin{array}{llll}
  \mbox{Terms} & e & ::= & x  ~|~ \econst ~|~ \efix f(x). e ~|~ \efixNC f(x). e ~|~ e_1 \eapp e_2 ~|~ \zeta \eapp e ~|~ \la e_1, e_2 \ra ~|~ \eleft(e) ~|~ \eright(e) ~|~  
  \\   &  & &  
              \einl e ~|~ \einr e ~|~ \ecase (e, x.e_1, y.e_2)   ~|~
              \enil ~|~ \econsNC(e_1,e_2) ~|~ \econsC(e_1,e_2) ~|~  \\   &  & & \ecase e \eof \enil \rightarrow e_1 ~|~ h ::_{NC} tl \rightarrow e_2 ~|~ h ::_{C} tl \rightarrow e_3  ~|~  \eLam i. e ~|~ e \, [I] ~|~ \\  & & & 
\epack e \ewith I ~|~ \eunpack e_1 \eas (x, i) \ein e_2 ~|~ \elet x = e_1 \ein e_2  ~|~  \eunit ~|~  \\ & & & 
\clet e_1 \eas x \ein e_2  ~|~ \ecelim e ~|~ \eder e ~|~ \eswitch e ~|~ \enoch e ~|~ \esplit(e_1,e_2) \ewith C ~|~ \econtra e\\
               % 
\\
  \mbox{Values} & v & ::= & \econst ~|~ \efix f(x).e ~|~  \efixNC f(x).e ~|~ \la  v_1, v_2 \ra ~|~ \einl v ~|~ \einr v
                            ~|~ \enil \\
  &&& ~|~ \econsNC(v_1,v_2) ~|~ \econsC(v_1,v_2) ~|~ \eLam i. e ~|~ \epack v \ewith I  ~|~ \eunit 
\end{array}
\]
  \caption{Syntax of values and expressions in {\tnamemin}} 
  
\end{figure}



\begin{figure}
  \centering
\[
\begin{array}{llll}
  \mbox{Terms} & e & ::= & x  ~|~ \econst ~|~ \efix f(x). e ~|~ \efixNC f(x). e ~|~ e_1 \eapp e_2 ~|~ \zeta \eapp e ~|~ \la e_1, e_2 \ra ~|~ \eleft(e) ~|~ \eright(e) ~|~  
  \\   &  & &  
              \einl e ~|~ \einr e ~|~ \ecase (e, x.e_1, y.e_2)   ~|~
              \enil ~|~ \econsNC(e_1,e_2) ~|~ \econsC(e_1,e_2) ~|~  \\   &  & & \ecase e \eof \enil \rightarrow e_1 ~|~ h ::_{NC} tl \rightarrow e_2 ~|~ h ::_{C} tl \rightarrow e_3  ~|~  \eLam i. e ~|~ e \, [I] ~|~ \\  & & & 
\epack e \ewith I ~|~ \eunpack e_1 \eas (x, i) \ein e_2 ~|~ \elet x = e_1 \ein e_2  ~|~  \eunit ~|~  \\ & & & 
\clet e_1 \eas x \ein e_2  ~|~ \ecelim e ~|~ \eder ~|~ \eswitch e ~|~ \enoch e ~|~ \esplit(e_1,e_2) \ewith C ~|~  \\
  &&&\econtra e ~|~ \eannobi{e}{\tau}{t} ~|~ \eanno{e}{\grt}{k}{t}\\
               % 
\\
  \mbox{Values} & v & ::= & \econst ~|~ \efix f(x).e ~|~  \efixNC f(x).e ~|~ \la  v_1, v_2 \ra ~|~ \einl v ~|~ \einr v
                            ~|~ \enil \\
  &&& ~|~ \econsNC(v_1,v_2) ~|~ \econsC(v_1,v_2) ~|~ \eLam i. e ~|~ \epack v \ewith I  ~|~ \eunit  
\end{array}
\]
  \caption{Syntax of values and expressions in {\bitname}} 
  
\end{figure}




%%% Local Variables:
%%% mode: latex
%%% TeX-master: "main"
%%% End: 
