# Supplementary material for: Bidirectional Type Checking for Relational Properties
Source: arXiv:1812.05067 source file (2018-12-12)
Supplement: Supplementary file 33 [file ty-anno-erasure.tex]

\begin{figure*}
  \centering
  \vspace{-1ex}
  \raggedright
  \[\begin{array}{ lc  l} 
      \erty{.} &:& \text{Expression}   \to \text{Expression}   \\\\
      \erty{\kw{n}} &=& \kw{n} \\
      \erty{()} &=& () \\
      \erty{x} &=& x \\
      \erty{\efix f(x). e} &=& \efix f(x). \erty{e} \\
      \erty{\efixNC f(x). e} &=& \efixNC f(x). \erty{e} \\
      \erty{e_1 \eapp e_2} &=& \erty{e_1} \eapp \erty{e_2} \\
      \vdots &&\\
      \erty{\eanno{e}{\grt}{k}{t}} &=& \erty{e} \\
      \erty{\eannobi{e}{\tau}{t}} &=& \erty{e} \\
    \end{array}\]

  \caption{Annotation erasure}
  \label{fig:ty-annot-erasure}
  
\end{figure*}

%%% Local Variables:
%%% mode: latex
%%% TeX-master: "main"
%%% End:
