# Supplementary material for: Bidirectional Type Checking for Relational Properties
Source: arXiv:1812.05067 source file (2018-12-12)
Supplement: Supplementary file 34 [file type-eq-rules.tex]

\begin{figure*}
  \fbox{$\Delta; \Phi_a \jeqtype{\tau_1}{\tau_2}$}~~~checks whether $\tau_1$ is equivalent to $\tau_2$

\raggedright
\begin{mathpar}
\etint
%
\and
%
\etunit
%
\and
%
\etfun
%
\and
%
\etprod
%
\and
%
\etsum
%
\and
%
\etlist
%
\and
%
\etforall
%
\and
%
\etexists
%
\and
%
\etboxB
%
\and
%
\etunrel
%
\and
%
\etcimpl
%
\and
%
\etcprod
\end{mathpar} 
%\nocaptionrule
\caption{{\tnamemin} binary type equivalence rules}
\label{fig:binary-eq-rules}  
\end{figure*}



%%% Local Variables:
%%% mode: latex
%%% TeX-master: "main"
%%% End:
