# Supplementary material for: Bidirectional Type Checking for Relational Properties
Source: arXiv:1812.05067 source file (2018-12-12)
Supplement: Supplementary file 35 [file types-wf.tex]

\begin{figure*}
  \fbox{$\Delta;  \Phi_a  \algwfa{\grt}$} checks well-formedness of the unary type $\grt$ \\
  \fbox{$\Delta;  \Phi_a \algwf{\tau}$} checks
  well-formedness of the binary type $\tau$  \vspace{-1ex} \raggedright
\begin{smathpar}

\inferrule
{
  \strut 
}
{
   \Delta;  \Phi_a \algwf{\trunit}
}~ \textbf{wf-unit}
%
\and
%
\inferrule
{ 
  \strut
}
{
   \Delta; \psi; \Phi_a \algwf{\trint}
}~ \textbf{wf-int}
%
\and
%
\inferrule
{ 
    \Delta; \psi; \Phi_a \algwf{\tau_1} \\
    \Delta; \psi; \Phi_a \algwf{\tau_2}
}
{
   \Delta; \psi; \Phi_a \algwf{\tau_1 \ttimes \tau_2}
}~ \textbf{wf-prod}
%
\and
%
\inferrule
{ 
    \Delta; \psi; \Phi_a \algwf{\tau_1} \\
    \Delta; \psi; \Phi_a \algwf{\tau_2}
}
{
   \Delta; \psi; \Phi_a \algwf{\tau_1 \tsum \tau_2}
}~ \textbf{wf-sum}
%
\and
%
\inferrule
{ 
    \Delta; \psi; \Phi_a \algwf{\tau_1} \\
    \Delta; \psi; \Phi_a \algwf{\tau_2} \\
    \Delta; \Phi_a \sty{t}{\scost}
}
{
   \Delta;  \Phi_a \algwf{ \tau_1 \tarrd{t} \tau_2}
}~ \textbf{wf-fun} 
%
\and
%
\inferrule
{ 
   \Delta,  \Phi_a \sty{n}{\ssize} \\
   \Delta,  \Phi_a \sty{\alpha}{\ssize} \\
   \Delta;  \Phi_a \algwf{\tau}
}
{
   \Delta;  \Phi_a \algwf{\tlist{n}{\alpha}{\tau}}
}~ \textbf{wf-list} 
%
\and
%
\inferrule
{ 
    \sorted{i},  \Delta; \Phi_a \algwf{\tau} \\
   \sorted{i},  \Delta; \Phi_a \sty{t}{\scost}
}
{
   \Delta;  \Phi_a \algwf{\tforalld{i}{t} \tau}
}~ \textbf{wf-$\forall$}  
%
\and
%
\inferrule
{
    \sorted{i},  \Delta; \Phi_a \algwf{\tau}{\Phi}
}
{
   \Delta;  \Phi_a \algwf{\texists{i}{\tau}}{\Phi}
}~ \textbf{wf-$\exists$}
%
\and
%
\inferrule
{ 
   \Delta; \psi; \Phi_a \algwfa{\grt_1} \\
   \Delta; \psi; \Phi_a \algwfa{\grt_2}
}
{
   \Delta; \psi; \Phi_a \algwf{\tch{\grt_1}{\grt_2}}
}~ \textbf{wf-$\achange$}
%
\and
%
\inferrule
{ 
   \Delta; \psi; \Phi_a \algwf{\tau}
}
{
   \Delta; \psi; \Phi_a \algwf{\tbox{\tau}}
}~ \textbf{wf-box}
%
\and
%
\inferrule
{
   \Delta;  \Phi_a \wf{C}\\
   \Delta;  \cand{C}{\Phi_a} \algwf{\tau}
}
{
   \Delta;  \Phi_a \algwf{\tcimpl{C}{\tau}}
}~ \textbf{wf-C$\mathrel{\supset}$}
%
\and
%
\inferrule
{
   \Delta;  \Phi_a \wf{C}\\
   \Delta;  \Phi_a \algwf{\tau}
}
{
   \Delta;  \Phi_a \algwf{\tcprod{C}{\tau}}
}~ \textbf{wf-C$\mathrel{\&}$}

\end{smathpar}
%\nocaptionrule
\caption{Well-formedness of binary types}
\label{fig:type-wf}
\end{figure*}  




\begin{figure*}
  \fbox{$ \Delta\algwfa{\grt}$} checks
  well-formedness of the unary type $\grt$
  $\Phi$ \vspace{-1ex} \raggedright
\begin{smathpar}

\inferrule
{
  \strut
}
{
   \Delta;  \Phi_a \algwfa{\tunit}
}~ \textbf{wf-u-unit}
%
\and
%
\inferrule
{ 
  \strut
}
{
   \Delta; \psi; \Phi_a \algwfa{\tint}
}~ \textbf{wf-u-int}
%
\and
%
\inferrule
{ 
    \Delta; \psi; \Phi_a \algwfa{\grt_1} \\
    \Delta; \psi; \Phi_a \algwfa{\grt_2}
}
{
   \Delta; \psi; \Phi_a \algwfa{\grt_1 \ttimes \grt_2}
}~ \textbf{wf-u-prod}
%
\and
%
\inferrule
{ 
    \Delta; \psi; \Phi_a \algwfa{\grt_1}\\
    \Delta; \psi; \Phi_a \algwfa{\grt_2}
}
{
   \Delta; \psi; \Phi_a \algwfa{\grt_1 \tsum \grt_2}
}~ \textbf{wf-u-sum}
%
\and
%
\inferrule
{ 
    \Delta; \psi; \Phi_a \algwfa{\grt_1} \\
    \Delta; \psi; \Phi_a \algwfa{\grt_2}\\
    \Delta; \Phi_a \sty{k}{\scost} \\
    \Delta; \Phi_a \sty{t}{\scost}
}
{
   \Delta;  \Phi_a \algwfa{ \grt_1 \uarr{k}{t} \grt_2}
}~ \textbf{wf-u-fun} 
%
\and
%
\inferrule
{ 
   \Delta,  \Phi_a \sty{n}{\ssize} \\
   \Delta;  \Phi_a \algwfa{\grt}
}
{
   \Delta;  \Phi_a \algwfa{\ulist{n}{\grt}}
}~ \textbf{wf-u-list} 
%
\and
%
\inferrule
{ 
    \sorted{i},  \Delta; \Phi_a \algwfa{\grt} \\
   \sorted{i},  \Delta; \Phi_a \sty{k}{\scost} \\
   \sorted{i},  \Delta; \Phi_a \sty{t}{\scost}
}
{
   \Delta;  \Phi_a \algwfa{\tforall{i}{k}{t} \grt}
}~ \textbf{wf-u-$\forall$}  
%
\and
%
\inferrule
{
    \sorted{i},  \Delta; \Phi_a \algwfa{\grt}
}
{
   \Delta;  \Phi_a \algwfa{\texists{i}{\grt}}
}~ \textbf{wf-u-$\exists$}
%
\and
%
\inferrule
{
   \Delta;  \Phi_a \wf{C}\\
   \Delta;  \cand{C}{\Phi_a} \algwfa{\grt}
}
{
   \Delta;  \Phi_a \algwfa{\tcimpl{C}{\grt}}
}~ \textbf{wf-u-C$\ra$}
%
\and
%
\inferrule
{
   \Delta;  \Phi_a \wf{C}\\
   \Delta;  \Phi_a \algwfa{\grt}
}
{
   \Delta;  \Phi_a \algwfa{\tcprod{C}{\grt}}
}~ \textbf{wf-u-C$\wedge$}

\end{smathpar}
%\nocaptionrule
\caption{Well-formedness of unary types}
\label{fig:utype-wf}
\end{figure*}  



%%% Local Variables: 
%%% mode: latex
%%% TeX-master: "main"
%%% End: 
 
