# Supplementary material for: Bidirectional Type Checking for Relational Properties
Source: arXiv:1812.05067 source file (2018-12-12)
Supplement: Supplementary file 36 [file typing-rules-defs.tex]

\newcommandx{\tyswitch}[2][1=,2=]
{
    \inferrule{
    \Delta; \Phi_a; \trm{\Gamma}{1} \jtype{k_1}{t_1}{e_1}{\grt_1}~~#1\\
    \Delta; \Phi_a; \trm{\Gamma}{2} \jtype{k_2}{t_2}{e_2}{\grt_2}~~#2
    } {\ctx \jtypediff{t_1-k_2}{e_1}{e_2}{\tch{\grt_1}{\grt_2}}}~\textbf{switch}
}
 


\newcommandx{\tynochange}[2][1=,2=]
{
  \inferrule
{
\Delta; \Phi_a; \Gamma \jtypediff{t}{e}{e}{\tau}~~#1\\\\
\forall x \in dom(\Gamma).~~
\Delta; \Phi_a  \jsubtype{\Gamma(x)}{\tbox{\Gamma(x)}} ~~#2
}
{
\Delta; \Phi_a; \Gamma, \Gamma'; \Omega \jtypediff{0}{e}{e}{\tbox{\tau}}
} ~\textbf{nochange}
}



\newcommand{\tyconst}
{
  \inferrule
  {
  }
  {
    \octx \jtype{0}{0}{\econst}{\tint}
  }~\textbf{const}
}

\newcommand{\tyrconst}
{
  \inferrule
  {
  }
  {
    \ctx \jtypediff{0}{\econst}{\econst}{\trint}
  }~\textbf{r-const}
}


\newcommand{\tyunit}
{
  \inferrule
  {
  }
  {
    \octx \jtype{0}{0}{{\eunit}}{\tunit}
  }~\textbf{unit}
}

\newcommand{\tyrunit}
{
  \inferrule
  {
  }
  {
    \ctx \jtypediff{0}{\eunit}{\eunit}{\trunit}
  }~\textbf{r-unit}
}



\newcommand{\tyelimU}
{\inferrule{
  \octx \jtype{k_1}{t_1}{e_1}{\grt_1}\\
  \Delta; \Phi_a;  x: \grt_1 , \Omega \jtype{k_2}{t_2}{e_2}{\grt_2}
}
{ \octx \jtype{k_1+k_2}{t_1+t_2}{\eelimU x = e_1 \ein e_2}{
  \grt_2} }~\textbf{elimU}
}


\newcommand{\tyrelimU}
{\inferrule{
  \ctx \jtypediff{t_1}{e_1}{e_1'}{\tch{\grt_1}{\grt_1'}}\\
  \Delta; \Phi_a; \Gamma;  x: \grt_1, \Omega \jtypediff{t_2}{e_2}{e_2'}{\tau_2}
}
{  \ctx \jtypediff{t_1+t_2}{\eelimU x = e_1 \ein e_2}{ \eelimU x = e_1' \ein e_2'}{
  \tau_2} }~\textbf{r-elimU}
}



\newcommand{\tyvar}
{  \inferrule{\Omega(x) = \grt }{\octx \jtype{0}{0}{x}{\grt}}~\textbf{var}
}

\newcommand{\tyrvar}{
  \inferrule{\Gamma(x) = \tau}{\ctx \jtypediff{0}{x}{x}{\tau}}~\textbf{r-var}
}


\newcommand{\tyinl}
{
  \inferrule
  {
    \octx  \jtype{k}{t}{e}{\grt_1}\\
    {\ifextra
    \Delta; \Phi_a \awfty{\grt_2}
    \fi}
  }
  { \octx  \jtype{k}{t}{\einl e}{\grt_1+ \grt_2}
  }~\textbf{inl}
}
\newcommand{\tyrinl}
{  \inferrule
  {
    \ctx  \jtypediff{t}{e}{e'}{\tau_1}\\
    {
     \ifextra
     \Delta; \Phi_a \wfty{\tau_2}
     \fi
   }
  }
  { \ctx  \jtypediff{t}{\einl e}{\einl e'}{\tau_1 + \tau_2}
  }~\textbf{r-inl}
}


\newcommand{\tyinr}
{
  \inferrule
  {
    \octx  \jtype{k}{t}{e}{\grt_2}\\
    \Delta; \Phi_a \awfty{\grt_1}
  }
  { \octx  \jtype{k}{t}{\einr e}{\grt_1 + \grt_2}
  }~\textbf{inr}
}
\newcommand{\tyrinr}
{  \inferrule
  {
    \ctx  \jtypediff{t}{e}{e'}{\tau_2}\\
    \Delta; \Phi_a \wfty{\tau_1}
  }
  { \ctx  \jtypediff{t}{\einr e}{\einr e'}{\tau_1 + \tau_2}
  }~\textbf{r-inr}
}

\newcommand{\tycase}
{  \inferrule{\octx \jtype{k}{t}{e}{\grt_1 + \grt_2} \\
    \Delta; \Phi_a;  x: \grt_1, \Omega \jtype{k'}{t'}{e_1}{\grt} \\
    \Delta; \Phi_a;  y: \grt_2, \Omega \jtype{k'}{t'}{e_2}{\grt}}
  {\octx \jtype{k+k'+\kcase}{t+t'+\kcase}{\ecase(e, x.e_1, y.e_2)}{\grt}}~\textbf{case}
}
%
\newcommand{\tyrcase}
{  \inferrule{
    \ctx \jtypediff{t}{e}{e'}{\tau_1 + \tau_2}\\
    \Delta; \Phi_a; x: \tau_1, \Gamma \jtypediff{t'}{e_1}{e_1'}{\tau}\\
    \Delta; \Phi_a; y: \tau_2, \Gamma  \jtypediff{t'}{e_2}{e_2'}{\tau}
}{\ctx \jtypediff{t+t'}{
    \ecase(e, x.e_1, y.e_2)}{\ecase(e', x.e_1', y.e_2')}{\tau}}~\textbf{r-case}}
%



\newcommand{\tyfix}
{  \inferrule{
    {\ifextra
    \Delta; \Phi_a \awfty{\grt_1 \uarr{k}{t} \grt_2} 
    \fi} \\
    \Delta; \Phi_a;  x: \grt_1, f : \grt_1 \uarr{k}{t}
    \grt_2, \Omega  \jtype{k}{t}{e}{\grt_2}}
  {
    \octx
    \jtype{0}{0}{ \efix f(x).e}{\grt_1 \uarr{k}{t}
    \grt_2}
}~\textbf{fix}
}




%
\newcommand{\tyrfix}
{  \inferrule{
       {\ifextra
       \Delta; \Phi_a \wfty{\tau_1 \tarrd{t} \tau_2}  
       \fi} \\
       \Delta; \Phi_a;  x: \tau_1, f : \tau_1 \tarrd{t} \tau_2, \Gamma  \jtypediff{t}{e_1}{e_2}{\tau_2}}
            {\ctx \jtypediff{0}{ \efix f(x).e_1}{\efix f(x).e_2}{
              \tau_1 \tarrd{t} \tau_2}}~\textbf{r-fix}}
%

\newcommandx{\tyrfixNC}[2][1=,2=]
{  \inferrule
  {
    {\ifextra \Delta; \Phi_a \wfty{\tau_1 \tarrd{t} \tau_2}
      \fi} \\
    \Delta; \Phi_a;  x: \tau_1, f : \tbox{(\tau_1 \tarrd{t} \tau_2)}, \Gamma  \jtypediff{t}{e}{e}{\tau_2}~~#1\\
    \forall x \in dom(\Gamma).~~
    \Delta; \Phi_a  \jsubtype{\Gamma(x)}{\tbox{\Gamma(x)}}~~#2
  }
  {\ctx \jtypediff{0}{ \efix f(x).e}{\efix f(x).e}{
              \tbox{(\tau_1 \tarrd{t} \tau_2)}}}~\textbf{r-fixNC}
}



\newcommand{\tyrfixE}
{  \inferrule{
    \Delta; \Phi_a; \Gamma;  x: \tau_1, f : \tau_1 \uarr{k}{t} \tau_2, \Omega  \jtype{k_1}{t_1}{e_1}{\tau_2} \\
    \Delta; \Phi_a; \Gamma;  x: \tau_1, f : \tau_1 \uarr{k}{t} \tau_2,\Omega  \jtype{k_2}{t_2}{e_2}{\tau_2}
}
{\ctx \jtypediff{0}{ \efix f(x).e_1}{\efix f(x).e_2}{
              \tau_1 \uarr{k}{t} \tau_2}}~\textbf{r-fix$\wexec$}}
%


\newcommand{\tyapp}
{\inferrule{
  \octx \jtype{k_1}{t_1}{e_1}{\grt_1\uarr{k}{t} \grt_2} \\
  \octx \jtype{k_2}{t_2}{e_2}{\grt_1}}
{
  \octx \jtype{k_1+k_2+k+\kapp}{t_1+t_2+t+\kapp}{ e_1 \eapp e_2}{
  \grt_2}}~\textbf{app}}
%
% \inferrule{\ctx \jtypemin{k_1} e_1: (\tau_1\uarr{\wmin}{k} \tau_2)^\mu
%   \\ \ctx \jtypemin{k_2} e_2: \tau_1\\ (\mu = \achange) \Rightarrow
%   (\lbound \tau_2)}{\ctx \jtypemin{k_1 + k_2 + k + 1} e_1 \eapp e_2: \tau_2} \and
% %
 


\newcommand{\tyrappD}
{\inferrule{\ctx \jtypediff{t_1}{e_1}{e_1'}{\tau_1}
  \tarrd{t} \tau_2 \\\\
 \ctx \jtypediff{t_2}{ e_2}{e_2'}{\tau_1}}
{\ctx \jtypediff{t_1+t_2+t}{e_1 \eapp e_2}{e_1' \eapp e_2'}{\tau_2}}~\textbf{r-app}}



\newcommand{\tyiLam}
{  \inferrule{
    i::S, \octx \jtype{k}{t}{e}{\grt}\\
    i \not \in \fiv{\Phi_a; \Omega}
  }
  { \octx \jtype{0}{0}{\eLam e}{\tforall{i}{k}{t} \grt}}~\textbf{iLam }}
%
\newcommandx{\tyriLam}[2][1=,2=]
{ \inferrule{
    i::S, \ctx \jtypediff{t}{e}{e'}{\tau}~~#1 \\
    i \not \in \fiv{\Phi_a; \Gamma} 
  }
  { \ctx \jtypediff{0}{\eLam e}{\eLam e'}{\tforalld{i}{t} \tau}}~\textbf{r-iLam}}
%
\newcommand{\tyriLamc}
{  \inferrule{
    i::S, \ctx \jtype{k}{t}{e}{\tau} \\
    i::S, \ctx \jtype{k}{t}{e'}{\tau} \\
  }
  { \ctx \jtypediff{0}{\eLam e}{\eLam e'}{\tforall{i}{k}{t} \tau}}~\textbf{r-iLam2}
}

\newcommand{\tyiApp}
{  \inferrule{
    \octx \jtype{k}{t}{e}{\tforall{i}{k'}{t'} \grt} \\
    \Delta \vdash I : S
  }
  {\octx \jtype{k+k'[I/i]}{t+t'[I/i]}{e \eApp}{\grt\{ I/ i\}}}~\textbf{iApp}}
%
\newcommandx{\tyriApp}[2][1=,2=]
{  \inferrule{
    \ctx \jtypediff{t}{e}{e'}{\tforalld{i}{t'} \tau} ~~#1\\
    \Delta \vdash I : S ~~#2
  }
  {\ctx \jtypediff{t+t'[I/i]}{e \eApp}{e' \eApp}{\tau\{ I/ i\}}}~\textbf{r-iApp}}
%

\newcommand{\typack}
{
\inferrule
{
  \octx  \jtype{k}{t}{e}{\grt\{I/i\}} \\
  \Delta \sty{I}{\sort}
}
{
  \octx  \jtype{k}{t}{\epack e}{\texists{i} \grt}
} ~\textbf{pack}
}

\newcommandx{\tyrpack}[2][1=,2=]
{
\inferrule
{
  \ctx  \jtypediff{t}{e}{e'}{\tau\{I/i\}}~~#1\\
  \Delta \sty{I}{\sort}~~#2
}
{
  \ctx  \jtypediff{t}{\epack e}{\epack e'}{\texists{i} \tau}
} ~\textbf{r-pack}
}

\newcommand{\tyunpack}{
\inferrule
{
  \octx \jtype{k_1}{t_1}{e_1}{\texists{i} \grt_1} \\
  \sorted{i}, \Delta; \Phi_a;  x: \grt_1, \Omega \jtype{k_2}{t_2}{e_2}{\grt_2} \\
  i \not\in FV(\Phi_a;\Gamma, \grt_2, k_2, t_2) \\
}
{
  \octx  \jtype{k_1+k_2}{t_1+t_2}{\eunpack e_1 \eas x \ein  e_2}{\grt_2}
}~\textbf{unpack}
}


\newcommandx{\tyrunpackD}[2][1=,2=]
{
\inferrule
{
  \ctx \jtypediff{t_1}{e_1}{e_1'}{\texists{i} \tau_1} ~~#1\\
  \sorted{i}, \Delta; \Phi_a; x: \tau_1, \Gamma \jtypediff{t_2}{e_2}{e_2'}{\tau_2} ~~#2\\
  i \not\in FV(\Phi_a;\Gamma, \tau_2, t_2) \\
}
{
  \ctx  \jtypediff{t_1+t_2}{\eunpack e_1 \eas x \ein  e_2}{\eunpack e_1' \eas x \ein  e_2'}{\tau_2}
}~\textbf{r-unpack1}}


\newcommand{\tynil}
{ \inferrule
  {
    {\ifextra
      \Delta; \Phi_a \awfty{\grt}
    \fi}
  }
  { \octx \jtype{0}{0}{\enil}{\ulist{0}{\grt}}
}~\textbf{nil}}
%
\newcommand{\tyrnil}
{  \inferrule
  {
    \Delta; \Phi_a \wfty{\tau}
  }
  { \ctx \jtypediff{0}{\enil}{\enil}{\tlist{0}{\alpha}{\tau}}}~\textbf{r-nil}
}

\newcommand{\tycons}
{  \inferrule
  { \octx \jtype{k_1}{t_1}{e_1}{\grt} \\
    \octx \jtype{k_2}{t_2}{e_2}{\ulist{n}{\grt}}
  }
  { \octx \jtype{k_1+k_2}{t_1+t_2}{\econs(e_1,e_2)}{\ulist{n+1}{\grt}}}~\textbf{cons}}
%
\newcommand{\tyrcons}
{   \inferrule
  { \ctx \jtypediff{t_1}{e_1}{e_1'}{\tau} \\
    \ctx \jtypediff{t_2}{e_2}{e_2'}{\tlist{n}{\alpha}{\tau}}
  }
  { \ctx \jtypediff{t_1+t_2}{ \econs(e_1,e_2) }{ \econs(e_1',e_2')}{\tlist{n+1}{\alpha+1}{\tau}}}~\textbf{r-cons1}}
%
\newcommand{\tyrconsbox}
{   \inferrule
  { \ctx \jtypediff{t_1}{e_1}{e_1'}{\tbox{\tau}} \\
    \ctx \jtypediff{t_2}{e_2}{e_2'}{\tlist{n}{\alpha}{\tau}}}
  { \ctx \jtypediff{t_1+t_2}{ \econs(e_1,e_2) }{ \econs(e_1',e_2')}{\tlist{n+1}{\alpha}{\tau}}}~\textbf{r-cons2}}
%

\newcommand{\tycaseL}
 { \inferrule
  {\octx \jtype{k}{t}{e}{\ulist{n}{\grt}} \\
   \Delta; \Phi_a \wedge n = 0 ;  \Omega \jtype{k'}{t'}{e_1}{\grt'} \\
   i, \Delta; \Phi_a \wedge n = i+1 ;  h: \grt, tl : \ulist{i}{\grt}, \Omega
   \jtype{k'}{t'}{e_2}{\grt'}
  } 
  {\octx \jtype{k+k'+\kcaseL}{t+t'+\kcaseL}{ \ecase e \eof \enil \rightarrow e_1 ~|~ h::tl \rightarrow
    e_2}{\grt'}}~\textbf{caseL}
 }

\newcommandx{\tyrcaseL}[4][1=,2=,3=,4=]
{ \inferrule
  {\ctx \jtypediff{t}{e}{e'}{\tlist{n}{\alpha}{\tau}} ~~#1\\
   \Delta; \Phi_a \wedge n = 0  ;\Gamma \jtypediff{t'}{e_1}{e_1'}{\tau'} ~~#2\\
   i, \Delta; \Phi_a \wedge n = i+1;  h: \tbox{\tau},
   tl : \tlist{i}{\alpha}{\tau}, \Gamma \jtypediff{t'}{e_2}{e_2'}{\tau'} ~~#3
\\
   i, \beta, \Delta; \Phi_a \wedge n = i+1 \wedge \alpha = \beta +1 ;
   h: \tau, tl : \tlist{i}{\beta}{\tau}, \Gamma \jtypediff{t'}{e_2}{e_2'}{\tau'} ~~#4
   }
  {\ctx \jtypediff{t+t'}{ \ecase e \eof \enil \rightarrow e_1 ~|~ h::tl \rightarrow
    e_2}{\ecase e' \eof \enil \rightarrow e_1' ~|~ h::tl \rightarrow
    e_2'}{\tau'}}~\textbf{r-caseL}
}


\newcommand{\tyleaf}
 { \inferrule
  {
    \Delta; \Phi_a \awfty{\grt}
  }
  { \octx \jtype{0}{0}{\eleaf}{\utree{0}{\grt}}}~\textbf{leaf}}
%
\newcommand{\tyrleaf}
{  \inferrule
  {
    \Delta; \Phi_a \wfty{\tau}
  }
  { \ctx \jtypediff{0}{\eleaf}{\eleaf}{\ttree{0}{\alpha}{\tau}}}~\textbf{r-leaf}
}

\newcommand{\tynode}
{ \inferrule
  { \\
    \octx \jtype{k}{t}{e}{\grt} \\
    \octx \jtype{k_1}{t_1}{e_l}{\utree{i}{\grt}} \\
    \octx \jtype{k_2}{t_2}{e_r}{\utree{j}{\grt}} 
  }
  { \octx \jtype{k+k_1+k_2}{t+t_1+t_2}{\enode(e_l,e,e_r)}{\utree{i+j+1}{\grt}}}~\textbf{node}
}
%

\newcommand{\tyrnode}
{   \inferrule
  { \\
    \ctx \jtypediff{t}{e}{e'}{\tau}\\
    \ctx \jtypediff{t_1}{e_l}{e_l'}{\ttree{i}{\alpha}{\tau}}\\
    \ctx \jtypediff{t_2}{e_r}{e_r'}{\ttree{j}{\beta}{\tau} }}
  { \ctx \jtypediff{t+t_1+t_2}{\enode(e_l,e,e_r)}{\enode(e_l',e',e_r')}{\ttree{i+j+1}{\alpha+\beta+1}{\tau}}}~\textbf{r-node1}
}

\newcommand{\tyrnodeb}
{   \inferrule
  { \\
    \ctx \jtypediff{t}{e}{e'}{\tbox{\tau}}\\
    \ctx \jtypediff{t_1}{e_l}{e_l'}{\ttree{i}{\alpha}{\tau}}\\
    \ctx \jtypediff{t_2}{e_r}{e_r'}{\ttree{j}{\beta}{\tau} }}
  { \ctx \jtypediff{t+t_1+t_2}{\enode(e_l,e,e_r)}{\enode(e_l',e',e_r')}{\ttree{i+j+1}{\alpha+\beta}{\tau}}}~\textbf{r-node2}
}



\newcommand{\tycaseT}
{  \inferrule
  {\octx \jtype{k}{t}{e}{\utree{n}{\grt}} \\
   \Delta; \Phi_a \wedge n = 0 ; \Omega \jtype{k'}{t'}{e_1}{\grt'} \\
   i, j, \Delta; \Phi_a \wedge n = i+j+1;  x: \grt, l : \utree{i}{\grt}, r : \utree{j}{\grt}, \Omega \jtype{k'}{t'}{e_2}{\grt'}
   }
  {\octx \jtype{k+k'+\kcaseT}{t+t'+\kcaseT}{\ecase e \eof \eleaf \rightarrow e_1 ~|~ \enode(l,x,r) \rightarrow
    e_2}{\grt'}}~\textbf{caseT}
}
 %
\newcommand{\tyrcaseT}
{ \inferrule
  {\ctx \jtypediff{t}{e}{e'}{\ttree{n}{\alpha}{\tau}}\\
   \Delta; \Phi_a \wedge n = 0  \wedge  ; \Gamma \jtypediff{t'}{e_1}{e_1'}{\tau'}\\
   i,j, \beta, \theta, \Delta; \Phi_a \wedge n = i+j+1 \wedge \alpha = \beta + \theta ;  x: \tbox{\tau}, l : \ttree{i}{\beta}{\tau}, r : \ttree{j}{\theta}{\tau}, \Gamma \jtypediff{t'}{ e_2}{e_2'}{\tau'} \\
     i,j, \beta, \theta, \Delta; \Phi_a \wedge n = i+j+1 \wedge \alpha = \beta + \theta +1;  x: \tau, l : \ttree{i}{\beta}{\tau}, r : \ttree{j}{\theta}{\tau}, \Gamma  \jtypediff{t'}{e_2}{e_2'}{\tau'}
   }
  {\ctx \jtypediff{t+t'}{\ecase e \eof \eleaf \rightarrow e_1 ~|~ \enode(l,x,r) \rightarrow
    e_2}{\ecase e' \eof \eleaf \rightarrow e_1' ~|~ \enode(l,x,r) \rightarrow}{e_2'}{\tau'}}~\textbf{r-caseT}
}

\newcommand{\typrod}
{\inferrule{
    \octx \jtype{k_1}{t_1}{e_1}{\grt_1} \\
    \octx \jtype{k_2}{t_2}{e_2}{\grt_2}}
  {
    \octx \jtype{k_1+k_2}{t_1+t_2}{\la e_1, e_2 \ra}{\grt_1
  \ttimes \grt_2}}~\textbf{prod}
}


\newcommand{\tyrprod}
{\inferrule{\ctx \jtypediff{t_1}{e_1}{e_1'}{\tau_1}\\ \ctx
  \jtypediff{t_2}{ e_2}{e_2'}{\tau_2}
}
{
  \ctx 
  \jtypediff{t_1+t_2}{\la e_1, e_2 \ra}{\la e_1' , e_2' \ra}{\tau_1 \ttimes \tau_2}
}~\textbf{r-prod}
}

\newcommand{\typroj}
{\inferrule{\octx \jtype{k}{t}{e}{\grt_1 \ttimes \grt_2}}
  {\octx
  \jtype{k+\kproj}{t+\kproj}{\eleft(e)}{\grt_1}}~\textbf{proj1}}

\newcommand{\tyrproj}
{\inferrule{
    \ctx \jtypediff{t}{e}{e'}{\tau_1 \ttimes\tau_2}
}
{\ctx \jtypediff{t}{ \eleft(e)}{\eleft(e')}{\tau_1}}~\textbf{r-proj1}
}



\newcommand{\tylet}
{\inferrule{
  \octx \jtype{k_1}{t_1}{e_1}{\grt_1} \\
  \Delta;\Phi_a;  x: \grt_1 , \Omega \jtype{k_2}{t_2}{e_2}{\grt_2}
}
{ \octx \jtype{k_1+k_2+\klet}{t_1+t_2+\klet}{\elet x = e_1 \ein e_2}{
  \grt_2}
}~\textbf{let}}
%
\newcommand{\tyrlet}
{\inferrule{
  \ctx \jtypediff{t_1}{e_1}{e_1'}{\tau_1}\\
  \Delta; \Phi_a; x: \tau_1, \Gamma  \jtypediff{t_2}{e_2}{e_2'}{\tau_2}
}
{ \ctx \jtypediff{t_1+t_2}{ \elet x = e_1 \ein e_2 }{\elet x = e_1' \ein e_2'}{
  \tau_2} }~\textbf{r-let1}
}


\newcommand{\tycandIntro}
{\inferrule
{
\Delta; \Phi_a \sat C \\
  \Delta; \Phi_a \wedge C;  \Omega \jtype{k}{t}{e}{\grt}
}
{
  \octx \jtype{k}{t}{e}{\tcprod{C}{\grt}}
} ~\textbf{c-andI}
}

\newcommand{\tyrcandIntro}
{\inferrule
{
\Delta; \Phi_a \sat C \\
  \Delta; \Phi_a \wedge C; \Gamma  \jtypediff{t}{e}{e'}{\tau}
}
{
  \ctx  \jtypediff{t}{e}{e'}{\tcprod{C}{\tau}}
} ~\textbf{c-andI}
}

\newcommand{\tycandElim}
{
\inferrule
{
  \octx \jtype{k_1}{t_1}{e_1}{\tcprod{C}{\grt_1}} \\
  \Delta; \Phi_a \wedge C;   x :\grt_1,  \Omega  \jtype{k_2}{t_2}{ e_2}{\grt_2} \\
}
{
  \octx  \jtype{k_1+k_2}{t_1+t_2}{\clet e_1 \eas x \ein e_2}{\grt_2}
} ~\textbf{c-andE}
}

\newcommand{\tyrcandElimD}
{
\inferrule
{
  \ctx \jtypediff{t_1}{e_1}{e_1 '}{\tcprod{C}{\tau_1}}\\
  \Delta; \Phi_a \wedge C; x :\tau_1, \Gamma  \jtypediff{t_2}{ e_2}{e_2'}{\tau_2}
}
{
  \ctx  \jtypediff{t_1+t_2}{\clet e_1 \eas x \ein e_2}{\clet e_1' \eas x \ein e_2'}{\tau_2}
} ~\textbf{r-c-andE}
}

\newcommand{\tycimplIntro}
{
\inferrule
{
\Delta; \Phi_a \wedge C;  \Omega  \jtype{k}{t}{e}{{\grt}}
}
{
  \octx  \jtype{k}{t}{e}{\tcimpl{C}{\grt}}
} ~\textbf{c-impI}

}

\newcommand{\tyrcimplIntro}
{
\inferrule
{
\Delta; \Phi_a \wedge C; \Gamma  \jtypediff{t}{e}{e'}{\tau}
}
{
  \ctx  \jtypediff{t}{e}{e'}{\tcimpl{C}{\tau}}
} ~\textbf{r-c-impI}
}


\newcommand{\tycimplElim}
{
\inferrule
{
  \octx  \jtype{k}{t}{e}{\tcimpl{C}{\grt}} \\
\Delta; \Phi_a \sat C
}
{
  \octx  \jtype{k}{t}{\ecelim e}{\grt}
} ~\textbf{c-implE}
}

\newcommand{\tyrcimplElimD}
{
\inferrule
{
  \ctx  \jtypediff{t}{e}{e'}{\tcimpl{C}{\tau}}\\
\Delta; \Phi_a \sat C
}
{
  \ctx  \jtypediff{t}{\ecelim e}{\ecelim  e'}{\tau}
} ~\textbf{r-c-implE}
}



\newcommand{\typrimapp}
{\inferrule{
    \primctx(\zeta) =  \grt_1 \uarr{k}{t} \grt_2  \\
  \octx \jtype{k'}{t'}{e}{\grt_1}}
{
   \octx \jtype{k+k'+\kapp}{t+t'+\kapp}{\zeta \eapp e}{\grt_2}}~\textbf{primapp}}


\newcommand{\tyrprimapp}
{\inferrule{
    \primctx(\zeta) = \tau_1 \tarrd{t} \tau_2 \\
    \ctx \jtypediff{t'}{e}{e'}{\tau_1}
}
{
 \ctx \jtypediff{t+t'}{\zeta \eapp e}{\zeta \eapp e'}{
  \tau_2}}~\textbf{r-primapp}}


\newcommand{\tyinterI}
{
   \inferrule{
    \octx \jtype{k}{t}{e}{\grt_1} \\
    \octx \jtype{k}{t}{e}{\grt_2} \\
}{
  \octx \jtype{k}{t}{e}{\grt_1 \tinter \grt_2}}~\textbf{interI}
}

\newcommand{\tyrinterI}
{
   \inferrule{
    \ctx \jtypediff{t}{e}{e'}{\tau_1}\\
    \ctx \jtypediff{t}{e}{e'}{\tau_2}\\
}{
  \ctx \jtypediff{t}{ e }{ e'}{\tau_1 \tinter \tau_2}}~\textbf{r-interI}
}


\newcommandx{\tyinterE}[1][1=i]
{
   \inferrule{
     \octx \jtype{k}{t}{e}{\grt_1 \tinter \grt_2} \\
}{
  \octx \jtype{k}{t}{e}{\grt_{#1}} }~\textbf{interE$_{#1}$}
}

\newcommandx{\tyrinterE}[1][1=i]
{
   \inferrule{
    \ctx \jtypediff{t}{e}{e'}{\tau_1 \tinter \tau_2}\\
}{
  \ctx \jtypediff{t}{ e}{e'}{\tau_{#1}} }~\textbf{r-interE$_{#1}$}
}



\newcommandx{\tysubsum}[4][1=,2=,3=,4=]
{
   \inferrule{
    \octx \jtype{k}{t}{e}{\grt} ~~#1\\
    \Delta; \Phi_a \jsubtype{\grt}{\grt'} ~~#2\\
    \Delta; \Phi_a \sat k' \leq k ~~#3\\
    \Delta; \Phi_a \sat t \leq t'~~#4
}{
  \octx \jtype{k'}{t'}{e}{\grt'}
}~{\pmb{\sqsubseteq}\wexec}
}

\newcommandx{\tyrsubsum}[3][1=,2=,3=]
{
   \inferrule{
    \ctx \jtypediff{t}{e_1}{e_2}{\tau}~~#1\\
    \Delta; \Phi_a \jsubtype{\tau}{\tau'}~~#2 \\
    \Delta; \Phi_a \sat t \leq t'~~#3
  }
  {\ctx \jtypediff{t'}{e_1}{e_2}{\tau'} }~{\textbf{r-}\pmb{\sqsubseteq}}
}

%



\newcommand{\tyrletMax}
{
  \inferrule{
  \rctx{1} \jtype{k_1}{t_1}{e_1}{\grt_1} \\
  \Delta; \Phi_a; x: \tchs{\grt_1}, \Gamma \jtypediff{t_2}{e_2}{e}{\tau_2}
}
{ \ctx \jtypediff{t_1+t_2+\klet}{ \elet x = e_1 \ein e_2}{ e}{\tau_2} }~\textbf{r-let-e}
}

\newcommand{\tyrletcsym}
{
  \inferrule{
  \rctx{2} \jtype{k_1}{t_1}{e_1}{\grt_1} \\
  \Delta; \Phi_a; x: \tchs{\grt_1}, \Gamma \jtypediff{t_2}{e}{e_2}{\tau_2}
}
{ \ctx \jtypediff{t_2-k_1-\klet}{ e }{\elet x = e_1 \ein e_2}{\tau_2} }~\textbf{r-e-let}
}


\newcommand{\tyappfun}
{
  \inferrule{
    \rctx{1} \jtype{k_1}{t_1}{e_1}{\grt_1 \uarr{k}{t} \grt_2}
  \\ \ctx \jtypediff{t_2}{e_2}{e_2'}{\tch{\grt_1}{\grt_2'}}
}
{\ctx \jtypediff{t_1+t_2+t+\kapp}{e_1 \eapp e_2}{e_2'}{\tch{\grt_2}{\grt_2'}}}~\textbf{r-app-e}}


\newcommand{\tyefix}
{
 \inferrule{
   \Delta; \Phi_a; x: \tch{\grt_1'}{\grt_1'}, % f : \tchs{(\grt_1 \uarr{k'}{t'} \grt_2')},
   \Gamma \jtypediff{t}{e}{e'}{\tch{\grt_1}{\grt_2'}} \\
    \Delta; \Phi_a; x:\grt_1', % f : \grt_1 \uarr{k'}{t'} \grt_2', 
    \trm{\Gamma}{2} \jtype{k'}{t'}{e'}{\grt_2'}
}
{\ctx \jtypediff{t+t'}{e}{% \efix f(x)
  \elam x  . e'}{\tch{\grt_1}{\grt_1 \uarr{k'}{t'} \grt_2'}}}~\textbf{r-e-lam}
}






\newcommand{\tyappfunsym}
{
  \inferrule{
    \rctx{2} \jtype{k_1}{t_1}{e_1'}{\grt_1' \uarr{k}{t} \grt_2'}
  \\ \ctx \jtypediff{t_2}{e_2}{e_2'}{\tch{\grt_2}{\grt_1'}}
}
{\ctx \jtypediff{t_2-k_1-k-\kapp}{ e_2 }{e_1' \eapp  e_2'}{
  \tch{\grt_2}{\grt_2'}}}~\textbf{r-e-app}}


\newcommand{\tyecase}
{  \inferrule{
    \rctx{2} \jtype{k'}{\_}{e'}{\grt_1 + \grt_2} \\
    \Delta; \Phi_a; x: \tchs{\grt_1}, \Gamma \jtypediff{t}{e}{e_1'}{\tau}\\
    \Delta; \Phi_a; y: \tchs{\grt_2}, \Gamma \jtypediff{t}{e}{e_2'}{\tau}
}{\ctx \jtypediff{t-k'-\kcase}{
   e  }{\ecase(e', x.e_1', y.e_2')}{\tau}}~\textbf{r-e-case}}
%

\newcommand{\tycasee}
{  \inferrule{
    \rctx{1} \jtype{\_}{t}{e}{\grt_1 + \grt_2} \\
    \Delta; \Phi_a; x: \tchs{\grt_1}, \Gamma \jtypediff{t'}{e_1}{e'}{\tau}\\
    \Delta; \Phi_a; y: \tchs{\grt_2}, \Gamma \jtypediff{t'}{e_2}{e'}{\tau}
}{\ctx \jtypediff{t'+t+\kcase}{\ecase(e, x.e_1, y.e_2)}{e'}{\tau}}~\textbf{r-case-e}}
%


% \newcommand{\tyepair}
% {
%   \inferrule
%   {
%     \rctx{1} \jtype{k}{t}{e_2}{\grt_2} \\
%     \ctx \jtypediff{e_1}{e}{}
   
%   }
% }




\newcommand{\tysplit}
{
  \inferrule
  {
    \Delta; \Phi_a \wedge C; \Gamma \jtype{k}{t}{e}{\grt} \\
    \Delta; \Phi_a \wedge \neg C; \Gamma \jtype{k}{t}{e}{\grt} \\
    \Delta \wfcs{C}
  }
  {
    \ctx \jtype{k}{t}{e}{\grt}
  } ~\textbf{split}
}


\newcommand{\tyrsplit}
{
  \inferrule
  {
    \Delta; \Phi_a \wedge C; \Gamma \jtypediff{t}{e_1}{e_2}{\tau}\\
    \Delta; \Phi_a \wedge \neg C; \Gamma \jtypediff{t}{e_1}{e_2}{\tau}\\
    \Delta \wfcs{C}
  }
  {
    \ctx \jtypediff{t}{e_1}{e_2}{\tau} } ~\textbf{r-split}
}


\newcommand{\tycontra}
{\inferrule
{
\Delta; \Phi_a \sat \bot \\
  \Delta; \Phi_a \wfty{\Omega}
}
{
  \ctx \jtype{k}{t}{e}{\grt}
} ~\textbf{contra}
}

\newcommand{\tyrcontra}
{\inferrule
{
\Delta; \Phi_a \sat \bot \\
  \Delta; \Phi_a \wfty{\Gamma}
}
{
  \ctx \jtypediff{t}{e_1}{e_2}{\tau}
} ~\textbf{r-contra}
}

%%% Local Variables:
%%% mode: latex
%%% TeX-master: "main"
%%% End:
