# Supplementary material for: Bidirectional Type Checking for Relational Properties
Source: arXiv:1812.05067 source file (2018-12-12)
Supplement: Supplementary file 37 [file typing-rules-min-defs.tex]

\newcommandx{\mtyswitch}[2][1=,2=]
{
    \inferrule{
    \Delta; \Phi_a; \trm{\Gamma}{1} \jtypeM{k_1}{t_1}{e_1}{\grt_1}~~#1\\
    \Delta; \Phi_a; \trm{\Gamma}{2} \jtypeM{k_2}{t_2}{e_2}{\grt_2}~~#2
    } {\ctx \jtypediffM{t_1-k_2}{\eswitch e_1}{\eswitch e_2}{\tch{\grt_1}{\grt_2}}}~\textbf{c-switch}
}
 

\newcommand{\mtyder}
{
  \inferrule
{
\Delta; \Phi_a; \Gamma  \jtypediffM{t}{e_1}{e_2}{\tbox{\tau}}
}
{
\Delta; \Phi_a; \Gamma  \jtypediffM{t}{\eder e_1}{\eder e_2}{\tau}
} ~\textbf{c-der}
}



\newcommand{\mtynochange}
{
  \inferrule
{
\Delta; \Phi_a; \tbox{\Gamma} \jtypediffM{t}{e}{e}{\tau}
}
{
\Delta; \Phi_a; \tbox{\Gamma}, \Gamma' \jtypediffM{0}{\enoch e}{\enoch e}{\tbox{\tau}}
} ~\textbf{c-nochange}
}



\newcommand{\mtyconst}
{
  \inferrule
  {
  }
  {
    \octx \jtypeM{0}{0}{\econst}{\tint}
  }~\textbf{c-const}
}

\newcommand{\mtyrconst}
{
  \inferrule
  {
  }
  {
    \ctx \jtypediffM{0}{\econst}{\econst}{\trint}
  }~\textbf{c-r-const}
}


\newcommand{\mtyunit}
{
  \inferrule
  {
  }
  {
    \octx \jtypeM{0}{0}{{\eunit}}{\tunit}
  }~\textbf{c-unit}
}

\newcommand{\mtyrunit}
{
  \inferrule
  {
  }
  {
    \ctx \jtypediffM{0}{\eunit}{\eunit}{\trunit}
  }~\textbf{c-r-unit}
}



\newcommand{\mtyelimU}
{\inferrule{
  \octx \jtypeM{k_1}{t_1}{e_1}{\grt_1}\\
  \Delta; \Phi_a;  x: \grt_1 , \Omega \jtypeM{k_2}{t_2}{e_2}{\grt_2}
}
{ \octx \jtypeM{k_1+k_2}{t_1+t_2}{\eelimU x = e_1 \ein e_2}{
  \grt_2} }~\textbf{c-elimU}
}


\newcommand{\mtyrelimU}
{\inferrule{
  \ctx \jtypediffM{t_1}{e_1}{e_1'}{\tch{\grt_1}{\grt_1'}}\\
  \Delta; \Phi_a; \Gamma;  x: \grt_1, \Omega \jtypediffM{t_2}{e_2}{e_2'}{\tau_2}
}
{  \ctx \jtypediffM{t_1+t_2}{\eelimU x = e_1 \ein e_2}{ \eelimU x = e_1' \ein e_2'}{
  \tau_2} }~\textbf{c-r-elimU}
}



\newcommand{\mtyvar}
{  \inferrule{\Omega(x) = \grt }{\octx \jtypeM{0}{0}{x}{\grt}}~\textbf{c-var}
}


\newcommand{\mtyrvar}{
  \inferrule{\Gamma(x) = \tau}{\ctx \jtypediffM{0}{x}{x}{\tau}}~\textbf{c-r-var}
}


\newcommand{\mtyinl}
{
  \inferrule
  {
    \octx  \jtypeM{k}{t}{e}{\grt_1}\\
    {\ifextra
    \Delta; \Phi_a \awfty{\grt_2}
    \fi}
  }
  { \octx  \jtypeM{k}{t}{\einl e}{\grt_1+ \grt_2}
  }~\textbf{c-inl}
}

\newcommand{\mtyrinl}
{  \inferrule
  {
    \ctx  \jtypediffM{t}{e}{e'}{\tau_1}\\
    {
     \ifextra
     \Delta; \Phi_a \wfty{\tau_2}
     \fi
   }
  }
  { \ctx  \jtypediffM{t}{\einl e}{\einl e'}{\tau_1 + \tau_2}
  }~\textbf{c-r-inl}
}


\newcommand{\mtyinr}
{
  \inferrule
  {
    \octx  \jtypeM{k}{t}{e}{\grt_2}\\
    \Delta; \Phi_a \awfty{\grt_1}
  }
  { \octx  \jtypeM{k}{t}{\einr e}{\grt_1 + \grt_2}
  }~\textbf{c-inr}
}
\newcommand{\mtyrinr}
{  \inferrule
  {
    \ctx  \jtypediffM{t}{e}{e'}{\tau_2}\\
    \Delta; \Phi_a \wfty{\tau_1}
  }
  { \ctx  \jtypediffM{t}{\einr e}{\einr e'}{\tau_1 + \tau_2}
  }~\textbf{c-r-inr}
}

\newcommand{\mtycase}
{  \inferrule{\octx \jtypeM{k}{t}{e}{\grt_1 + \grt_2} \\
    \Delta; \Phi_a;  x: \grt_1, \Omega \jtypeM{k'}{t'}{e_1}{\grt} \\
    \Delta; \Phi_a;  y: \grt_2, \Omega \jtypeM{k'}{t'}{e_2}{\grt}}
  {\octx \jtypeM{k+k'+\kcase}{t+t'+\kcase}{\ecase(e, x.e_1, y.e_2)}{\grt}}~\textbf{c-case}
}
%
\newcommand{\mtyrcase}
{  \inferrule{
    \ctx \jtypediffM{t}{e}{e'}{\tau_1 + \tau_2}\\
    \Delta; \Phi_a; x: \tau_1, \Gamma \jtypediffM{t'}{e_1}{e_1'}{\tau}\\
    \Delta; \Phi_a; y: \tau_2, \Gamma  \jtypediffM{t'}{e_2}{e_2'}{\tau}
}{\ctx \jtypediffM{t+t'}{
    \ecase(e, x.e_1, y.e_2)}{\ecase(e', x.e_1', y.e_2')}{\tau}}~\textbf{c-r-case}}
%



\newcommand{\mtyfix}
{  \inferrule{
    {\ifextra
    \Delta; \Phi_a \awfty{\grt_1 \uarr{k}{t} \grt_2} 
    \fi} \\
    \Delta; \Phi_a;  x: \grt_1, f : \grt_1 \uarr{k}{t}
    \grt_2, \Omega  \jtypeM{k}{t}{e}{\grt_2}}
  {
    \octx
    \jtypeM{0}{0}{ \efix f(x).e}{\grt_1 \uarr{k}{t}
    \grt_2}
}~\textbf{c-fix}
}




%
\newcommand{\mtyrfix}
{  \inferrule{
       {\ifextra
       \Delta; \Phi_a \wfty{\tau_1 \tarrd{t} \tau_2}  
       \fi} \\
       \Delta; \Phi_a;  x: \tau_1, f : \tau_1 \tarrd{t} \tau_2, \Gamma  \jtypediffM{t}{e_1}{e_2}{\tau_2}}
            {\ctx \jtypediffM{0}{ \efix f(x).e_1}{\efix f(x).e_2}{
              \tau_1 \tarrd{t} \tau_2}}~\textbf{c-r-fix}}
%

\newcommand{\mtyrfixNC}
{  \inferrule
  {
    {\ifextra \Delta; \Phi_a \wfty{\tau_1 \tarrd{t} \tau_2}
      \fi} \\
    \Delta; \Phi_a;  x: \tau_1, f : \tbox{(\tau_1 \tarrd{t} \tau_2)}, \tbox{\Gamma} \jtypediffM{t}{e}{e}{\tau_2}
  }
  {\nctx \jtypediffM{0}{\efixNC f(x).e}{\efixNC f(x).e}{
              \tbox{(\tau_1 \tarrd{t} \tau_2)}}}~\textbf{c-r-fixNC}
} 



\newcommand{\mtyrfixE}
{  \inferrule{
    \Delta; \Phi_a; \Gamma;  x: \tau_1, f : \tau_1 \uarr{k}{t} \tau_2, \Omega  \jtypeM{k_1}{t_1}{e_1}{\tau_2} \\
    \Delta; \Phi_a; \Gamma;  x: \tau_1, f : \tau_1 \uarr{k}{t} \tau_2,\Omega  \jtypeM{k_2}{t_2}{e_2}{\tau_2}
}
{\ctx \jtypediffM{0}{ \efix f(x).e_1}{\efix f(x).e_2}{
              \tau_1 \uarr{k}{t} \tau_2}}~\textbf{c-r-fix$\wexec$}}
%


\newcommand{\mtyapp}
{\inferrule{
  \octx \jtypeM{k_1}{t_1}{e_1}{\grt_1\uarr{k}{t} \grt_2} \\
  \octx \jtypeM{k_2}{t_2}{e_2}{\grt_1}}
{
  \octx \jtypeM{k_1+k_2+k+\kapp}{t_1+t_2+t+\kapp}{ e_1 \eapp e_2}{
  \grt_2}}~\textbf{c-app}}
%
% \inferrule{\ctx \jtypemin{k_1} e_1: (\tau_1\uarr{\wmin}{k} \tau_2)^\mu
%   \\ \ctx \jtypemin{k_2} e_2: \tau_1\\ (\mu = \achange) \Rightarrow
%   (\lbound \tau_2)}{\ctx \jtypemin{k_1 + k_2 + k + 1} e_1 \eapp e_2: \tau_2} \and
% %
 


\newcommand{\mtyrappD}
{\inferrule{\ctx \jtypediffM{t_1}{e_1}{e_1'}{\tau_1}
  \tarrd{t} \tau_2 \\\\
  \ctx \jtypediffM{t_2}{ e_2}{e_2'}{\tau_1}
}
{\ctx \jtypediffM{{t_1+t_2+t}}{e_1 \eapp e_2}{e_1' \eapp e_2'}{\tau_2}}~\textbf{c-r-app}}



\newcommand{\mtyiLam}
{  \inferrule{
    i::S, \octx \jtypeM{k}{t}{e}{\grt}\\
    i \not \in \fiv{\Phi_a; \Omega}
  }
  { \octx \jtypeM{0}{0}{\eLam i. e}{\tforall{i}{k}{t} \grt}}~\textbf{c-iLam }}
%
\newcommand{\mtyriLam}
{ \inferrule{
    i::S, \ctx \jtypediffM{t}{e}{e'}{\tau} \\
    i \not \in \fiv{\Phi_a; \Gamma} 
  }
  { \ctx \jtypediffM{0}{\eLam i. e}{\eLam i. e'}{\tforalld{i}{t} \tau}}~\textbf{c-r-iLam}}
%
\newcommand{\mtyriLamc}
{  \inferrule{
    i::S, \ctx \jtypeM{k}{t}{e}{\tau} \\
    i::S, \ctx \jtypeM{k}{t}{e'}{\tau} \\
  }
  { \ctx \jtypediffM{0}{\eLam i. e}{\eLam i. e'}{\tforall{i}{k}{t} \tau}}~\textbf{c-r-iLam2}
}

\newcommand{\mtyiApp}
{  \inferrule{
    \octx \jtypeM{k}{t}{e}{\tforall{i}{k'}{t'} \grt} \\
    \Delta \vdash I : S
  }
  {\octx \jtypeM{k+k'[I/i]}{t+t'[I/i]}{e [I]}{\grt\{ I/ i\}}}~\textbf{c-iApp}}
%
\newcommand{\mtyriApp}
{  \inferrule{
    \ctx \jtypediffM{t}{e}{e'}{\tforalld{i}{t'} \tau}\\
    \Delta \vdash I : S
  }
  {\ctx \jtypediffM{t+t'[I/i]}{e [I]}{e' [I]}{\tau\{ I/ i\}}}~\textbf{c-r-iApp}}
%

\newcommand{\mtypack}
{
\inferrule
{
  \octx  \jtypeM{k}{t}{e}{\grt\{I/i\}} \\
  \Delta \sty{I}{\sort}
}
{
  \octx  \jtypeM{k}{t}{\epack e \ewith I}{\texists{i} \grt}
} ~\textbf{c-pack}
}

\newcommand{\mtyrpack}{
\inferrule
{
  \ctx  \jtypediffM{t}{e}{e'}{\tau\{I/i\}}\\
  \Delta \sty{I}{\sort}
}
{
  \ctx  \jtypediffM{t}{\epack e \ewith I}{\epack e' \ewith I}{\texists{i} \tau}
} ~\textbf{c-r-pack}
}

\newcommand{\mtyunpack}{
\inferrule
{
  \octx \jtypeM{k_1}{t_1}{e_1}{\texists{i} \grt_1} \\
  \sorted{i}, \Delta; \Phi_a;  x: \grt_1, \Omega \jtypeM{k_2}{t_2}{e_2}{\grt_2} \\
  i \not\in FV(\Phi_a;\Gamma, \grt_2, k_2, t_2) \\
}
{
  \octx  \jtypeM{k_1+k_2}{t_1+t_2}{\eunpack e_1 \eas (x, i) \ein  e_2}{\grt_2}
}~\textbf{c-unpack}
}


\newcommand{\mtyrunpackD}{
\inferrule
{
  \ctx \jtypediffM{t_1}{e_1}{e_1'}{\texists{i} \tau_1}\\
  \sorted{i}, \Delta; \Phi_a; x: \tau_1, \Gamma \jtypediffM{t_2}{e_2}{e_2'}{\tau_2}\\
  i \not\in FV(\Phi_a;\Gamma, \tau_2, t_2) \\
}
{
  \ctx  \jtypediffM{t_1+t_2}{\eunpack e_1 \eas (x, i) \ein  e_2}{\eunpack e_1' \eas (x, i) \ein  e_2'}{\tau_2}
}~\textbf{c-r-unpack1}}


\newcommand{\mtynil}
{ \inferrule
  {
    {\ifextra
      \Delta; \Phi_a \awfty{\grt}
    \fi}
  }
  { \octx \jtypeM{0}{0}{\enil}{\ulist{0}{\grt}}
}~\textbf{c-nil}}
%
\newcommand{\mtyrnil}
{  \inferrule
  {
    \Delta; \Phi_a \wfty{\tau}
  }
  { \ctx \jtypediffM{0}{\enil}{\enil}{\tlist{0}{\alpha}{\tau}}}~\textbf{c-r-nil}
}

\newcommand{\mtycons}
{  \inferrule
  { \octx \jtypeM{k_1}{t_1}{e_1}{\grt} \\
    \octx \jtypeM{k_2}{t_2}{e_2}{\ulist{n}{\grt}}
  }
  { \octx \jtypeM{k_1+k_2}{t_1+t_2}{\econsC(e_1,e_2)}{\ulist{n+1}{\grt}}}~\textbf{c-cons}}
%
\newcommand{\mtyrcons} 
{   \inferrule
  { \ctx \jtypediffM{t_1}{e_1}{e_1'}{\tau} \\
    \ctx \jtypediffM{t_2}{e_2}{e_2'}{\tlist{n}{\alpha}{\tau}}
  }
  { \ctx \jtypediffM{t_1+t_2}{ \econsC(e_1,e_2) }{ \econsC(e_1',e_2')}{\tlist{n+1}{\alpha+1}{\tau}}}~\textbf{c-r-cons1}}
%
\newcommand{\mtyrconsbox}
{   \inferrule
  { \ctx \jtypediffM{t_1}{e_1}{e_1'}{\tbox{\tau}} \\
    \ctx \jtypediffM{t_2}{e_2}{e_2'}{\tlist{n}{\alpha}{\tau}}}
  { \ctx \jtypediffM{t_1+t_2}{ \econsNC(e_1,e_2) }{ \econsNC(e_1',e_2')}{\tlist{n+1}{\alpha}{\tau}}}~\textbf{c-r-cons2}}
%

\newcommand{\mtycaseL}
 { \inferrule
  {\octx \jtypeM{k}{t}{e}{\ulist{n}{\grt}} \\
   \Delta; \Phi_a \wedge n = 0 ;  \Omega \jtypeM{k'}{t'}{e_1}{\grt'} \\
   i, \Delta; \Phi_a \wedge n = i+1 ;  h: \grt, tl : \ulist{i}{\grt}, \Omega
   \jtypeM{k'}{t'}{e_2}{\grt'}
  } 
  {\octx \jtypeM{k+k'+\kcaseL}{t+t'+\kcaseL}{ \ecase e \eof \enil \rightarrow e_1 ~|~ h::_{NC}tl \rightarrow
    e_2 ~|~ h::_{C}tl \rightarrow
    e_3}{\grt'}}~\textbf{c-caseL}
 }

\newcommand{\mtyrcaseL}
{ \inferrule
  {\ctx \jtypediffM{t}{e}{e'}{\tlist{n}{\alpha}{\tau}}\\
   \Delta; \Phi_a \wedge n = 0  ;\Gamma \jtypediffM{t'}{e_1}{e_1'}{\tau'}\\
   i, \Delta; \Phi_a \wedge n = i+1;  h: \tbox{\tau},
   tl : \tlist{i}{\alpha}{\tau}, \Gamma \jtypediffM{t'}{e_2}{e_2'}{\tau'}
\\
   i, \beta, \Delta; \Phi_a \wedge n = i+1 \wedge \alpha = \beta +1 ;
   h': \tau, tl : \tlist{i}{\beta}{\tau}, \Gamma \jtypediffM{t'}{e_3}{e_3'}{\tau'}
   }
  {\ctx \jtypediffM{t+t'}{
      \begin{minipage}[c]{10em}
        ~ $\ecase e \eof \enil \, \rightarrow e_1$ \\
         $~~~~~~~~|~h\,::_{N} tl\, \rightarrow e_2$ \\
         $~~~~~~~~|~h'::_{C} tl' \rightarrow e_3$
      \end{minipage}
}{
      \begin{minipage}[c]{10em}
         ~ $\ecase e \eof \enil \, \rightarrow e_1'$ \\
         $~~~~~~~~|~h\,::_{N} tl\, \rightarrow e_2'$ \\
         $~~~~~~~~|~h'::_{C} tl' \rightarrow e_3'$
      \end{minipage}
}{\tau'}}~\textbf{c-r-caseL}
}


\newcommand{\mtyleaf}
 { \inferrule
  {
    \Delta; \Phi_a \awfty{\grt}
  }
  { \octx \jtypeM{0}{0}{\eleaf}{\utree{0}{\grt}}}~\textbf{c-leaf}}
%
\newcommand{\mtyrleaf}
{  \inferrule
  {
    \Delta; \Phi_a \wfty{\tau}
  }
  { \ctx \jtypediffM{0}{\eleaf}{\eleaf}{\ttree{0}{\alpha}{\tau}}}~\textbf{c-r-leaf}
}

\newcommand{\mtynode}
{ \inferrule
  { \\
    \octx \jtypeM{k}{t}{e}{\grt} \\
    \octx \jtypeM{k_1}{t_1}{e_l}{\utree{i}{\grt}} \\
    \octx \jtypeM{k_2}{t_2}{e_r}{\utree{j}{\grt}} 
  }
  { \octx \jtypeM{k+k_1+k_2}{t+t_1+t_2}{\enode(e_l,e,e_r)}{\utree{i+j+1}{\grt}}}~\textbf{c-node}
}
%

\newcommand{\mtyrnode}
{   \inferrule
  { \\
    \ctx \jtypediffM{t}{e}{e'}{\tau}\\
    \ctx \jtypediffM{t_1}{e_l}{e_l'}{\ttree{i}{\alpha}{\tau}}\\
    \ctx \jtypediffM{t_2}{e_r}{e_r'}{\ttree{j}{\beta}{\tau} }}
  { \ctx \jtypediffM{t+t_1+t_2}{\enode(e_l,e,e_r)}{\enode(e_l',e',e_r')}{\ttree{i+j+1}{\alpha+\beta+1}{\tau}}}~\textbf{c-r-node1}
}

\newcommand{\mtyrnodeb}
{   \inferrule
  { \\
    \ctx \jtypediffM{t}{e}{e'}{\tbox{\tau}}\\
    \ctx \jtypediffM{t_1}{e_l}{e_l'}{\ttree{i}{\alpha}{\tau}}\\
    \ctx \jtypediffM{t_2}{e_r}{e_r'}{\ttree{j}{\beta}{\tau} }}
  { \ctx \jtypediffM{t+t_1+t_2}{\enode(e_l,e,e_r)}{\enode(e_l',e',e_r')}{\ttree{i+j+1}{\alpha+\beta}{\tau}}}~\textbf{c-r-node2}
}



\newcommand{\mtycaseT}
{  \inferrule
  {\octx \jtypeM{k}{t}{e}{\utree{n}{\grt}} \\
   \Delta; \Phi_a \wedge n = 0 ; \Omega \jtypeM{k'}{t'}{e_1}{\grt'} \\
   i, j, \Delta; \Phi_a \wedge n = i+j+1;  x: \grt, l : \utree{i}{\grt}, r : \utree{j}{\grt}, \Omega \jtypeM{k'}{t'}{e_2}{\grt'}
   }
  {\octx \jtypeM{k+k'+\kcaseT}{t+t'+\kcaseT}{\ecase e \eof \eleaf \rightarrow e_1 ~|~ \enode(l,x,r) \rightarrow
    e_2}{\grt'}}~\textbf{c-caseT}
}
 %
\newcommand{\mtyrcaseT}
{ \inferrule
  {\ctx \jtypediffM{t}{e}{e'}{\ttree{n}{\alpha}{\tau}}\\
   \Delta; \Phi_a \wedge n = 0  \wedge  ; \Gamma \jtypediffM{t'}{e_1}{e_1'}{\tau'}\\
   i,j, \beta, \theta, \Delta; \Phi_a \wedge n = i+j+1 \wedge \alpha = \beta + \theta ;  x: \tbox{\tau}, l : \ttree{i}{\beta}{\tau}, r : \ttree{j}{\theta}{\tau}, \Gamma \jtypediffM{t'}{ e_2}{e_2'}{\tau'} \\
     i,j, \beta, \theta, \Delta; \Phi_a \wedge n = i+j+1 \wedge \alpha = \beta + \theta +1;  x: \tau, l : \ttree{i}{\beta}{\tau}, r : \ttree{j}{\theta}{\tau}, \Gamma  \jtypediffM{t'}{e_2}{e_2'}{\tau'}
   }
  {\ctx \jtypediffM{t+t'}{\ecase e \eof \eleaf \rightarrow e_1 ~|~ \enode(l,x,r) \rightarrow
    e_2}{\ecase e' \eof \eleaf \rightarrow e_1' ~|~ \enode(l,x,r) \rightarrow}{e_2'}{\tau'}}~\textbf{c-r-caseT}
}

\newcommand{\mtyprod}
{\inferrule{
    \octx \jtypeM{k_1}{t_1}{e_1}{\grt_1} \\
    \octx \jtypeM{k_2}{t_2}{e_2}{\grt_2}}
  {
    \octx \jtypeM{k_1+k_2}{t_1+t_2}{\la e_1, e_2 \ra}{\grt_1
  \ttimes \grt_2}}~\textbf{c-prod}
}


\newcommand{\mtyrprod}
{\inferrule{\ctx \jtypediffM{t_1}{e_1}{e_1'}{\tau_1}\\ \ctx
  \jtypediffM{t_2}{ e_2}{e_2'}{\tau_2}
}
{
  \ctx 
  \jtypediffM{t_1+t_2}{\la e_1, e_2 \ra}{\la e_1' , e_2' \ra}{\tau_1 \ttimes \tau_2}
}~\textbf{c-r-prod}
}

\newcommand{\mtyproj}
{\inferrule{\octx \jtypeM{k}{t}{e}{\grt_1 \ttimes \grt_2}}
  {\octx
  \jtypeM{k+\kproj}{t+\kproj}{\eleft(e)}{\grt_1}}~\textbf{c-proj1}}

\newcommand{\mtyrproj}
{\inferrule{
    \ctx \jtypediffM{t}{e}{e'}{\tau_1 \ttimes\tau_2}
}
{\ctx \jtypediffM{t}{ \eleft(e)}{\eleft(e')}{\tau_1}}~\textbf{c-r-proj1}
}



\newcommand{\mtylet}
{\inferrule{
  \octx \jtypeM{k_1}{t_1}{e_1}{\grt_1} \\
  \Delta;\Phi_a;  x: \grt_1 , \Omega \jtypeM{k_2}{t_2}{e_2}{\grt_2}
}
{ \octx \jtypeM{k_1+k_2+\klet}{t_1+t_2+\klet}{\elet x = e_1 \ein e_2}{
  \grt_2}
}~\textbf{c-let}}
%
\newcommand{\mtyrlet}
{\inferrule{
  \ctx \jtypediffM{t_1}{e_1}{e_1'}{\tau_1}\\
  \Delta; \Phi_a; x: \tau_1, \Gamma  \jtypediffM{t_2}{e_2}{e_2'}{\tau_2}
}
{ \ctx \jtypediffM{t_1+t_2}{ \elet x = e_1 \ein e_2 }{\elet x = e_1' \ein e_2'}{
  \tau_2} }~\textbf{c-r-let1}
}


\newcommand{\mtycandIntro}
{\inferrule
{
\Delta; \Phi_a \sat C \\
  \Delta; \Phi_a \wedge C;  \Omega \jtypeM{k}{t}{e}{\grt}
}
{
  \octx \jtypeM{k}{t}{e}{\tcprod{C}{\grt}}
} ~\textbf{c-candI}
}

\newcommand{\mtyrcandIntro}
{\inferrule
{
\Delta; \Phi_a \sat C \\
  \Delta; \Phi_a \wedge C; \Gamma  \jtypediffM{t}{e}{e'}{\tau}
}
{
  \ctx  \jtypediffM{t}{e}{e'}{\tcprod{C}{\tau}}
} ~\textbf{c-r-candI}
}

\newcommand{\mtycandElim}
{
\inferrule
{
  \octx \jtypeM{k_1}{t_1}{e_1}{\tcprod{C}{\grt_1}} \\
  \Delta; \Phi_a \wedge C;   x :\grt_1,  \Omega  \jtypeM{k_2}{t_2}{ e_2}{\grt_2} \\
}
{
  \octx  \jtypeM{k_1+k_2}{t_1+t_2}{\clet e_1 \eas x \ein e_2}{\grt_2}
} ~\textbf{c-candE}
}

\newcommand{\mtyrcandElimD}
{
\inferrule
{
  \ctx \jtypediffM{t_1}{e_1}{e_1 '}{\tcprod{C}{\tau_1}}\\
  \Delta; \Phi_a \wedge C; x :\tau_1, \Gamma  \jtypediffM{t_2}{ e_2}{e_2'}{\tau_2}
}
{
  \ctx  \jtypediffM{t_1+t_2}{\clet e_1 \eas x \ein e_2}{\clet e_1' \eas x \ein e_2'}{\tau_2}
} ~\textbf{c-r-candE}
}

\newcommand{\mtycimplIntro}
{
\inferrule
{
\Delta; \Phi_a \wedge C;  \Omega  \jtypeM{k}{t}{e}{{\grt}}
}
{
  \octx  \jtypeM{k}{t}{e}{\tcimpl{C}{\grt}}
} ~\textbf{c-cimpI}

}

\newcommand{\mtyrcimplIntro}
{
\inferrule
{
\Delta; \Phi_a \wedge C; \Gamma  \jtypediffM{t}{e}{e'}{\tau}
}
{
  \ctx  \jtypediffM{t}{e}{e'}{\tcimpl{C}{\tau}}
} ~\textbf{c-r-cimpI}
}


\newcommand{\mtycimplElim}
{
\inferrule
{
  \octx  \jtypeM{k}{t}{e}{\tcimpl{C}{\grt}} \\
\Delta; \Phi_a \sat C
}
{
  \octx  \jtypeM{k}{t}{\ecelim e}{\grt}
} ~\textbf{c-cimplE}
}

\newcommand{\mtyrcimplElimD}
{
\inferrule
{
  \ctx  \jtypediffM{t}{e}{e'}{\tcimpl{C}{\tau}}\\
\Delta; \Phi_a \sat C
}
{
  \ctx  \jtypediffM{t}{\ecelim e}{\ecelim  e'}{\tau}
} ~\textbf{c-r-cimplE}
}



\newcommand{\mtyprimapp}
{\inferrule{
    \primctx(\zeta) =  \grt_1 \uarr{k}{t} \grt_2  \\
  \octx \jtypeM{k'}{t'}{e}{\grt_1}}
{
   \octx \jtypeM{k+k'+\kapp}{t+t'+\kapp}{\zeta \eapp e}{\grt_2}}~\textbf{c-primapp}}


\newcommand{\mtyrprimapp}
{\inferrule{
    \primctx(\zeta) = \tau_1 \tarrd{t} \tau_2 \\
    \ctx \jtypediffM{t'}{e}{e'}{\tau_1}
}
{
 \ctx \jtypediffM{t+t'}{\zeta \eapp e}{\zeta \eapp e'}{
  \tau_2}}~\textbf{c-r-primapp}}


\newcommand{\mtyinterI}
{
   \inferrule{
    \octx \jtypeM{k}{t}{e}{\grt_1} \\
    \octx \jtypeM{k}{t}{e}{\grt_2} \\
}{
  \octx \jtypeM{k}{t}{e}{\grt_1 \tinter \grt_2}}~\textbf{c-interI}
}

\newcommand{\mtyrinterI}
{
   \inferrule{
    \ctx \jtypediffM{t}{e}{e'}{\tau_1}\\
    \ctx \jtypediffM{t}{e}{e'}{\tau_2}\\
}{
  \ctx \jtypediffM{t}{ e }{ e'}{\tau_1 \tinter \tau_2}}~\textbf{c-r-interI}
}


\newcommandx{\mtyinterE}[1][1=i]
{
   \inferrule{
     \octx \jtypeM{k}{t}{e}{\grt_1 \tinter \grt_2} \\
}{
  \octx \jtypeM{k}{t}{e}{\grt_{#1}} }~\textbf{c-interE$_{#1}$}
}

\newcommandx{\mtyrinterE}[1][1=i]
{
   \inferrule{
    \ctx \jtypediffM{t}{e}{e'}{\tau_1 \tinter \tau_2}\\
}{
  \ctx \jtypediffM{t}{ e}{e'}{\tau_{#1}} }~\textbf{c-r-interE$_{#1}$}
}



\newcommand{\mtysubsum}
{
   \inferrule{
    \octx \jtypeM{k}{t}{e}{\grt} \\
    \Delta; \Phi_a \jsubtype{\grt}{\grt'} \\
    \Delta; \Phi_a \sat \cleq{k'}{k} \\
    \Delta; \Phi_a \sat \cleq{t}{t'}
}{
  \octx \jtypeM{k'}{t'}{e}{\grt'}
}~{\textbf{c-r}\pmb{\sqsubseteq}\wexec}
}

\newcommand{\mtyrsubsum}
{
   \inferrule{
     \ctx \jtypediffM{t}{e}{e'}{\tau}\\
     \Delta; \Phi_a \jeqtype{\tau}{\tau'} \\\\
    \Delta; \Phi_a \sat \cleq{t}{t'}
  }
  {\ctx \jtypediffM{t'}{e}{e'}{\tau'} }
  ~{\textbf{c-r}-\pmb{\sqsubseteq}}
}

%



\newcommand{\mtyrletMax}
{
  \inferrule{
  \rctx{1} \jtypeM{k_1}{t_1}{e_1}{\grt_1} \\
  \Delta; \Phi_a; x: \tchs{\grt_1}, \Gamma \jtypediffM{t_2}{e_2}{e}{\tau_2}
}
{ \ctx \jtypediffM{t_1+t_2+\klet}{ \elet x = e_1 \ein e_2}{ e}{\tau_2} }~\textbf{c-r-let-e}
}

\newcommand{\mtyrletcsym}
{
  \inferrule{
  \rctx{2} \jtypeM{k_1}{t_1}{e_1}{\grt_1} \\
  \Delta; \Phi_a; x: \tchs{\grt_1}, \Gamma \jtypediffM{t_2}{e}{e_2}{\tau_2}
}
{ \ctx \jtypediffM{t_2-k_1-\klet}{ e }{\elet x = e_1 \ein e_2}{\tau_2} }~\textbf{c-r-e-let}
}


\newcommand{\mtyappfun}
{
  \inferrule{
    \rctx{1} \jtypeM{k_1}{t_1}{e_1}{\grt_1 \uarr{k}{t} \grt_2}
  \\ \ctx \jtypediffM{t_2}{e_2}{e_2'}{\tch{\grt_1}{\grt_2'}}
}
{\ctx \jtypediffM{t_1+t_2+t+\kapp}{e_1 \eapp e_2}{e_2'}{\tch{\grt_2}{\grt_2'}}}~\textbf{c-r-app-e}}


\newcommand{\mtyefix}
{
 \inferrule{
   \Delta; \Phi_a; x: \tch{\grt_1'}{\grt_1'}, % f : \tchs{(\grt_1 \uarr{k'}{t'} \grt_2')},
   \Gamma \jtypediffM{t}{e}{e'}{\tch{\grt_1}{\grt_2'}} \\
    \Delta; \Phi_a; x:\grt_1', % f : \grt_1 \uarr{k'}{t'} \grt_2', 
    \trm{\Gamma}{2} \jtypeM{k'}{t'}{e'}{\grt_2'}
}
{\ctx \jtypediffM{t+t'}{e}{% \efix f(x)
  \elam x  . e'}{\tch{\grt_1}{\grt_1 \uarr{k'}{t'} \grt_2'}}}~\textbf{c-r-e-lam}
}






\newcommand{\mtyappfunsym}
{
  \inferrule{
    \rctx{2} \jtypeM{k_1}{t_1}{e_1'}{\grt_1' \uarr{k}{t} \grt_2'}
  \\ \ctx \jtypediffM{t_2}{e_2}{e_2'}{\tch{\grt_2}{\grt_1'}}
}
{\ctx \jtypediffM{t_2-k_1-k-\kapp}{ e_2 }{e_1' \eapp  e_2'}{
  \tch{\grt_2}{\grt_2'}}}~\textbf{c-r-e-app}}


\newcommand{\mtyecase}
{  \inferrule{
    \rctx{2} \jtypeM{k'}{\_}{e'}{\grt_1 + \grt_2} \\
    \Delta; \Phi_a; x: \tchs{\grt_1}, \Gamma \jtypediffM{t}{e}{e_1'}{\tau}\\
    \Delta; \Phi_a; y: \tchs{\grt_2}, \Gamma \jtypediffM{t}{e}{e_2'}{\tau}
}{\ctx \jtypediffM{t-k'-\kcase}{
   e  }{\ecase(e', x.e_1', y.e_2')}{\tau}}~\textbf{c-r-e-case}}
%

\newcommand{\mtycasee}
{  \inferrule{
    \rctx{1} \jtypeM{\_}{t}{e}{\grt_1 + \grt_2} \\
    \Delta; \Phi_a; x: \tchs{\grt_1}, \Gamma \jtypediffM{t'}{e_1}{e'}{\tau}\\
    \Delta; \Phi_a; y: \tchs{\grt_2}, \Gamma \jtypediffM{t'}{e_2}{e'}{\tau}
}{\ctx \jtypediffM{t'+t+\kcase}{\ecase(e, x.e_1, y.e_2)}{e'}{\tau}}~\textbf{c-r-case-e}}
%


% \newcommand{\mtyepair}
% {
%   \inferrule
%   {
%     \rctx{1} \jtypeM{k}{t}{e_2}{\grt_2} \\
%     \ctx \jtypediffM{e_1}{e}{}
   
%   }
% }




\newcommand{\mtysplit}
{
  \inferrule
  {
    \Delta; \Phi_a \wedge C; \Omega \jtypeM{k}{t}{e_1}{\grt} \\
    \Delta; \Phi_a \wedge \neg C; \Omega \jtypeM{k}{t}{e_2}{\grt} \\
  }
  {
    \octx \jtypeM{k}{t}{\esplit (e_1, e_2) \ewith C}{\grt}
  } ~\textbf{c-split}
}


\newcommand{\mtyrsplit}
{
  \inferrule
  {
    \Delta; \Phi_a \wedge C; \Gamma \jtypediffM{t}{e_1}{e_2}{\tau}\\
    \Delta; \Phi_a \wedge \neg C; \Gamma \jtypediffM{t}{e_1'}{e_2'}{\tau}\\
  }
  {
    \ctx \jtypediffM{t}{\esplit (e_1,e_1') \ewith C}{\esplit (e_2,e_2') \ewith C}{\tau} } ~\textbf{c-r-split}
}


\newcommand{\mtycontra}
{\inferrule
{
\Delta; \Phi_a \sat \bot \\
  \Delta; \Phi_a \wfty{\Omega}
}
{
  \octx \jtypeM{k}{t}{\econtra e}{\grt}
} ~\textbf{c-contra}
}

\newcommand{\mtyrcontra}
{\inferrule
{
\Delta; \Phi_a \sat \bot \\
  \Delta; \Phi_a \wfty{\Gamma}
}
{
  \ctx \jtypediffM{t}{\econtra  e_1}{\econtra  e_2}{\tau}
} ~\textbf{c-r-contra}
}

%%% Local Variables:
%%% mode: latex
%%% TeX-master: "main"
%%% End:
