# Supplementary material for: Bidirectional Type Checking for Relational Properties
Source: arXiv:1812.05067 source file (2018-12-12)
Supplement: Supplementary file 38 [file typing-rules-min.tex]

\begin{figure}

\framebox{General rules}
\begin{mathpar}
  \mtyswitch
  \and
  \mtynochange
  \and
  \mtyder
\end{mathpar}
 

\framebox{Constant integers and unit}
\begin{mathpar}
  \mtyconst
  \and
  \mtyrconst
  \and
  \mtyunit
  \and
  \mtyrunit
\end{mathpar}

\framebox{Variables $x$}
\begin{mathpar}
  \mtyvar
  \and
  \mtyrvar
\end{mathpar}


\framebox{$\einl e $ }
\begin{mathpar}
  \mtyinl
  \and
  \mtyrinl
\end{mathpar}


\framebox{$\einr e $ }
\begin{mathpar}
  \mtyinr
  \and
  \mtyrinr
\end{mathpar}

\framebox{$\ecase(e,x.e_1,y.e_2)$}
\begin{mathpar}
 \mtycase
 \and
 \mtyrcase
\end{mathpar}


\caption{{\tnamemin} typing rules (Part 1)}
\label{fig:relcostcore-typing1}
\end{figure}



\begin{figure}


\framebox{$\efix f(x).e$}
\begin{mathpar}
  \mtyfix
  \and
  \mtyrfix
  \and
  \mtyrfixNC
\end{mathpar}


\framebox{$e_1 \eapp e_2$}
\begin{mathpar}
  \mtyapp
  \and
  \mtyrappD
  % \and
  % \mtyrappE
\end{mathpar}


\framebox{$\la e_1, e_2 \ra$}
\begin{mathpar}
  \mtyprod
  \and
  \mtyrprod
\end{mathpar}

\framebox{$\eleft (e)$}
\begin{mathpar}
  \mtyproj
  \and
  \mtyrproj
\end{mathpar}


\framebox{$\eright (e)$}\\

Symmetric rules. \\



\caption{{\tnamemin} typing rules (Part 2)}
\label{fig:relcostcore-typing2}
\end{figure}


\begin{figure}




\framebox{$\enil$}
\begin{mathpar}
  \mtynil
  \and
  \mtyrnil
\end{mathpar}


\framebox{$\econs(e_1,e_2)$}
\begin{mathpar}
  \mtycons
  \and
  \mtyrcons
  \and
  \mtyrconsbox
\end{mathpar}

\framebox{$\ecase e \eof \enil \rightarrow e_1 ~|~ h::tl \rightarrow e_2$}
\begin{mathpar}
  \mtycaseL
  \and
  \mtyrcaseL
\end{mathpar}

% \framebox{$\eleaf$}
% \begin{mathpar}
%   \mtyleaf
%   \and
%   \mtyrleaf
% \end{mathpar}

% \framebox{$\enode(e_l,e, e_r)$}
% \begin{mathpar}
%   \mtynode
%   \and
%   \mtyrnode
%   \and
%   \mtyrnodeb
%  \end{mathpar}

\caption{{\tnamemin} typing rules (Part 3)}
\label{fig:relcostcore-typing3}
\end{figure}




\begin{figure}
% \framebox{$\ecase e \eof \eleaf \rightarrow e_1 ~|~ \enode(l,x,r) \rightarrow e_2$}
% \begin{mathpar}
%   \mtycaseT
%   \and
%   \mtyrcaseT
% \end{mathpar}


\framebox{$\eLam e$}
\begin{mathpar}
  \mtyiLam
  \and
  \mtyriLam
\end{mathpar}


\framebox{$e \eApp$}
\begin{mathpar}
  \mtyiApp
  \and
  \mtyriApp
\end{mathpar}

\framebox{$\epack e$}
\begin{mathpar}
  \mtypack
  \and
  \mtyrpack
\end{mathpar}


\framebox{$\eunpack e \eas x \ein e'$}
\begin{mathpar}
  \mtyunpack
  \and
  \mtyrunpackD
\end{mathpar}


\caption{{\tnamemin} typing rules (Part 4)}
\label{fig:relcostcore-typing4}

\end{figure}





\begin{figure}

\framebox{Primitive application}
\begin{mathpar}
  \mtyprimapp
  \and
  \mtyrprimapp
\end{mathpar}



\framebox{$\tcprod{C}{\tau}$ intro. rules}
\begin{mathpar}
  \mtycandIntro
  \and
  \mtyrcandIntro
\end{mathpar}

\framebox{$\tcprod{C}{\tau}$ elim. rules}
\begin{mathpar}
  \mtycandElim
  \and
  \mtyrcandElimD
\end{mathpar}

\framebox{$\tcimpl{C}{\tau}$ intro. rules}
\begin{mathpar}
  \mtycimplIntro
  \and
  \mtyrcimplIntro
\end{mathpar}


\framebox{$\tcimpl{C}{\tau}$ elim. rules}
\begin{mathpar}
  \mtycimplElim
  \and
  \mtyrcimplElimD
\end{mathpar}

% \framebox{Intersection intro. rules}
% \begin{mathpar}
%   \mtyinterI
%   \and
%   \mtyrinterI
% \end{mathpar}

% \framebox{Intersection elim. rules}
% \begin{mathpar}
%   \mtyinterE
%   \and
%   \mtyrinterE
% \end{mathpar}


\framebox{$\elet x = e_1 \ein e_2$}
\begin{mathpar}
  \mtylet
  \and
  \mtyrlet
\end{mathpar}

\caption{{\tnamemin} typing rules (Part 5)}
\label{fig:relcostcore-typing5}
\end{figure}


 
\begin{figure}



\framebox{Unary Subtyping}
\begin{mathpar}
  \mtysubsum
\end{mathpar}


\framebox{Binary Subeffecting}
\begin{mathpar}
  \mtyrsubsum
\end{mathpar}



\framebox{Constraint dependent typing}
\begin{mathpar}
  \mtysplit
  \and
  \mtyrsplit
  \and
  \mtycontra
  \and
  \mtyrcontra
\end{mathpar}


\framebox{Heuristic typing}
\begin{mathpar}
  \mtyrletMax
  \and
  \mtyrletcsym
  \and
  \mtyappfun
  \and
  \mtyappfunsym
  \and
  % \mtyefix
  % \and
  \mtycasee
  \and 
  \mtyecase
  % \and
  % \mtyepair
\end{mathpar}

\caption{{\tnamemin} typing rules (Part 6)}
\label{fig:relcostcore-typing6}
\end{figure}



%%% Local Variables:
%%% mode: latex
%%% TeX-master: "main"
%%% End:
