# Supplementary material for: Bidirectional Type Checking for Relational Properties
Source: arXiv:1812.05067 source file (2018-12-12)
Supplement: Supplementary file 39 [file typing-rules.tex]

\begin{figure}

\framebox{General rules}
\begin{mathpar}
  \tyswitch
  \and
  \tynochange
\end{mathpar}


% \framebox{$\eelimU x = e_1 \ein e_2$}
% \begin{mathpar}
%   \tyelimU
%   \and
%   \tyrelimU
% \end{mathpar}

\framebox{Constant integers and unit}
\begin{mathpar}
  \tyconst
  \and
  \tyrconst
  \and
  \tyunit
  \and
  \tyrunit
\end{mathpar}

\framebox{Variables $x$}
\begin{mathpar}
  \tyvar
  \and
  \tyrvar
\end{mathpar}


\framebox{$\einl e $ }
\begin{mathpar}
  \tyinl
  \and
  \tyrinl
\end{mathpar}


\framebox{$\einr e $ }
\begin{mathpar}
  \tyinr
  \and
  \tyrinr
\end{mathpar}

\framebox{$\ecase(e,x.e_1,y.e_2)$}
\begin{mathpar}
 \tycase
 \and
 \tyrcase
\end{mathpar}


\caption{ {\tname} typing rules (Part 1)}
\end{figure}



\begin{figure}


\framebox{$\efix f(x).e$}
\begin{mathpar}
  \tyfix
  \and
  \tyrfix
  \and
  \tyrfixNC
\end{mathpar}


\framebox{$e_1 \eapp e_2$}
\begin{mathpar}
  \tyapp
  \and
  \tyrappD
  % \and
  % \tyrappE
\end{mathpar}


\framebox{$\la e_1, e_2 \ra$}
\begin{mathpar}
  \typrod
  \and
  \tyrprod
\end{mathpar}

\framebox{$\eleft (e)$}
\begin{mathpar}
  \typroj
  \and
  \tyrproj
\end{mathpar}


\framebox{$\eright (e)$}\\

Symmetric rules. \\



\caption{{\tname} typing rules (Part 2)}
\end{figure}


\begin{figure}




\framebox{$\enil$}
\begin{mathpar}
  \tynil
  \and
  \tyrnil
\end{mathpar}


\framebox{$\econs(e_1,e_2)$}
\begin{mathpar}
  \tycons
  \and
  \tyrcons
  \and
  \tyrconsbox
\end{mathpar}

\framebox{$\ecase e \eof \enil \rightarrow e_1 ~|~ h::tl \rightarrow e_2$}
\begin{mathpar}
  \tycaseL
  \and
  \tyrcaseL
\end{mathpar}

\framebox{$\eleaf$}
\begin{mathpar}
  \tyleaf
  \and
  \tyrleaf
\end{mathpar}

\framebox{$\enode(e_l,e, e_r)$}
\begin{mathpar}
  \tynode
  \and
  \tyrnode
  \and
  \tyrnodeb
 \end{mathpar}

\caption{{\tname} typing rules (Part 3)}
\end{figure}




\begin{figure}
\framebox{$\ecase e \eof \eleaf \rightarrow e_1 ~|~ \enode(l,x,r) \rightarrow e_2$}
\begin{mathpar}
  \tycaseT
  \and
  \tyrcaseT
\end{mathpar}


\framebox{$\eLam e$}
\begin{mathpar}
  \tyiLam
  \and
  \tyriLam
\end{mathpar}


\framebox{$e \eApp$}
\begin{mathpar}
  \tyiApp
  \and
  \tyriApp
\end{mathpar}

\framebox{$\epack e$}
\begin{mathpar}
  \typack
  \and
  \tyrpack
\end{mathpar}


\framebox{$\eunpack e \eas x \ein e'$}
\begin{mathpar}
  \tyunpack
  \and
  \tyrunpackD
\end{mathpar}


\caption{Typing rules (Part 4)}
\end{figure}





\begin{figure}

\framebox{Primitive application}
\begin{mathpar}
  \typrimapp
  \and
  \tyrprimapp
\end{mathpar}



\framebox{$\tcprod{C}{\tau}$ intro. rules}
\begin{mathpar}
  \tycandIntro
  \and
  \tyrcandIntro
\end{mathpar}

\framebox{$\tcprod{C}{\tau}$ elim. rules}
\begin{mathpar}
  \tycandElim
  \and
  \tyrcandElimD
\end{mathpar}

\framebox{$\tcimpl{C}{\tau}$ intro. rules}
\begin{mathpar}
  \tycimplIntro
  \and
  \tyrcimplIntro
\end{mathpar}


\framebox{$\tcimpl{C}{\tau}$ elim. rules}
\begin{mathpar}
  \tycimplElim
  \and
  \tyrcimplElimD
\end{mathpar}

% \framebox{Intersection intro. rules}
% \begin{mathpar}
%   \tyinterI
%   \and
%   \tyrinterI
% \end{mathpar}

% \framebox{Intersection elim. rules}
% \begin{mathpar}
%   \tyinterE
%   \and
%   \tyrinterE
% \end{mathpar}


\framebox{$\elet x = e_1 \ein e_2$}
\begin{mathpar}
  \tylet
  \and
  \tyrlet
\end{mathpar}


\end{figure}


 
\begin{figure}



\framebox{Subtyping}
\begin{mathpar}
  \tysubsum
  \and
  \tyrsubsum
\end{mathpar}



\framebox{Constraint dependent typing}
\begin{mathpar}
  \tysplit
  \and
  \tyrsplit
  \and
  \tycontra
  \and
  \tyrcontra
\end{mathpar}


\framebox{Heuristic typing}
\begin{mathpar}
  \tyrletMax
  \and
  \tyrletcsym
  \and
  \tyappfun
  \and
  \tyappfunsym
  \and
  % \tyefix
  % \and
  \tycasee
  \and 
  \tyecase
  % \and
  % \tyepair
\end{mathpar}

\caption{{\tname} typing rules (Part 6)}
\end{figure}



%%% Local Variables:
%%% mode: latex
%%% TeX-master: "main"
%%% End:
